# Supplementary material for: High-dimensional Black-box Optimization Under Uncertainty
Source: arXiv:1911.02457 source file (2021-09-09)
Supplement: Supplementary file 1 [file Appendix-archive.tex]

\section{Additional Experimental Results}\label{app:results}

This section provides experimental results in addition to those in Section \ref{sec:results}. Figure~\ref{fig:auc_box_rast} presents the box-plots of the MTFAUC for 30 executions using different approaches on the Rastrigin test function when we use TK-MARS in a surrogate optimization algorithm. We can observe that $\mathit{Fixedrep},10$  has the smallest interquartile range and is the most robust approach to uncertainty, however, it has a higher average MTFAUC across different noise levels compared with that of $\mathit{Smartrep},10$.
The reason is likely due to the highly fluctuating behavior of the Rastrigin function with several local optima combined with the noise added to the function, which makes an optimum hard to obtain.

Figure~\ref{fig:bks_box_rast} shows the box-plots of the true objective value of BSMS after 1000 black-box function evaluations for the same 30 executions on the Rastrigin test function. We observe the same pattern for the quality of the final BSMS after 1000 evaluations. $\mathit{Smartrep},10$ finds a slightly better BSMS across the noise levels with relative robustness. 

Figure~\ref{fig:auc_box_levy} displays the box-plots of the MTFAUC  for 30 executions using different approaches on the Levy test function. We note that the interquartile range for $\mathit{Smartrep},10$ is comparatively small at higher levels of noise. 

Figure~\ref{fig:bks_box_levy} shows the box-plots of the true objective value of BSMS after 1000 black-box function evaluations for the same 30 executions on the Levy test function.
Although $\mathit{Norepl}$ is the most robust approach to the different noise levels, the performance of the $\mathit{Smartrep},10$ is also competitive.  

Figure~\ref{fig:rbf_auc_box_rast} presents the box-plots of the MTFAUC for 30 executions using different approaches on the Rastrigin test function when we use RBF in a surrogate optimization algorithm. We observe that $\mathit{Fixedrep},10$ has the highest robustness to uncertainty, however, it has a larger true objective value of the BSMS, comparatively, as shown in Figure~\ref{fig:rbf_bks_box_rast}. 

Figure~\ref{fig:rbf_bks_box_rast} shows the box-plots of the true objective value of BSMS after 1000 black-box function evaluations for the same 30 executions.
On average, $\mathit{Norepl}$ finds better BSMS when the uncertainty level is low, and $\mathit{Smartrep},10$ finds better BSMS at the highest noise level.
Consequently, this suggests that for a highly fluctuating function like Rastrigin, we need more exploration as well as more replication.

Figure~\ref{fig:rbf_auc_box_levy} presents the box-plots of the MTFAUC for 30 executions using different approaches on the Levy test function when we use RBF in a surrogate optimization algorithm. We note that $\mathit{Smartrep},5$ is the most robust approach across different noise levels.
$\mathit{Smartrep},10$ is competitive as well. Although the performance of $\mathit{Fixedrep},5$ is noticeable at the higher noise levels, it conducts unnecessary black-box function evaluations in a deterministic environment.

Figure~\ref{fig:rbf_bks_box_levy} shows the box-plots of the true objective value of the BSMS after 1000 black-box function evaluations for the same 30 executions on the Levy test function.
We verified that $\mathit{Smartrep},5$ has the smallest interquartile range overall, except when executed in a deterministic environment in which $\mathit{Norepl}$ has the lowest MTFAUC. In terms of robustness to uncertainty, $\mathit{Smartrep},5$ outperforms other approaches. It has a smaller interquartile range in a higher level of noise compared with $\mathit{Norepl}$ and at the lower levels of noise compared with $\mathit{Fixedrep},5$ and $\mathit{Fixedrep},10$.  

\begin{figure}[!htp]
\centering
    \begin{minipage}{\linewidth}
        \subfloat[]{\includegraphics[width=0.35\textwidth]{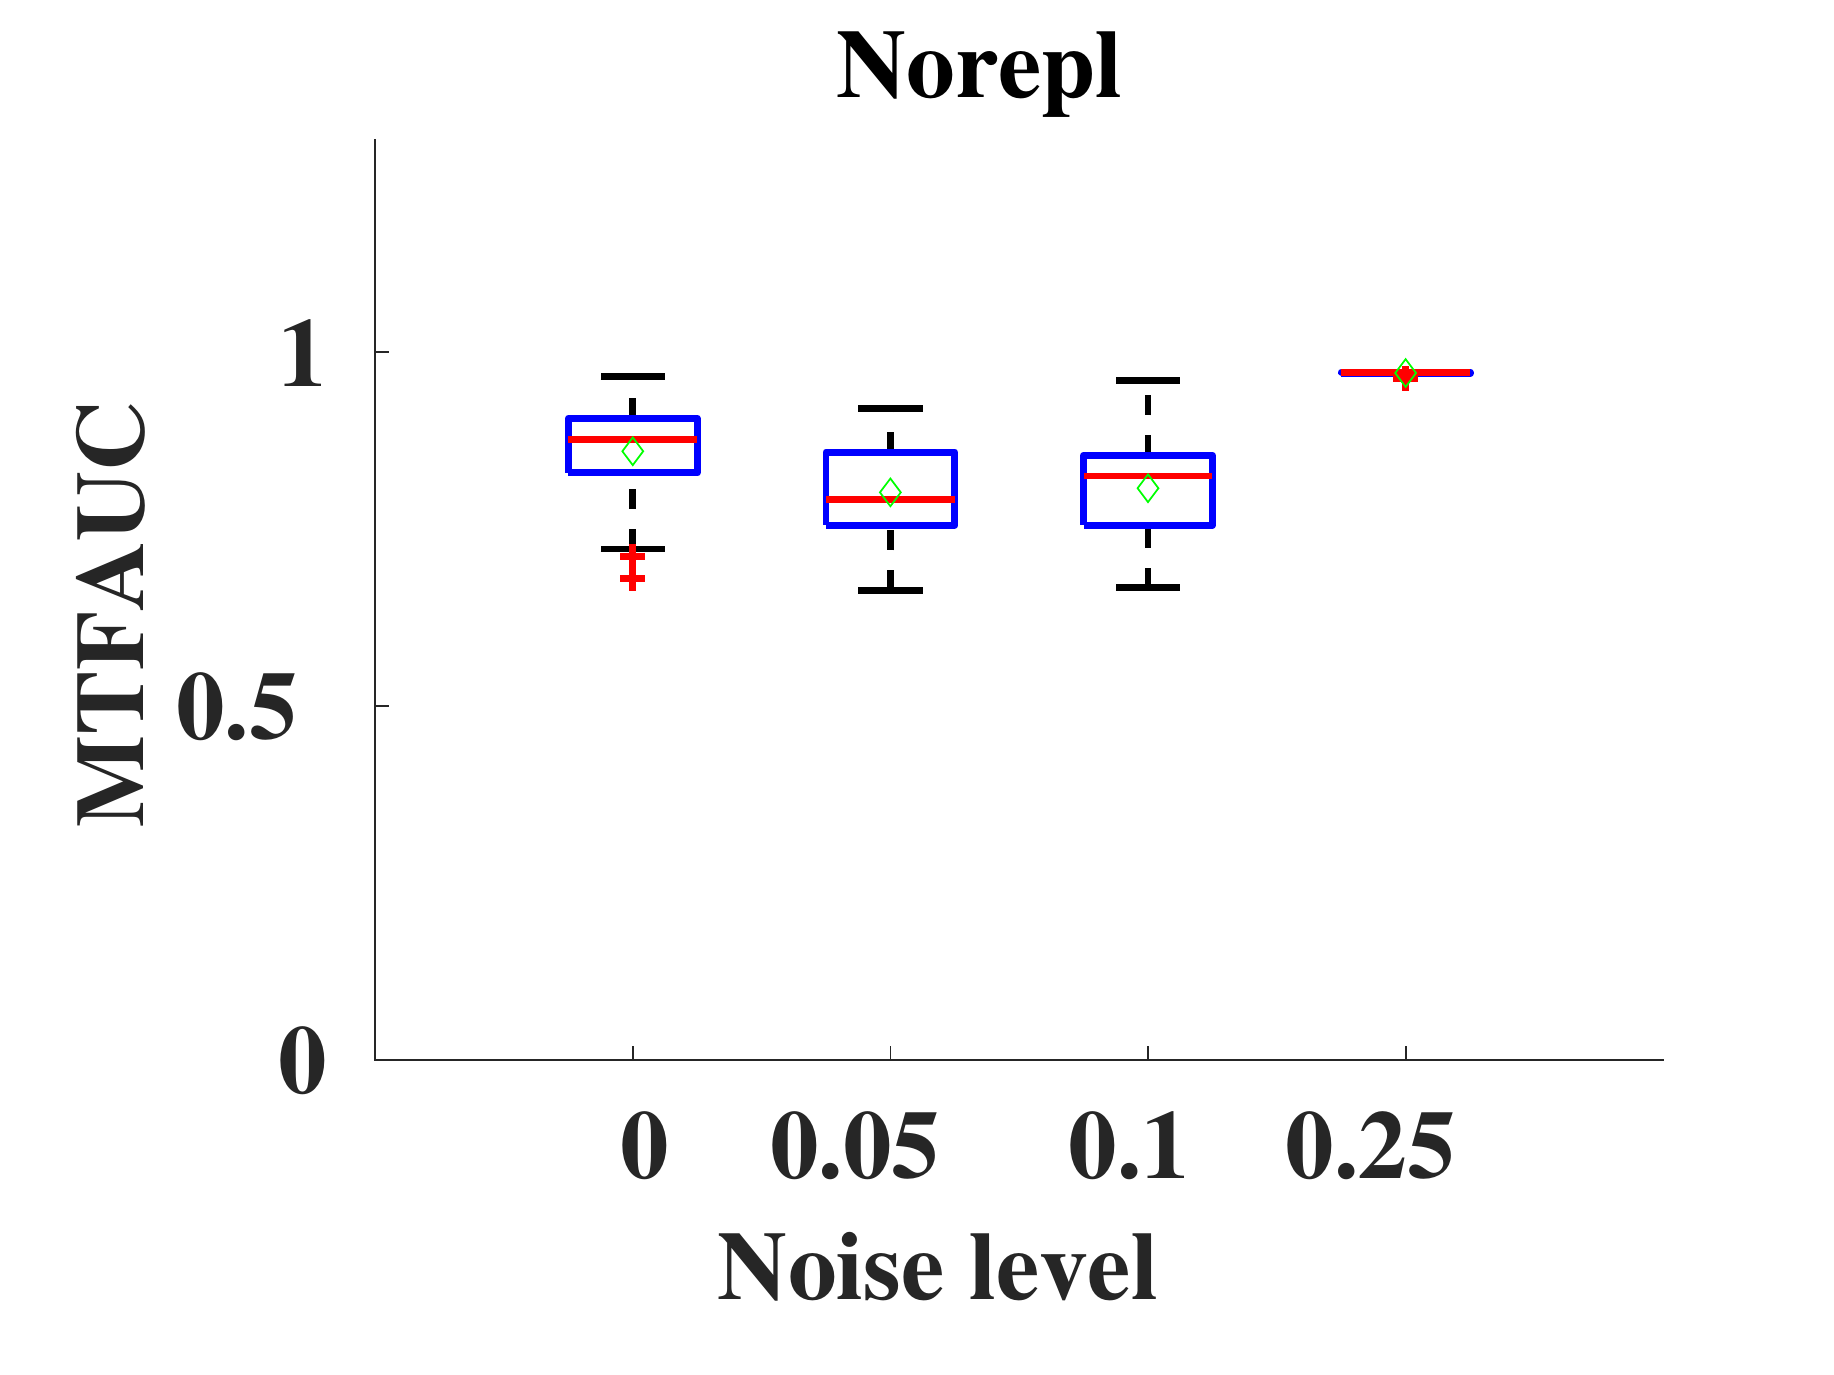}}
        \subfloat[]{\includegraphics[width=0.35\textwidth]{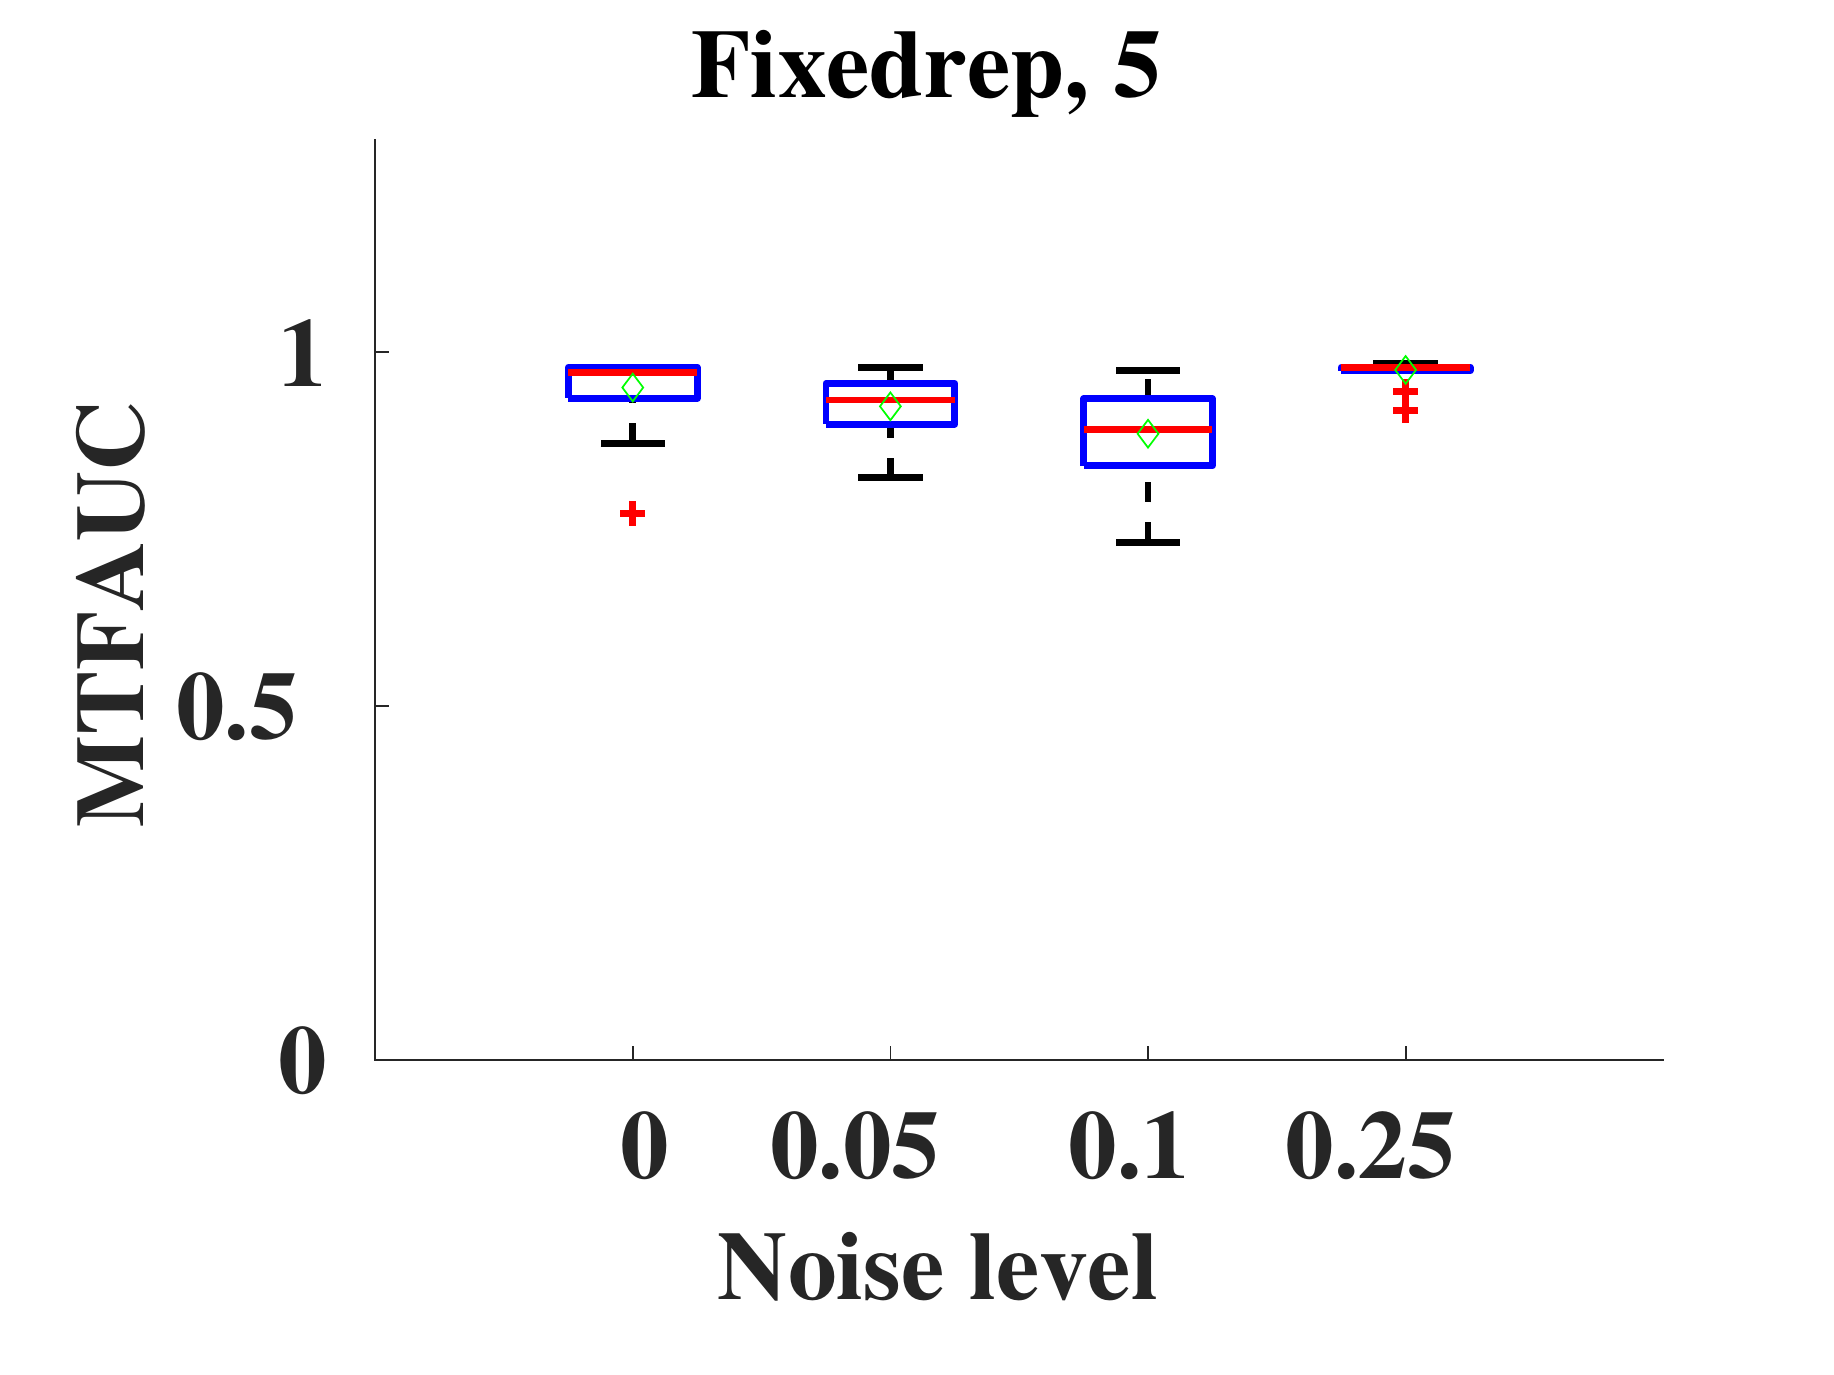}}
        \subfloat[]{\includegraphics[width=0.35\textwidth]{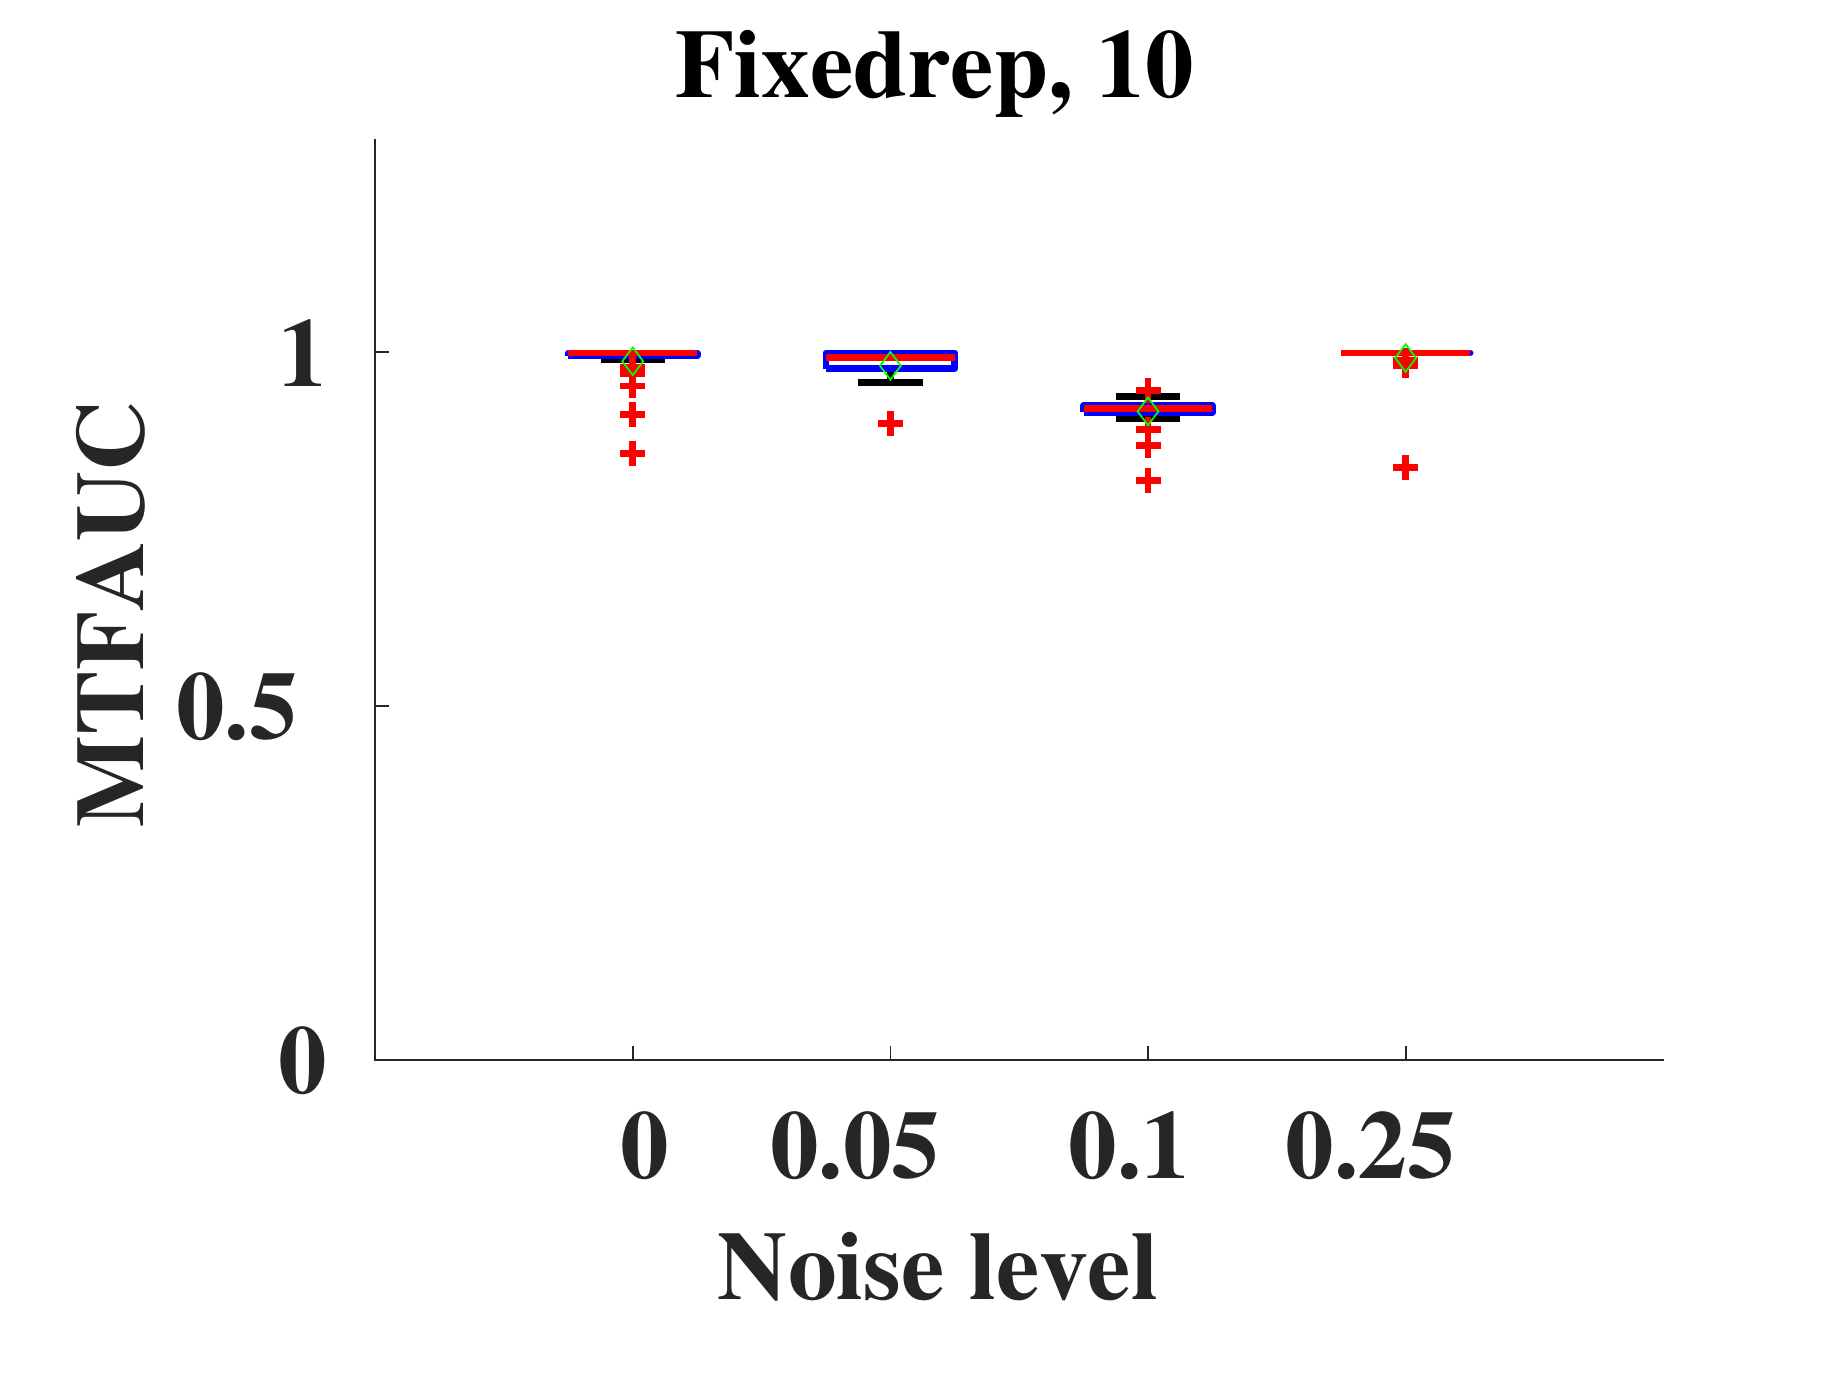}}
    \end{minipage}

    \begin{minipage}{\linewidth}
        \subfloat[]{\includegraphics[width=0.35\textwidth]{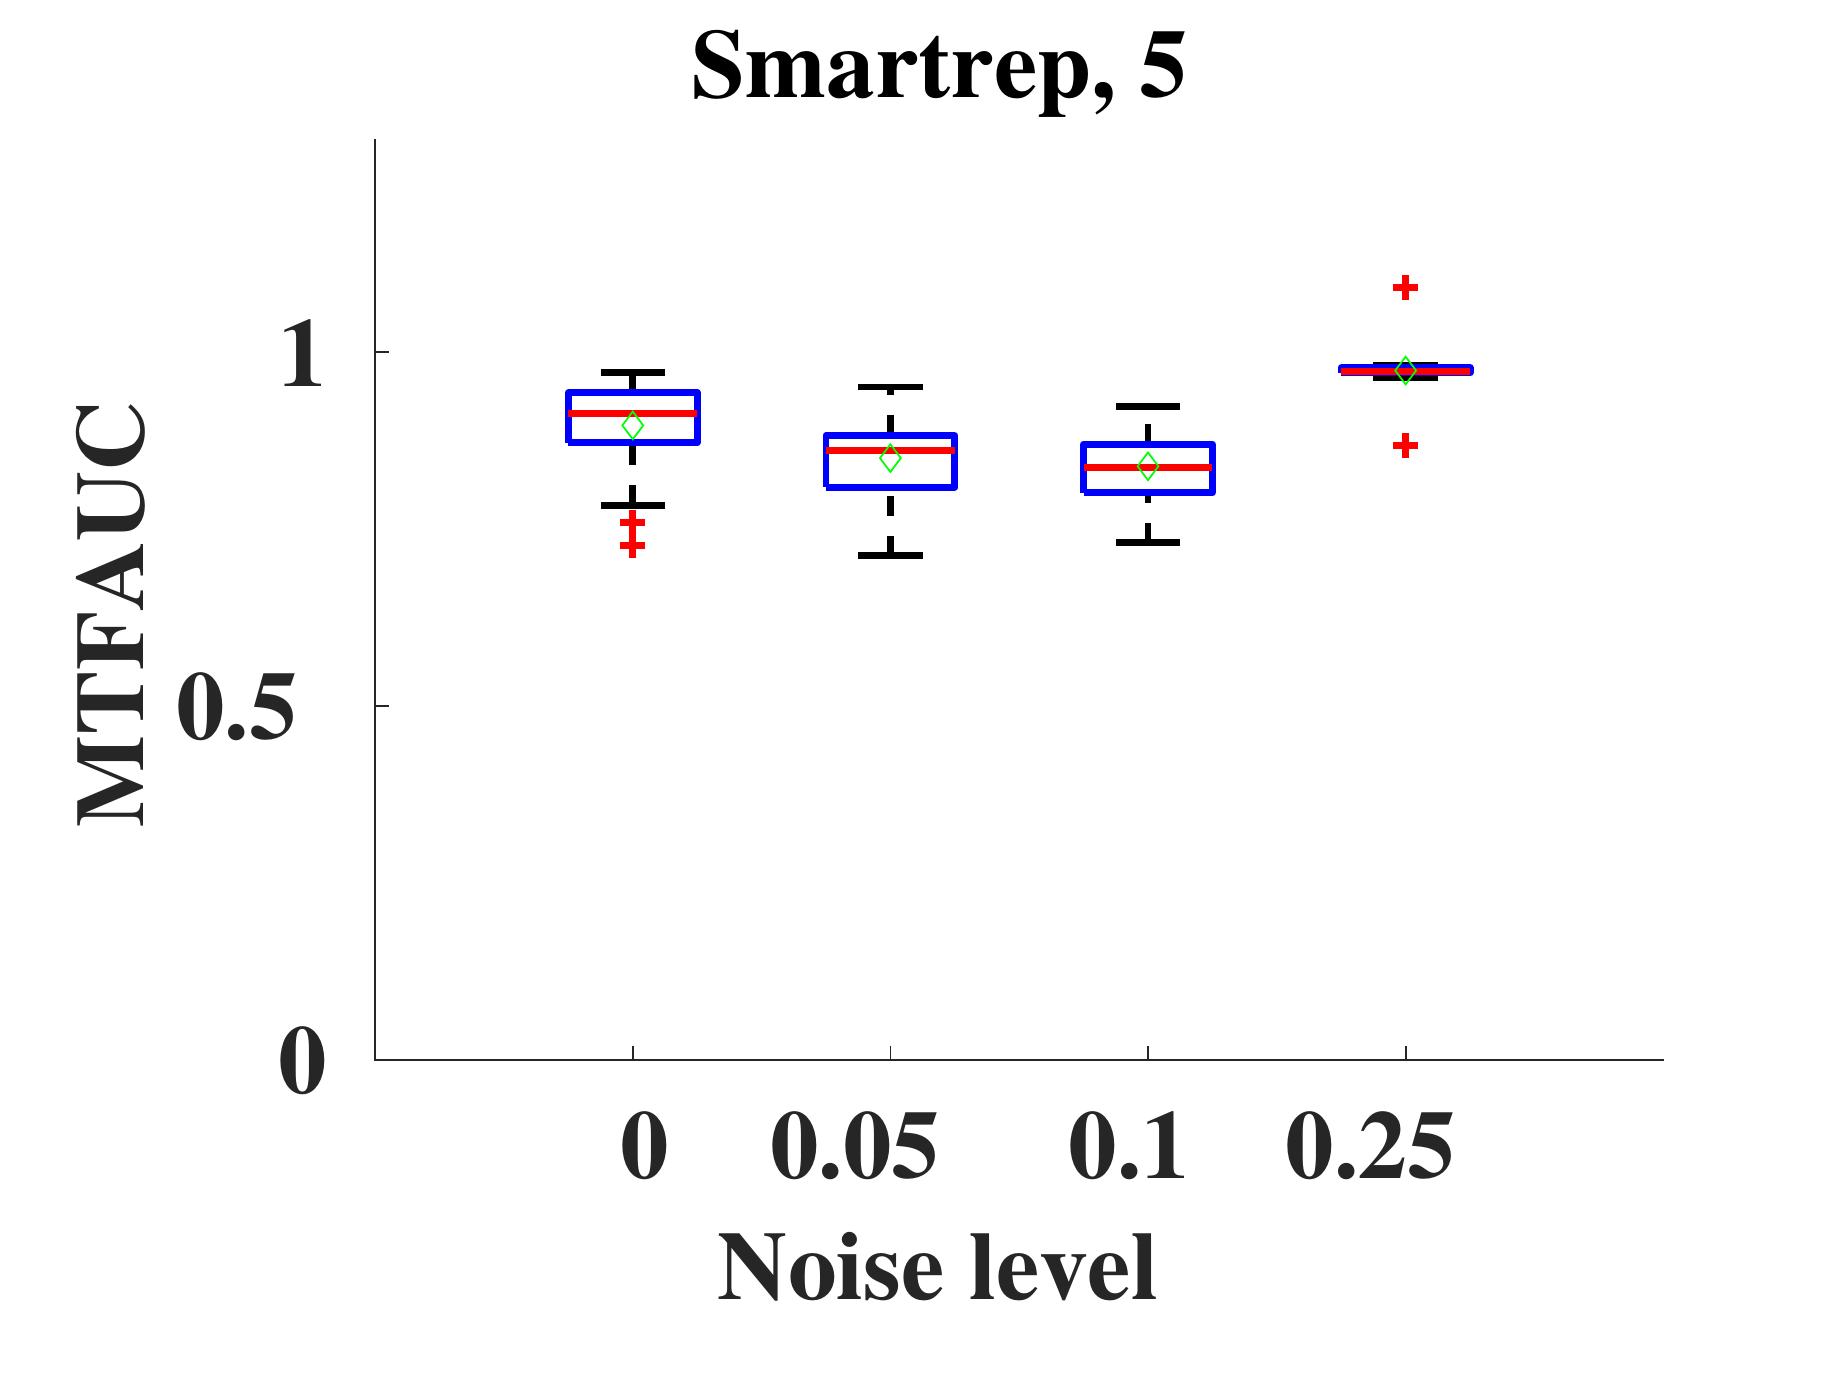}}
        \subfloat[]{\includegraphics[width=0.35\textwidth]{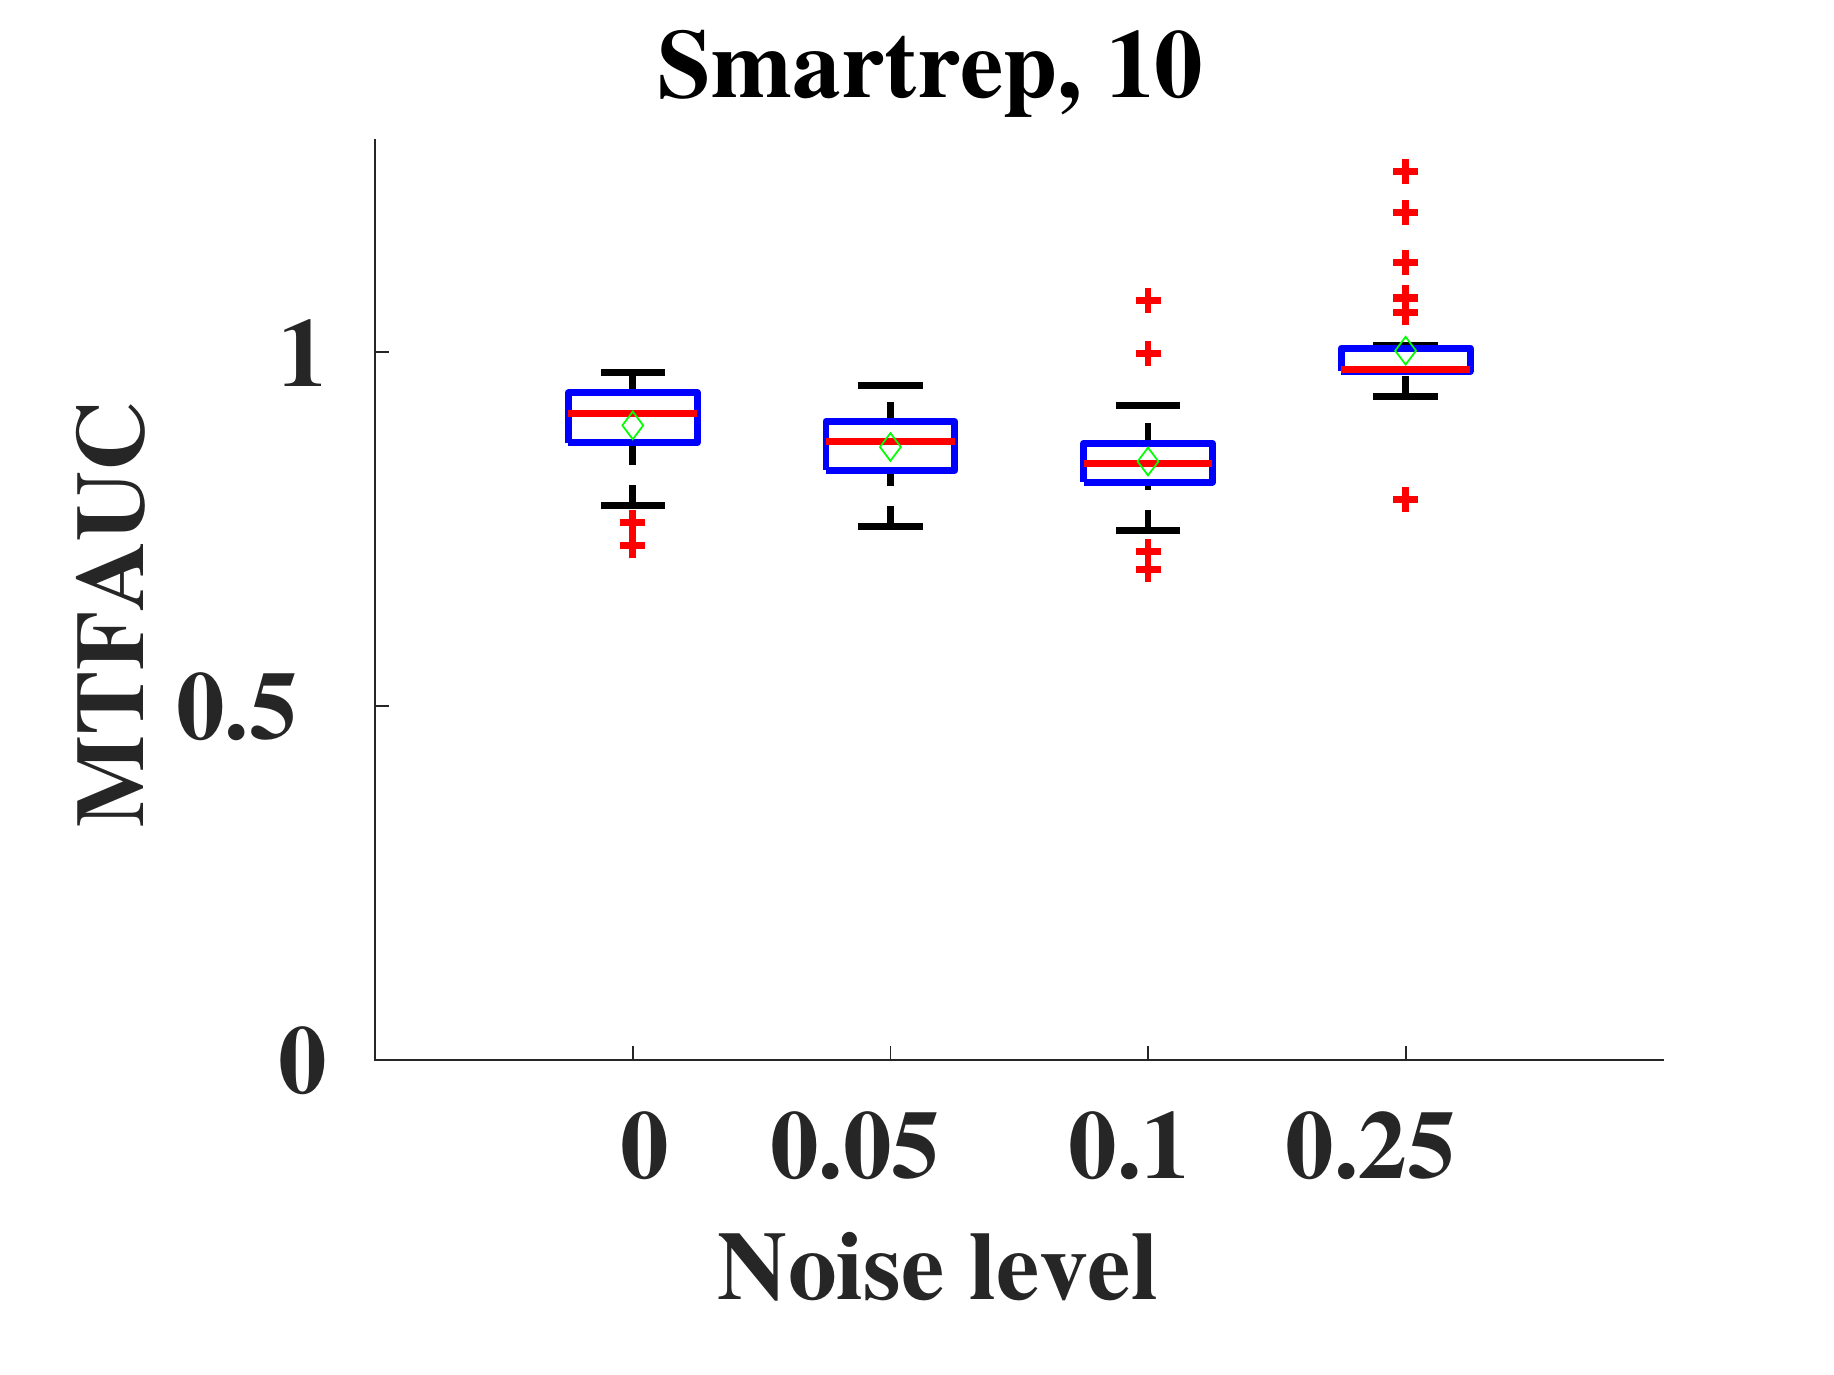}}
    \end{minipage}
    \caption{Box-plots of MTFAUC of surrogate optimization using TK-MARS on the Rastrigin function}
    \label{fig:auc_box_rast}
    \vspace{-5mm}
\end{figure}

\begin{figure}[!htp]
\centering
    \begin{minipage}{\linewidth}
        \subfloat[]{\includegraphics[width=0.35\textwidth]{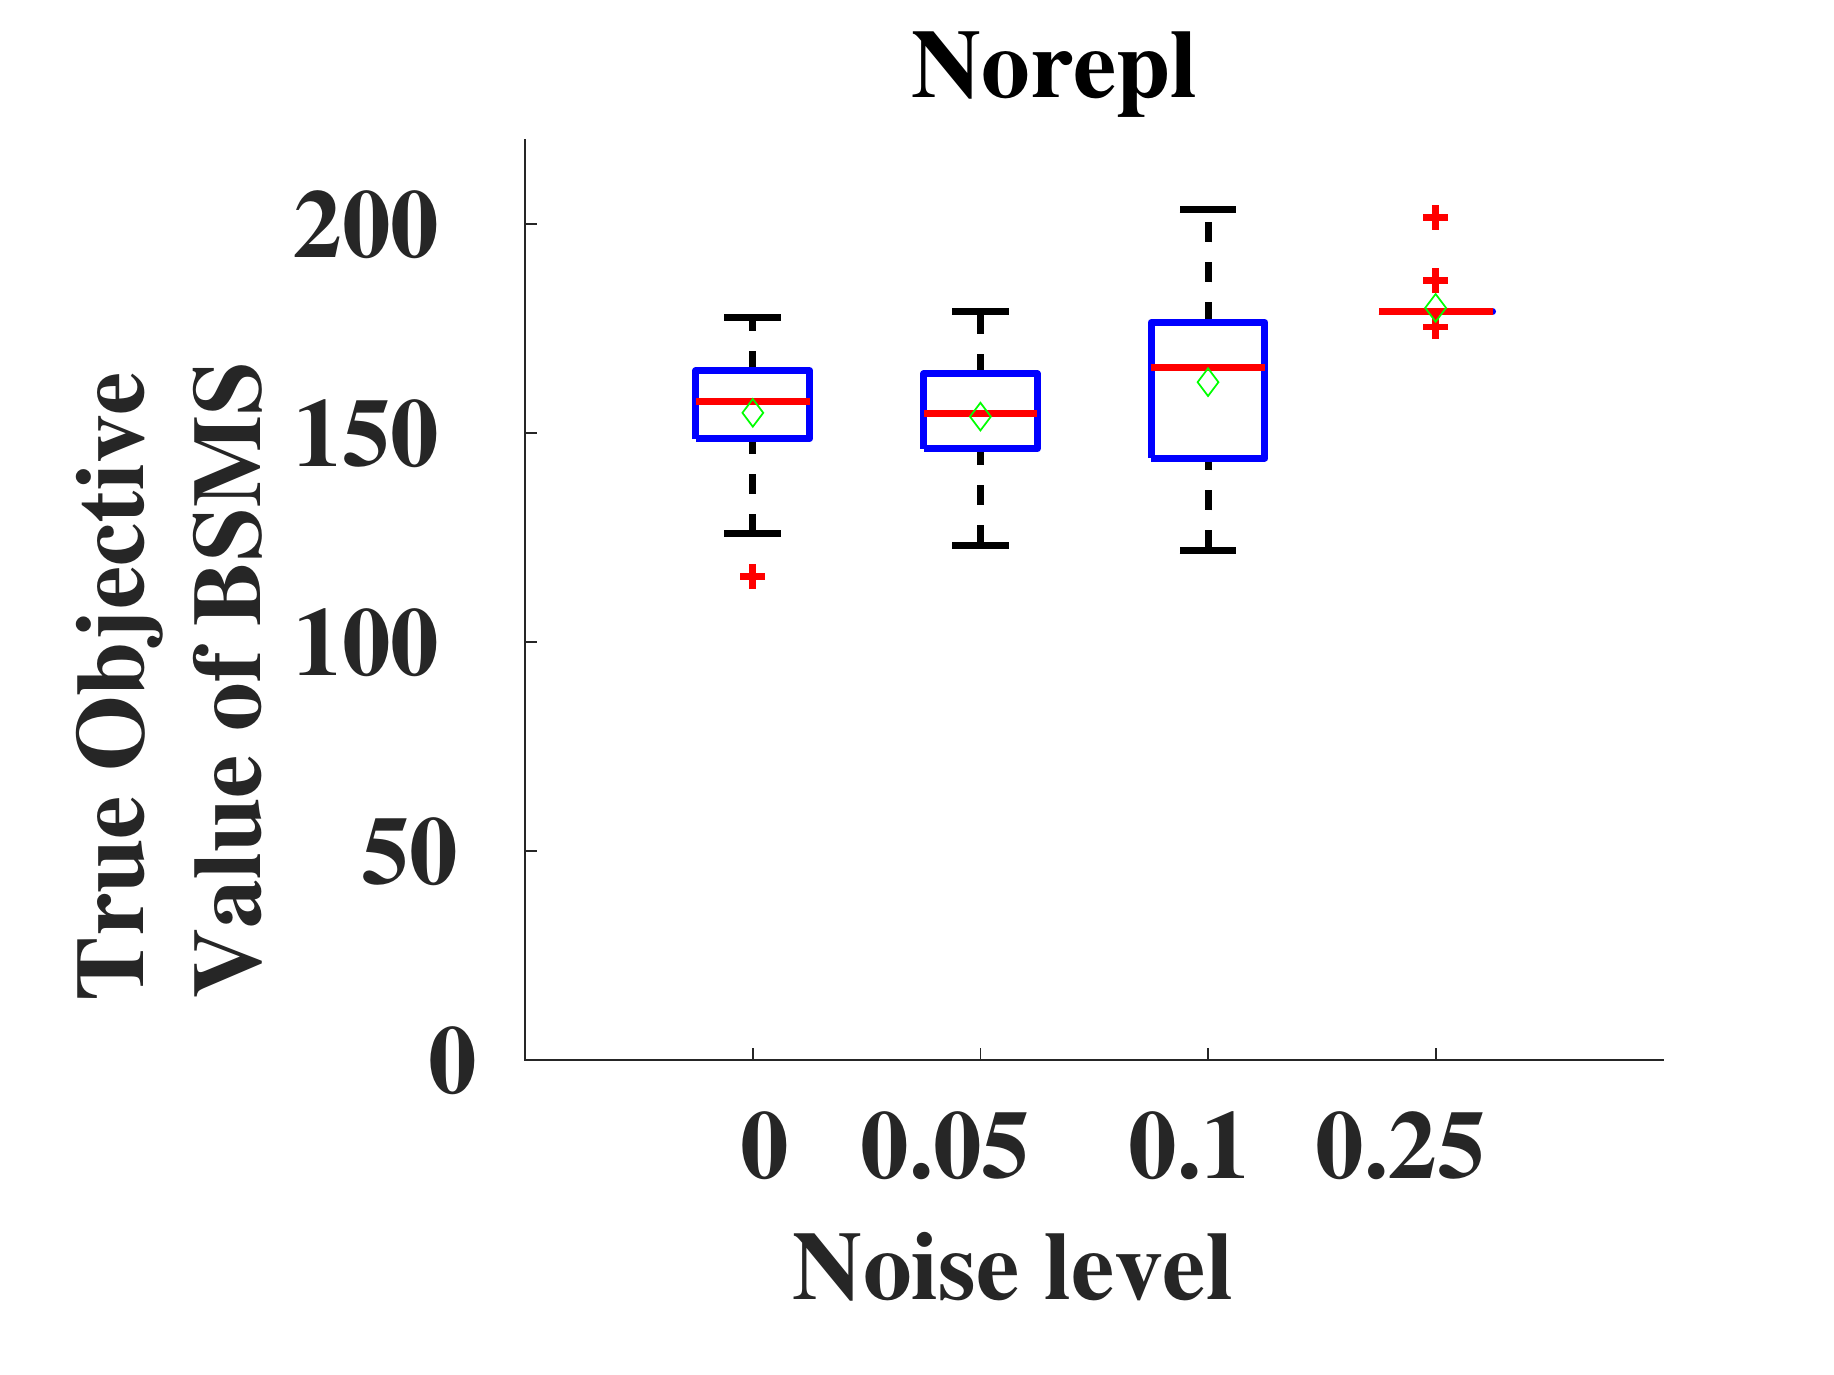}}
        \subfloat[]{\includegraphics[width=0.35\textwidth]{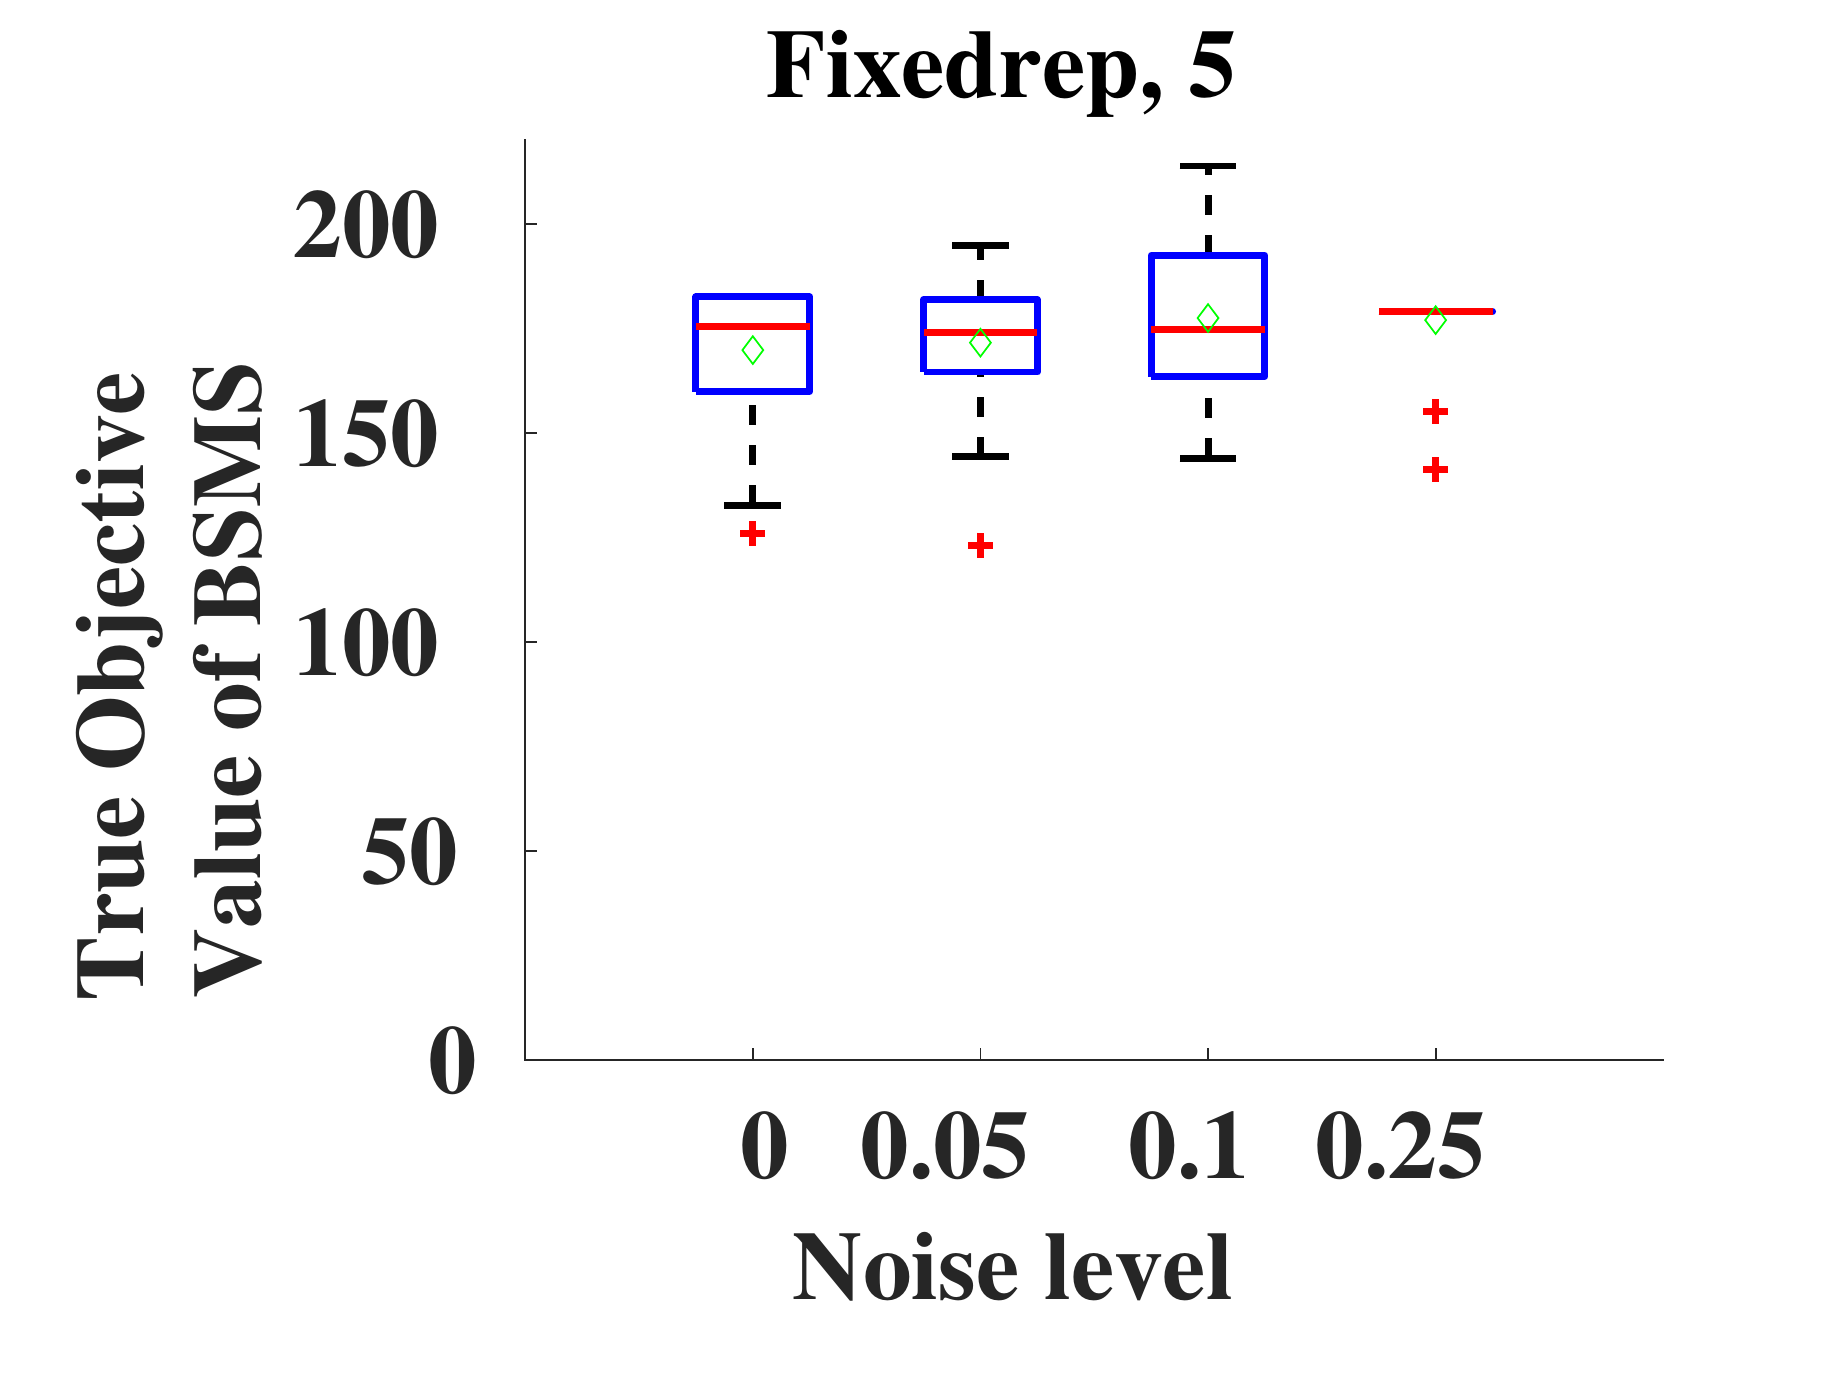}}
        \subfloat[]{\includegraphics[width=0.35\textwidth]{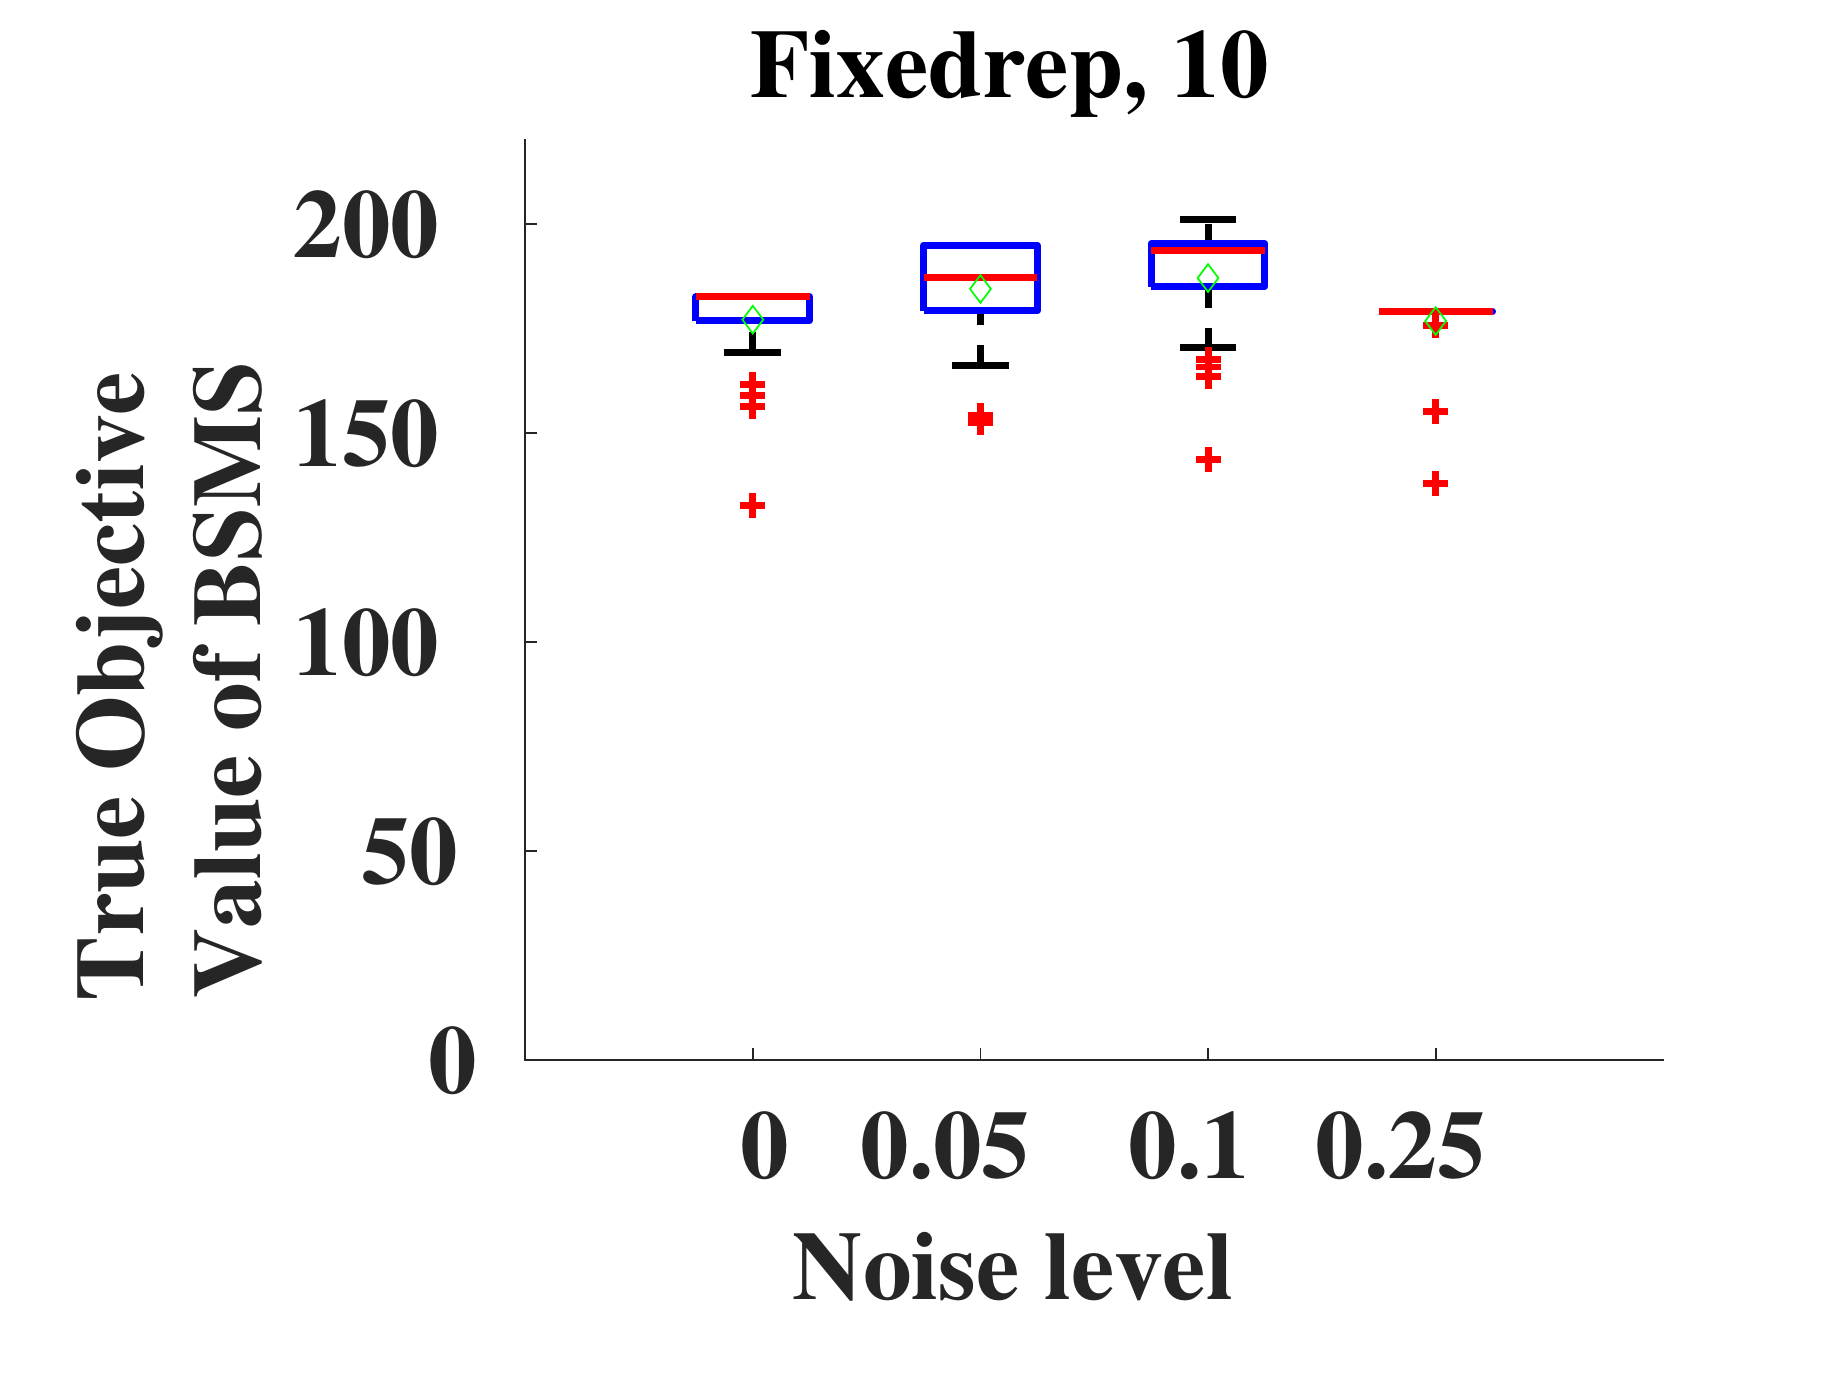}}
    \end{minipage}

    \begin{minipage}{\linewidth}
        \subfloat[]{\includegraphics[width=0.35\textwidth]{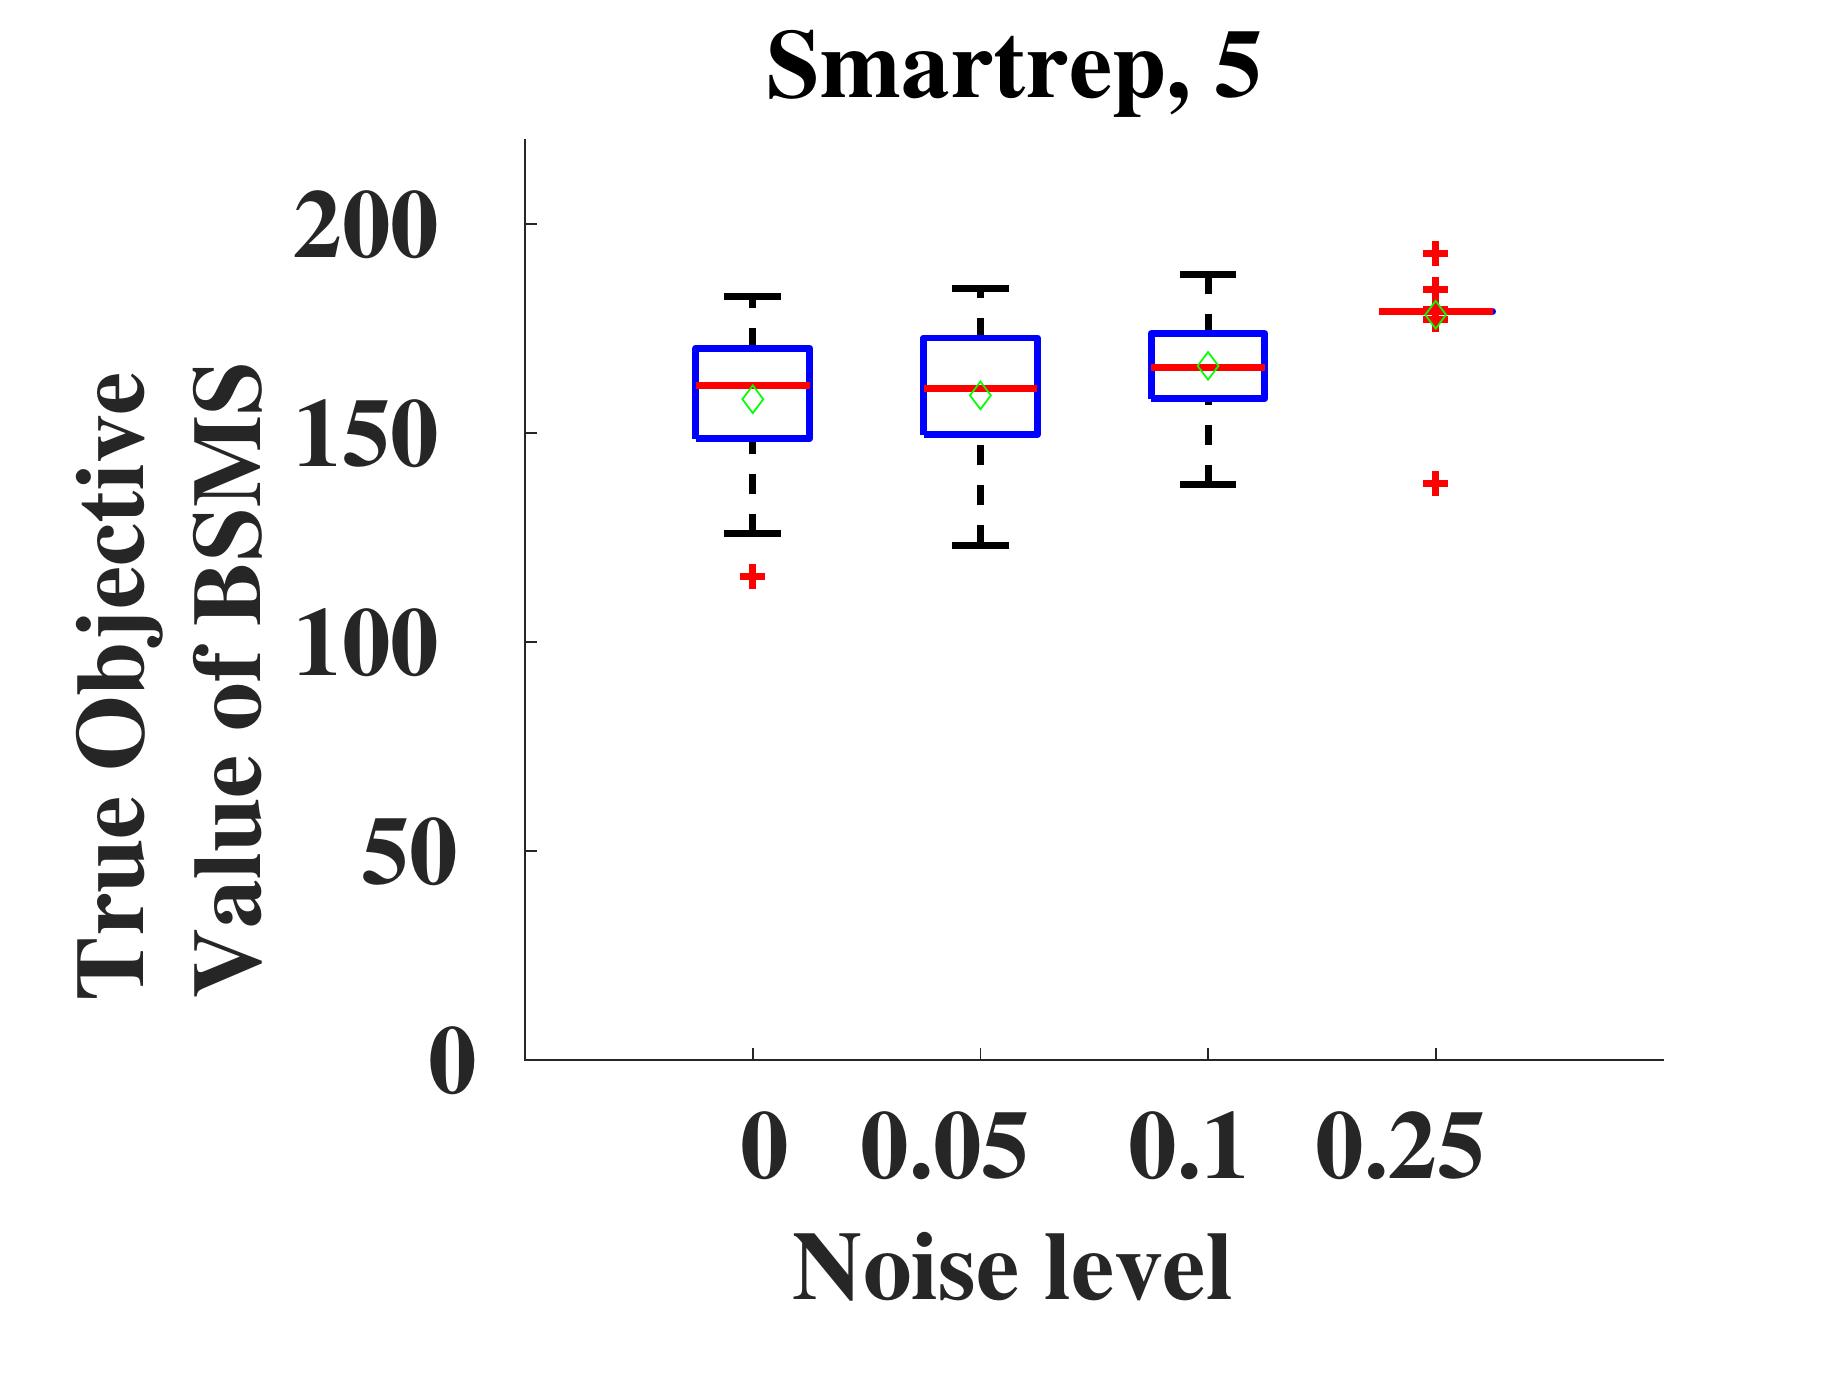}}
        \subfloat[]{\includegraphics[width=0.35\textwidth]{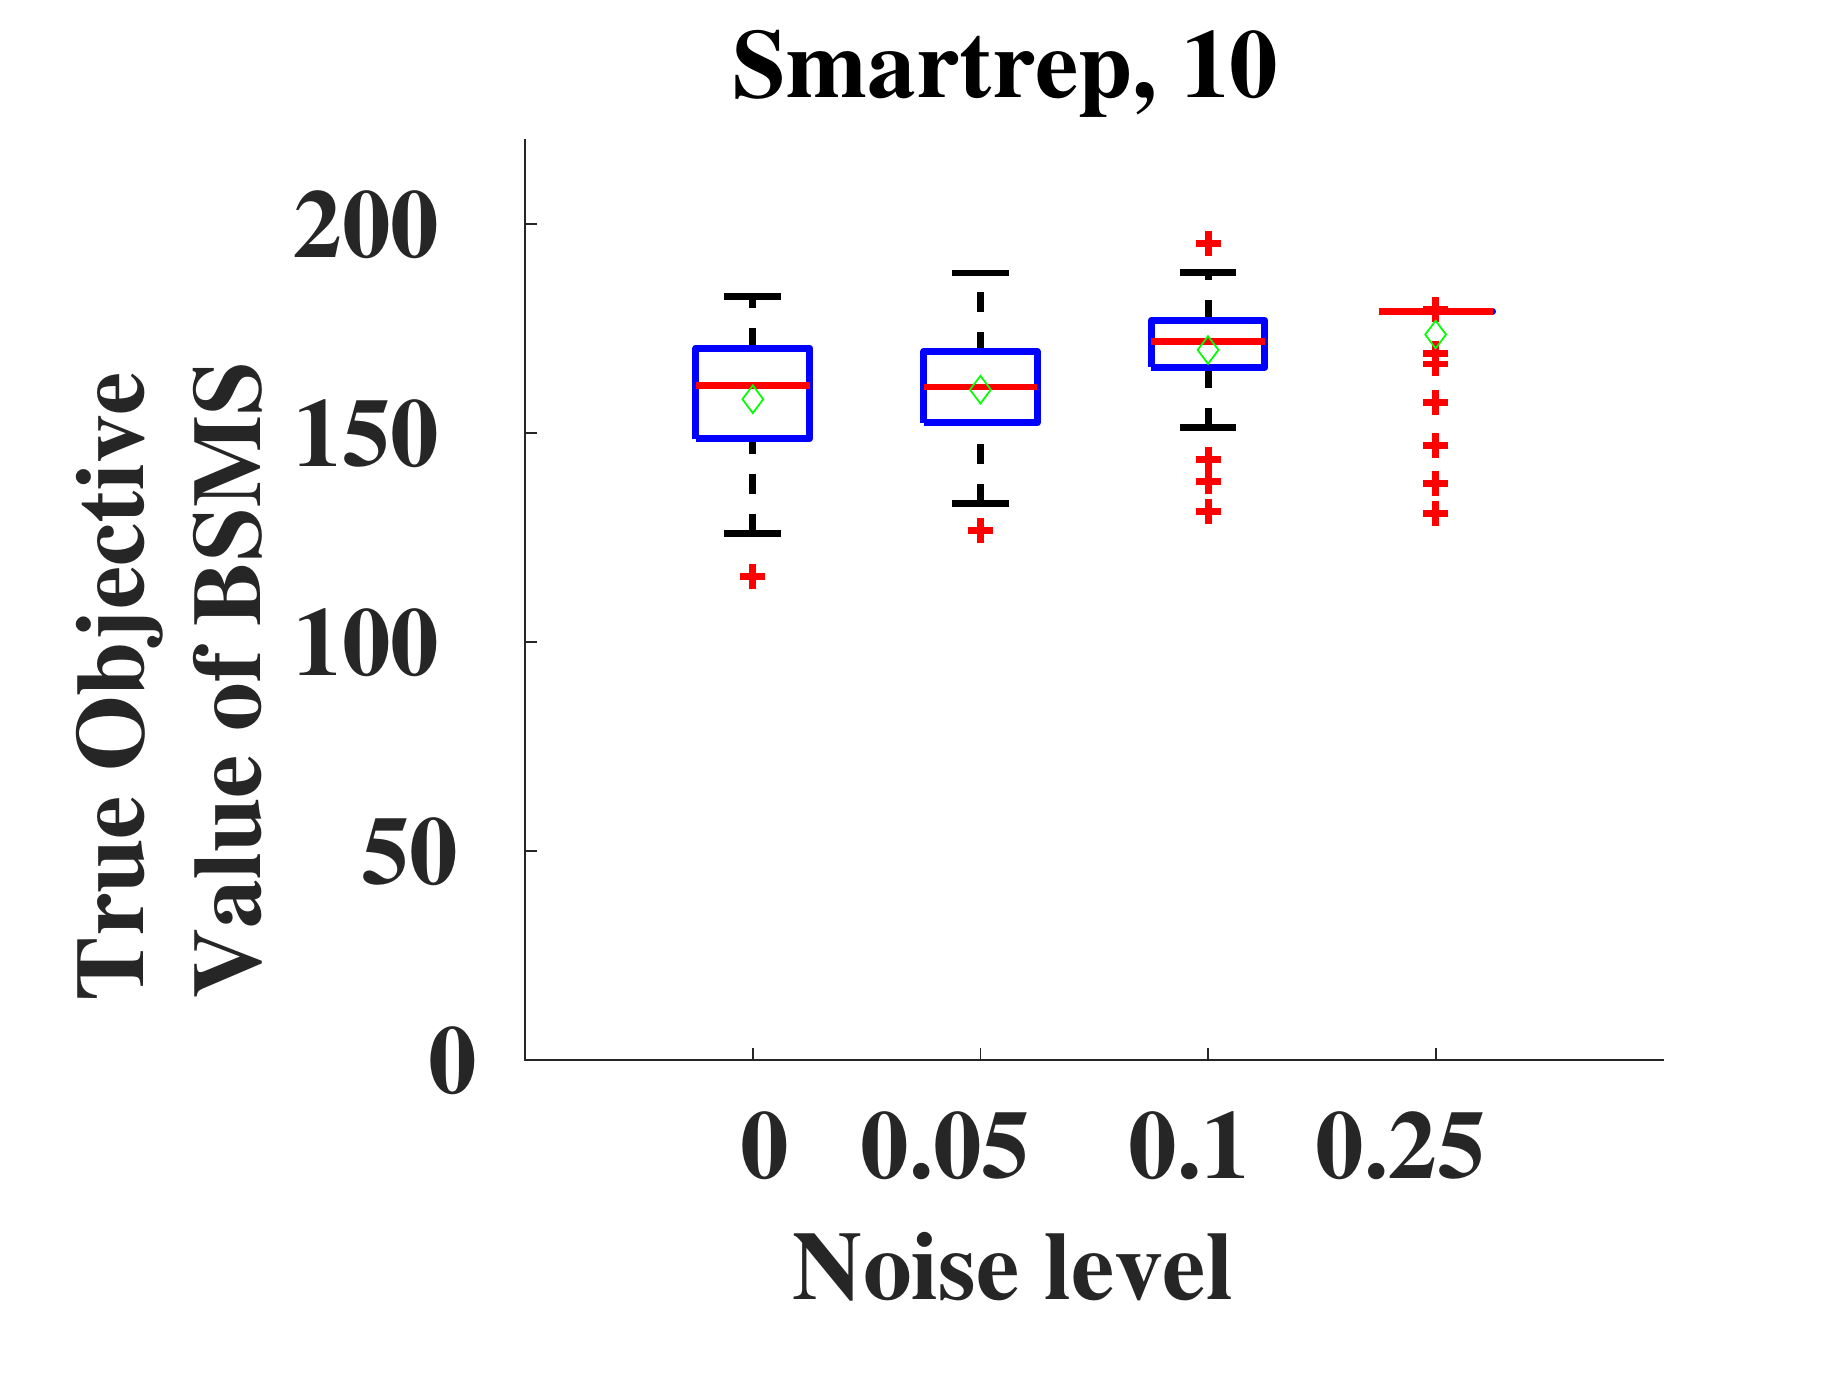}}
    \end{minipage}
    \caption{Box-plots of the true objective value of the BSMS after 1000 black-box function evaluations of surrogate optimization using TK-MARS on the Rastrigin function}
    \label{fig:bks_box_rast}
    \vspace{-5mm}
\end{figure}

\begin{figure}[!htp]
\centering
    \begin{minipage}{\linewidth}
        \subfloat[]{\includegraphics[width=0.35\textwidth]{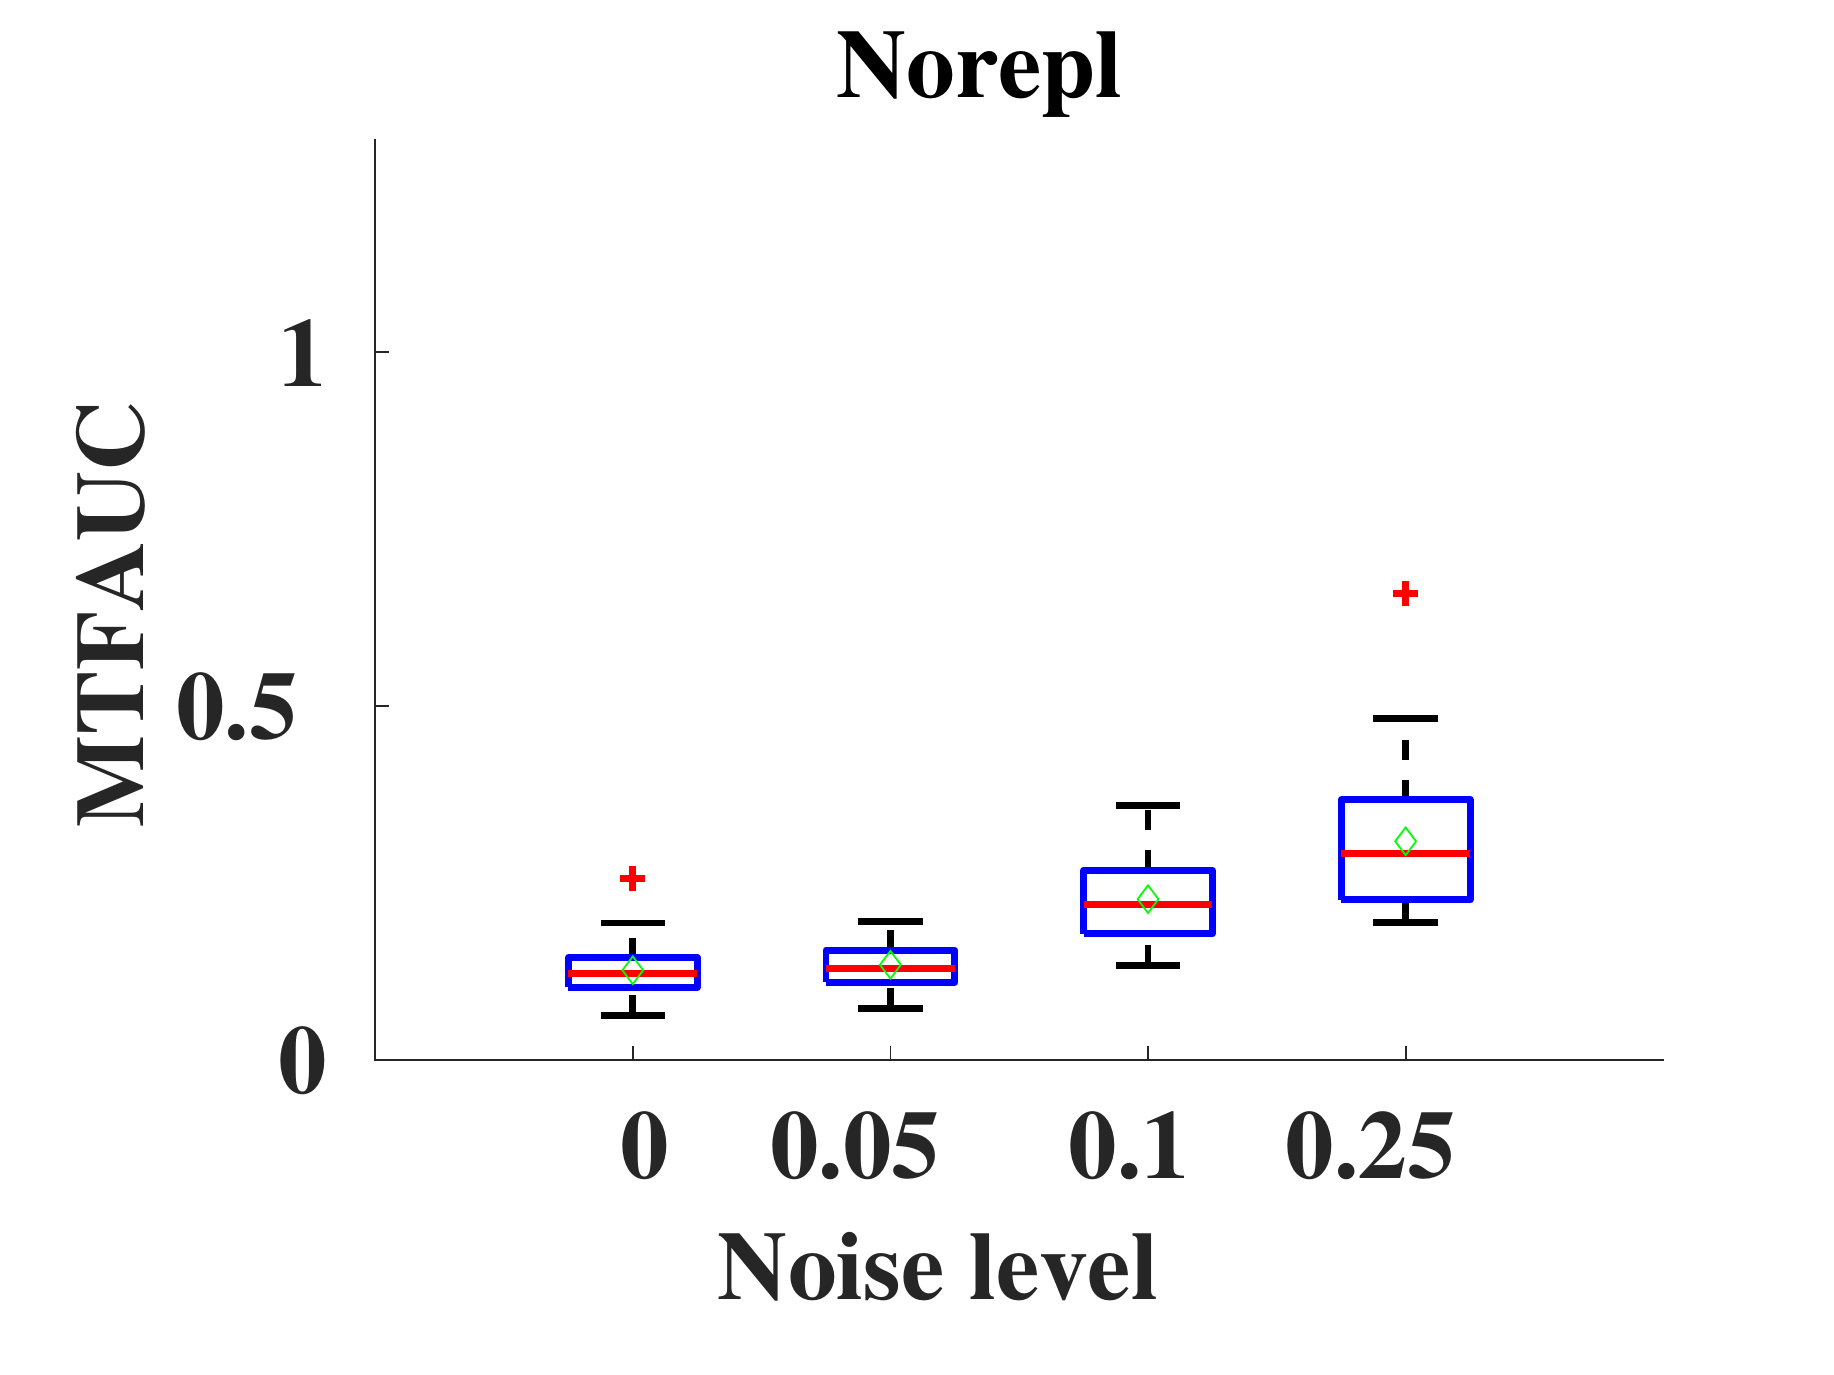}}
        \subfloat[]{\includegraphics[width=0.35\textwidth]{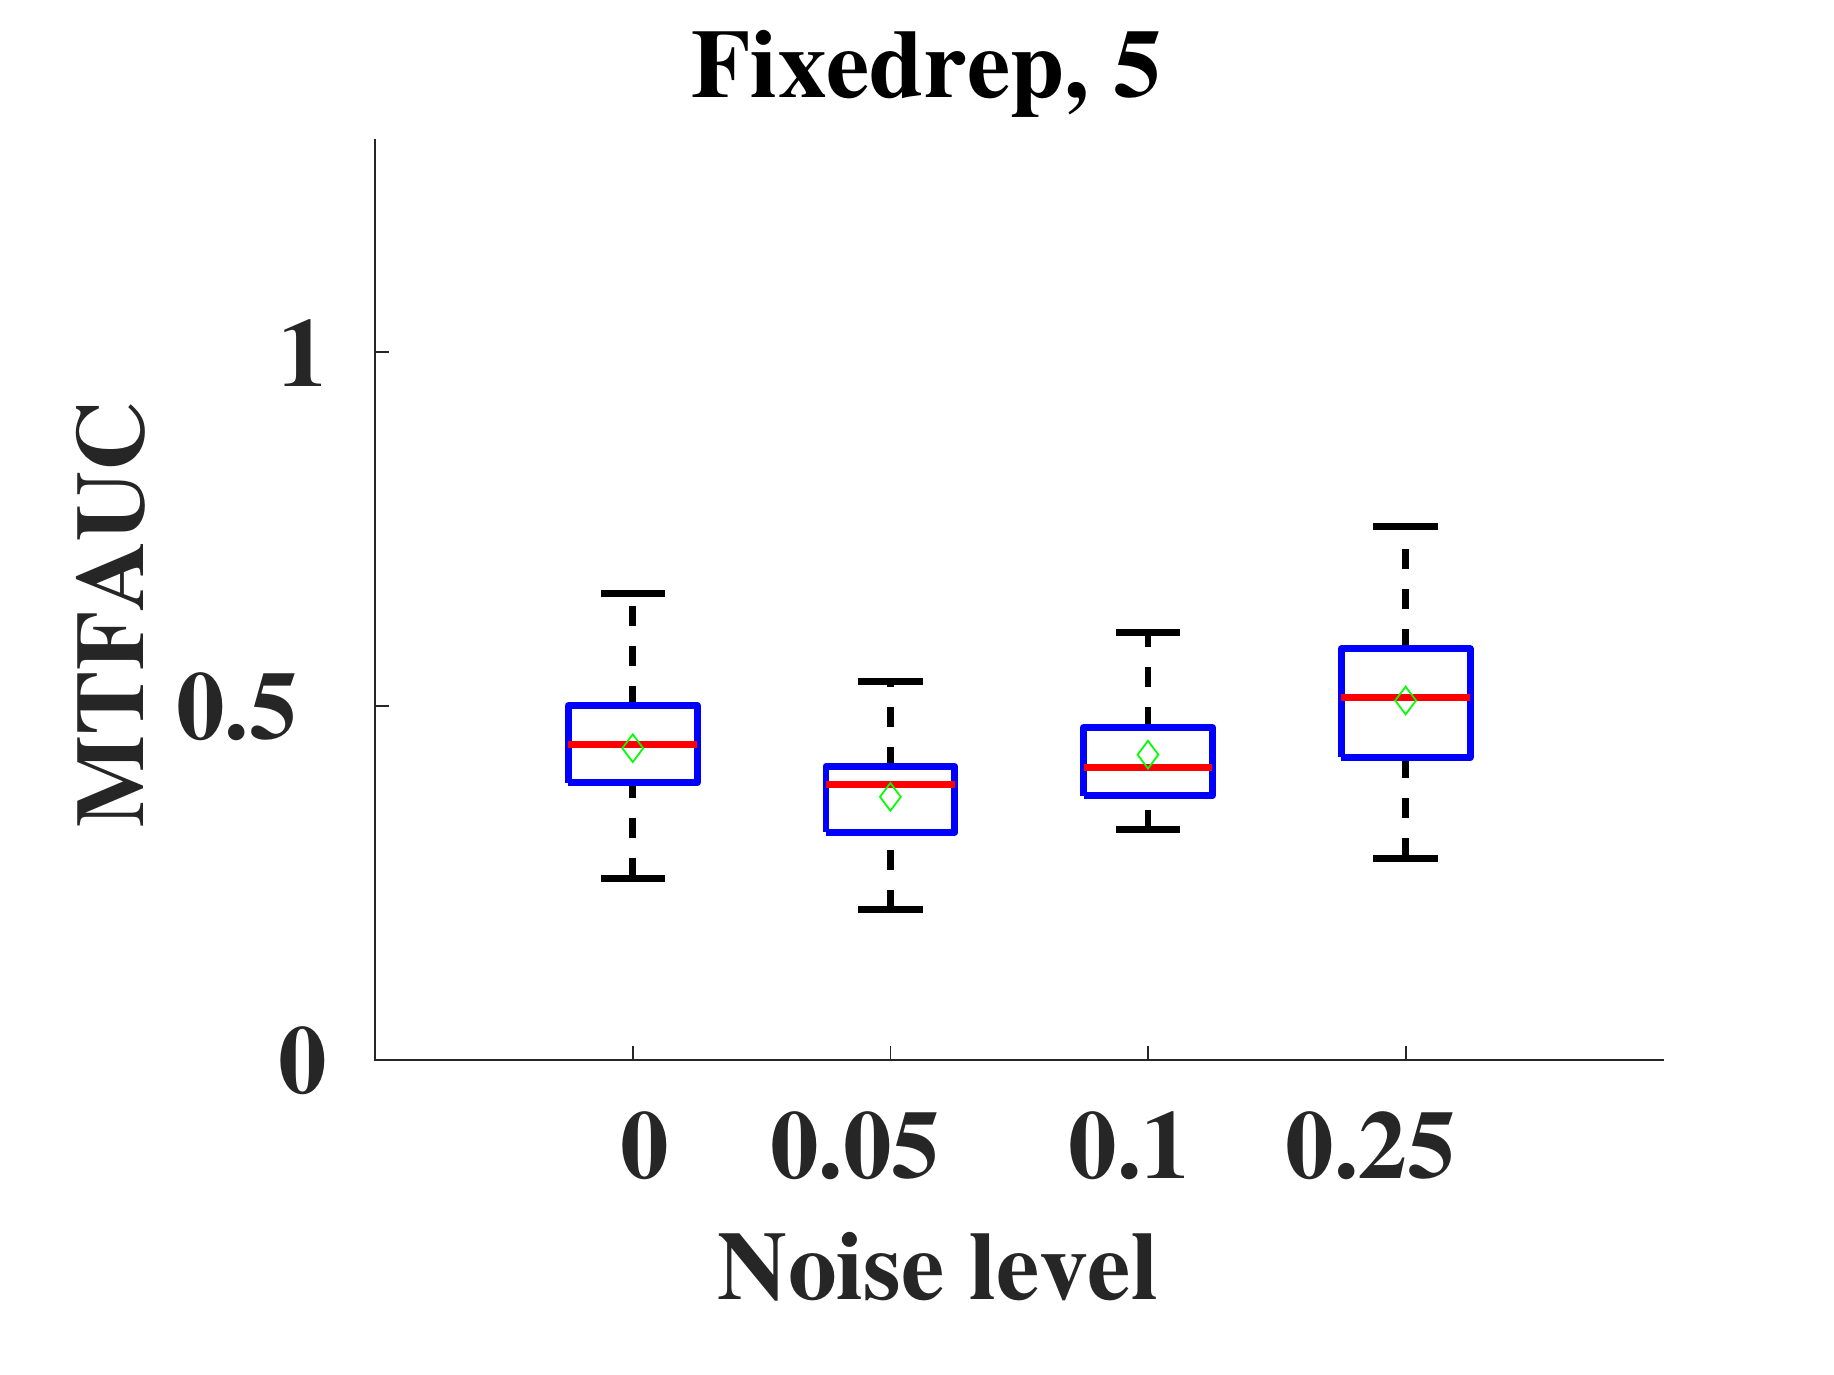}}
        \subfloat[]{\includegraphics[width=0.35\textwidth]{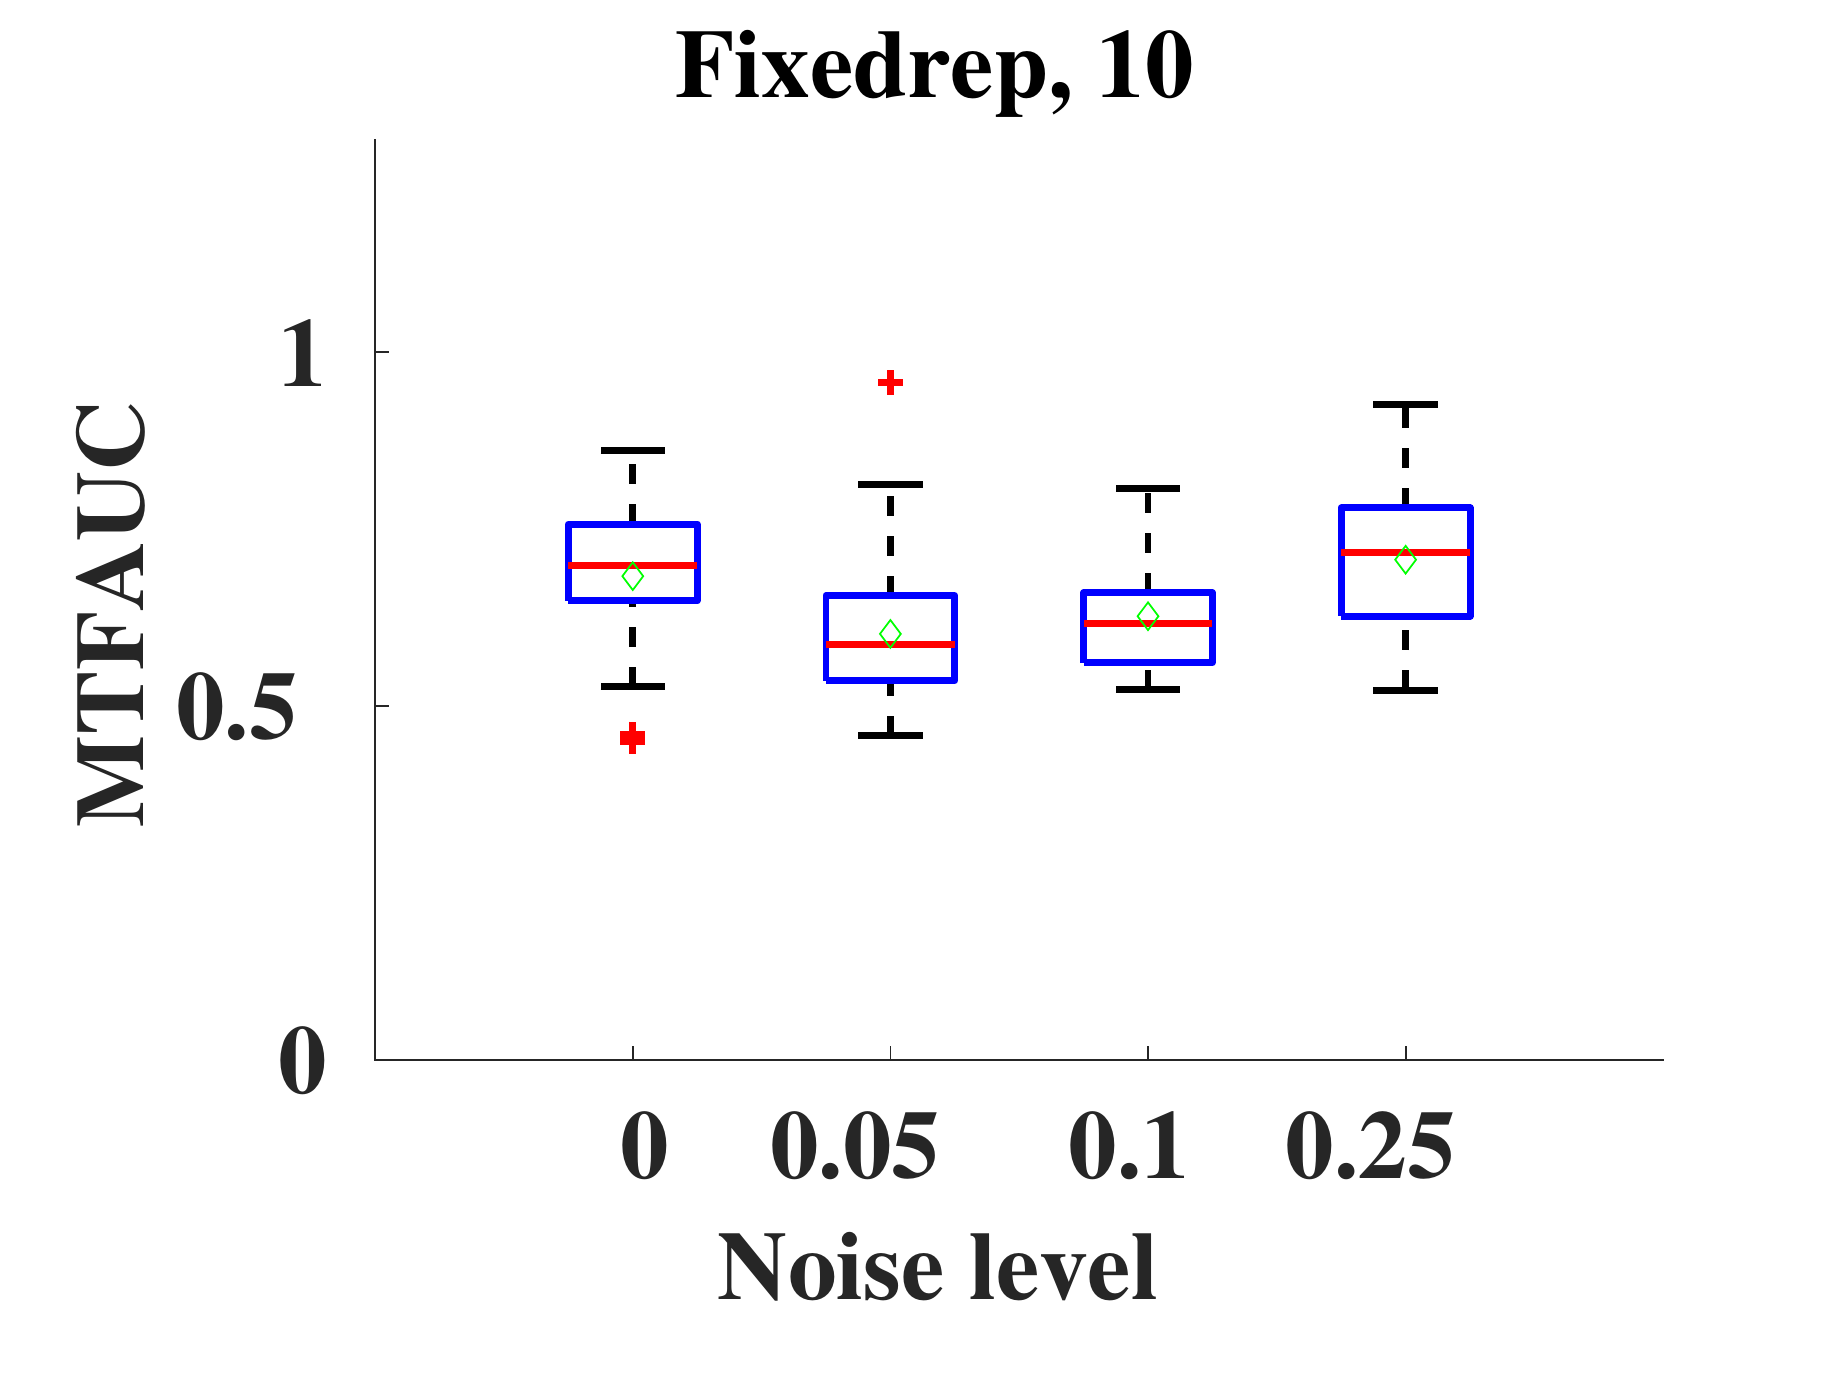}}
    \end{minipage}

    \begin{minipage}{\linewidth}
        \subfloat[]{\includegraphics[width=0.35\textwidth]{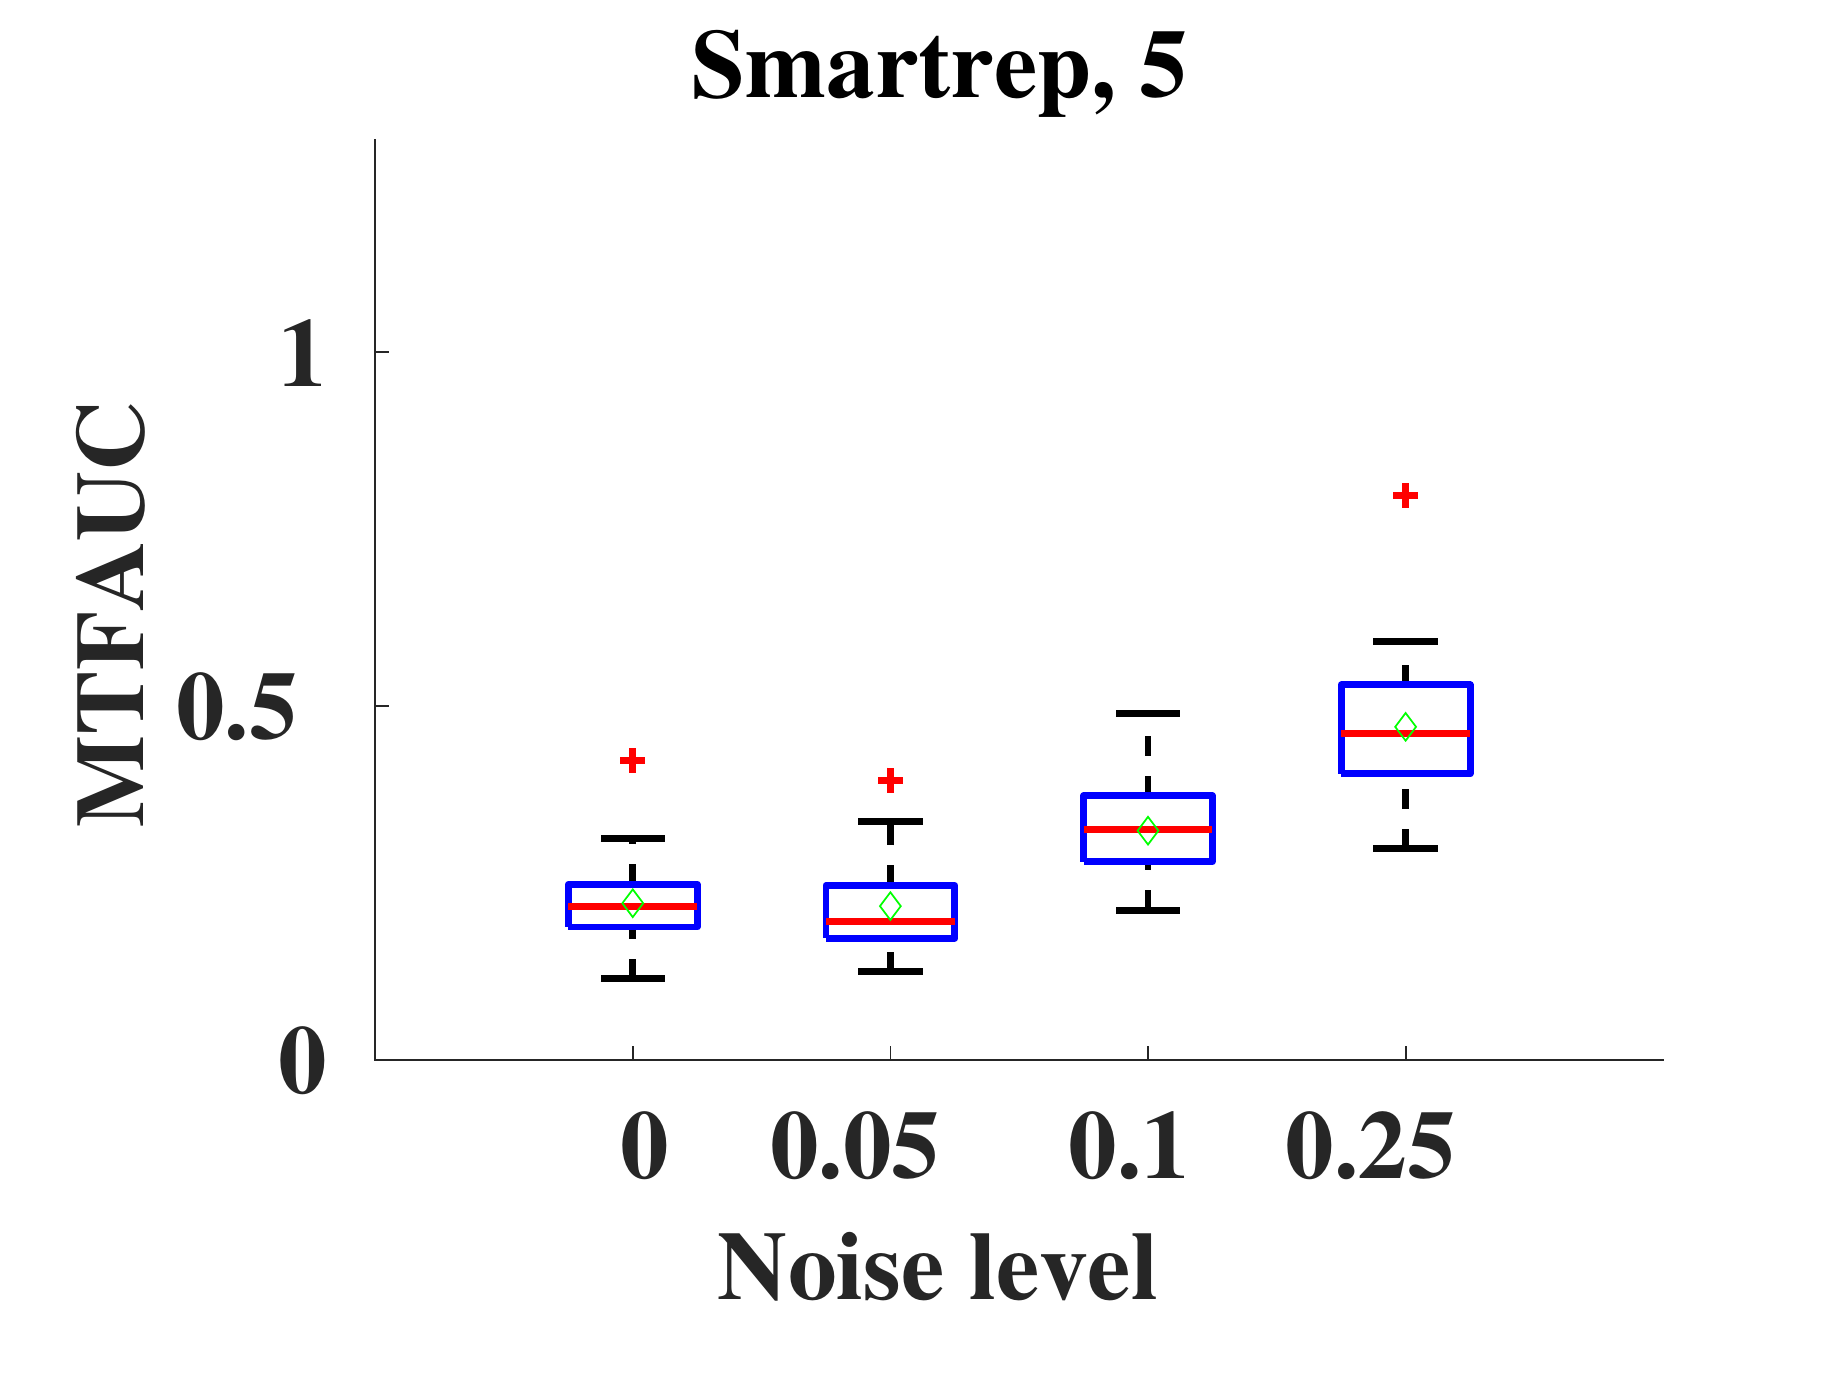}}
        \subfloat[]{\includegraphics[width=0.35\textwidth]{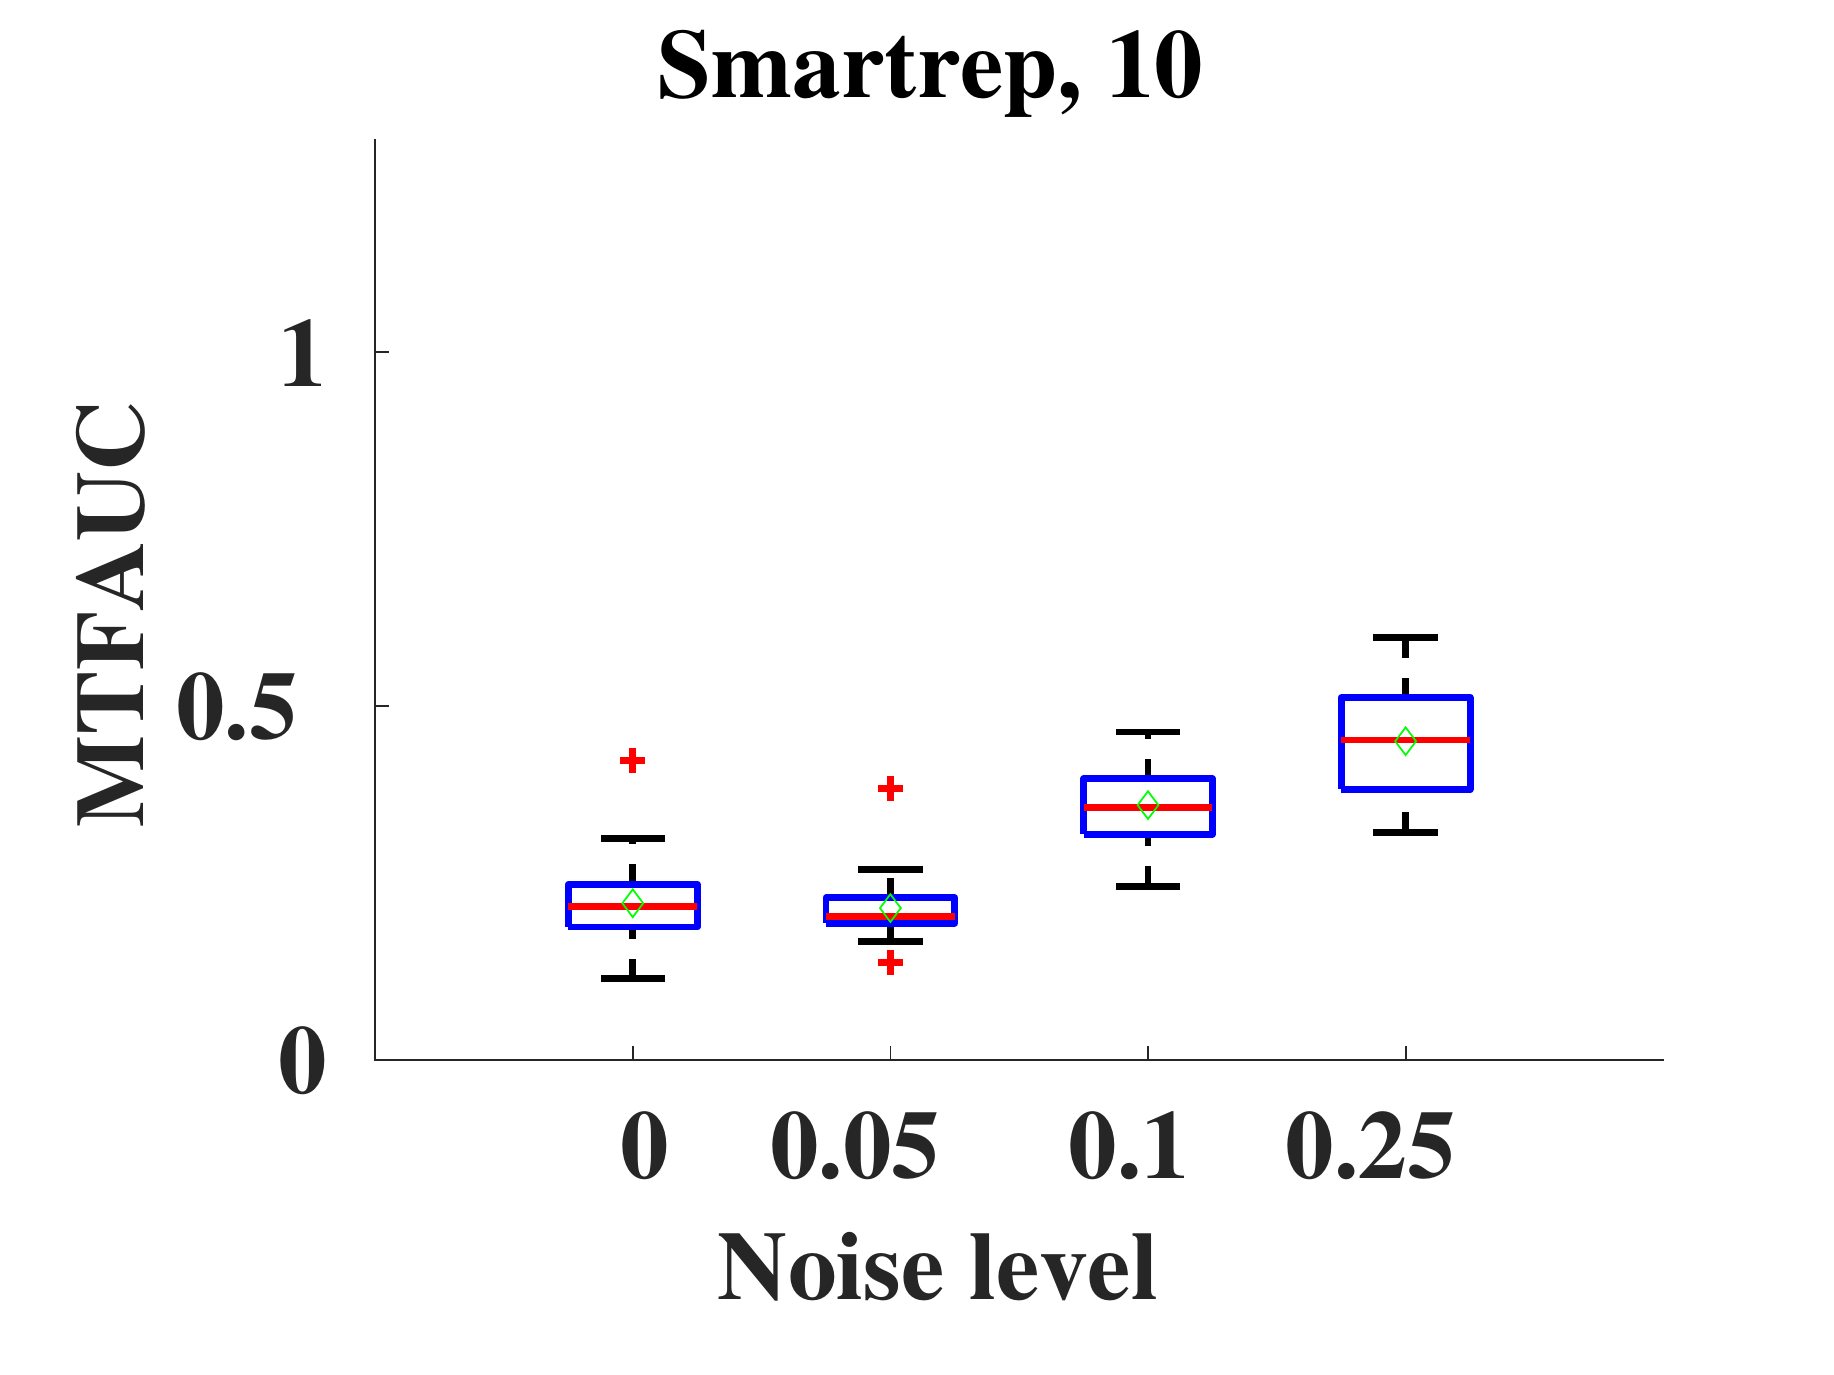}}
    \end{minipage}
    \caption{Box-plots of MTFAUC of surrogate optimization using TK-MARS on the Levy function}
    \label{fig:auc_box_levy}
    \vspace{-5mm}
\end{figure}
\begin{figure}[!htp]
\centering
    \begin{minipage}{\linewidth}
        \subfloat[]{\includegraphics[width=0.35\textwidth]{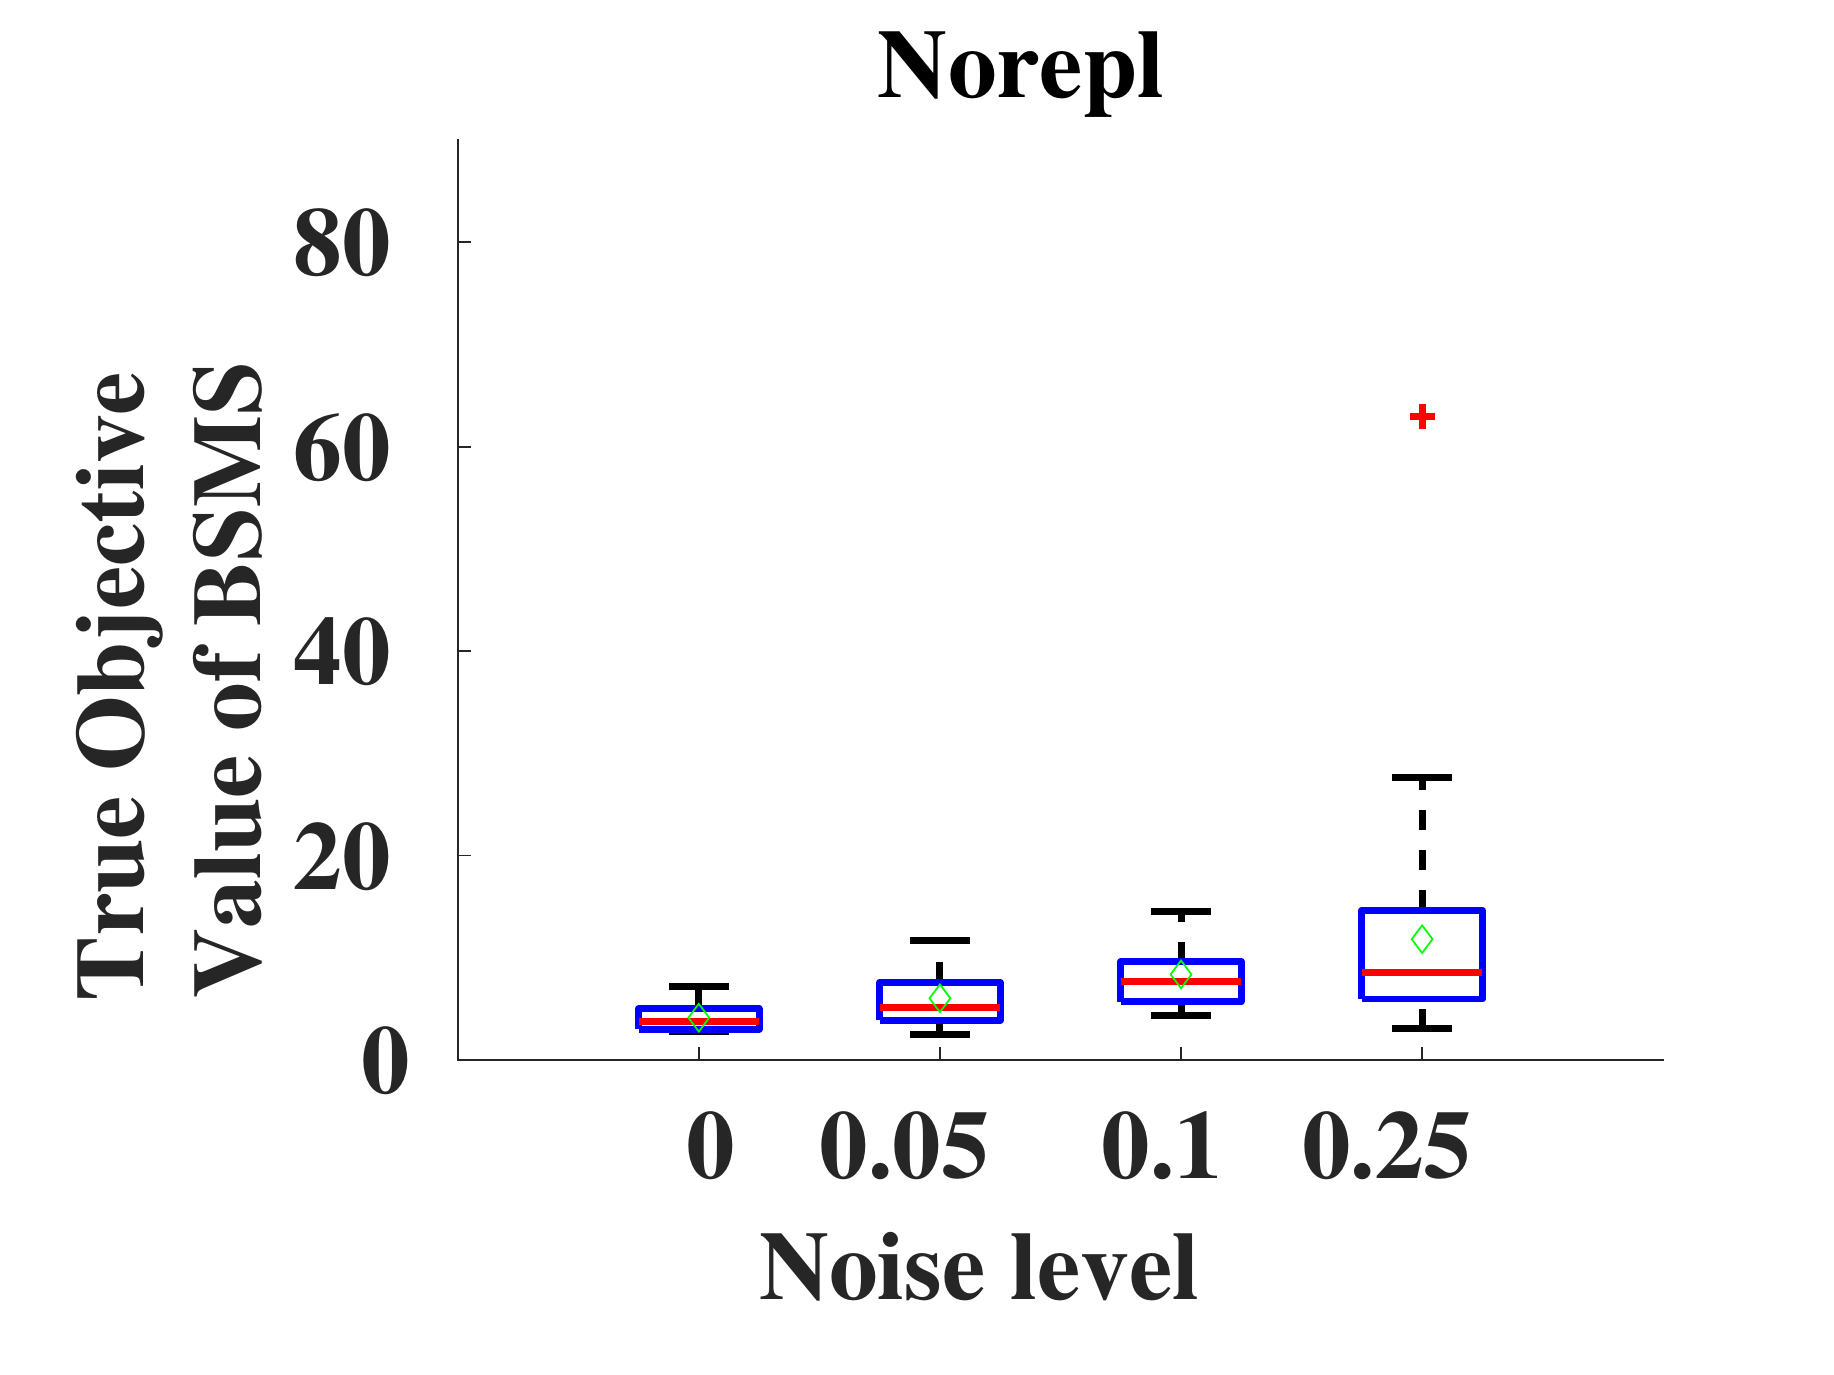}}
        \subfloat[]{\includegraphics[width=0.35\textwidth]{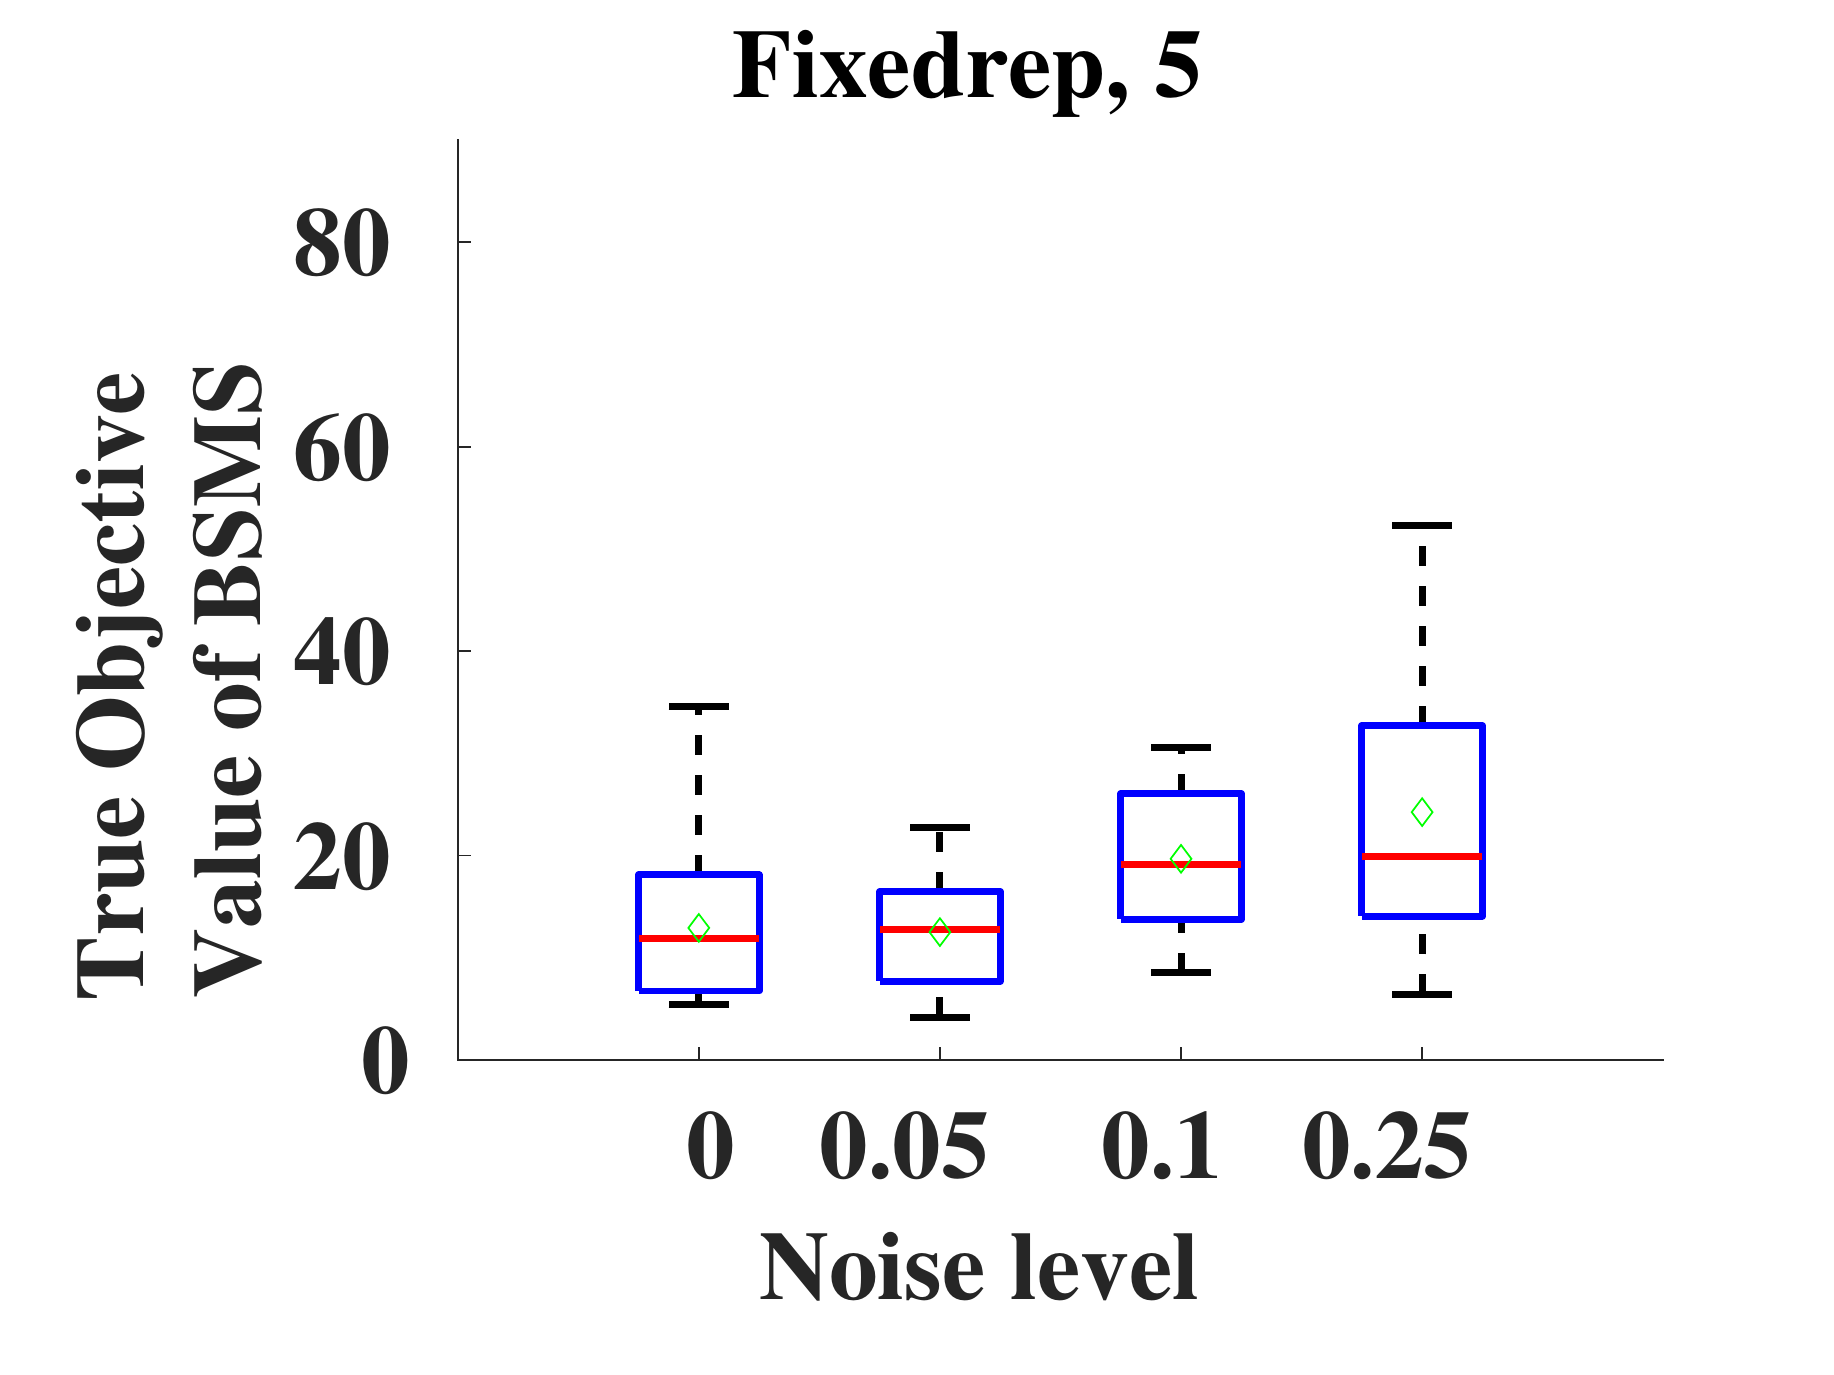}}
        \subfloat[]{\includegraphics[width=0.35\textwidth]{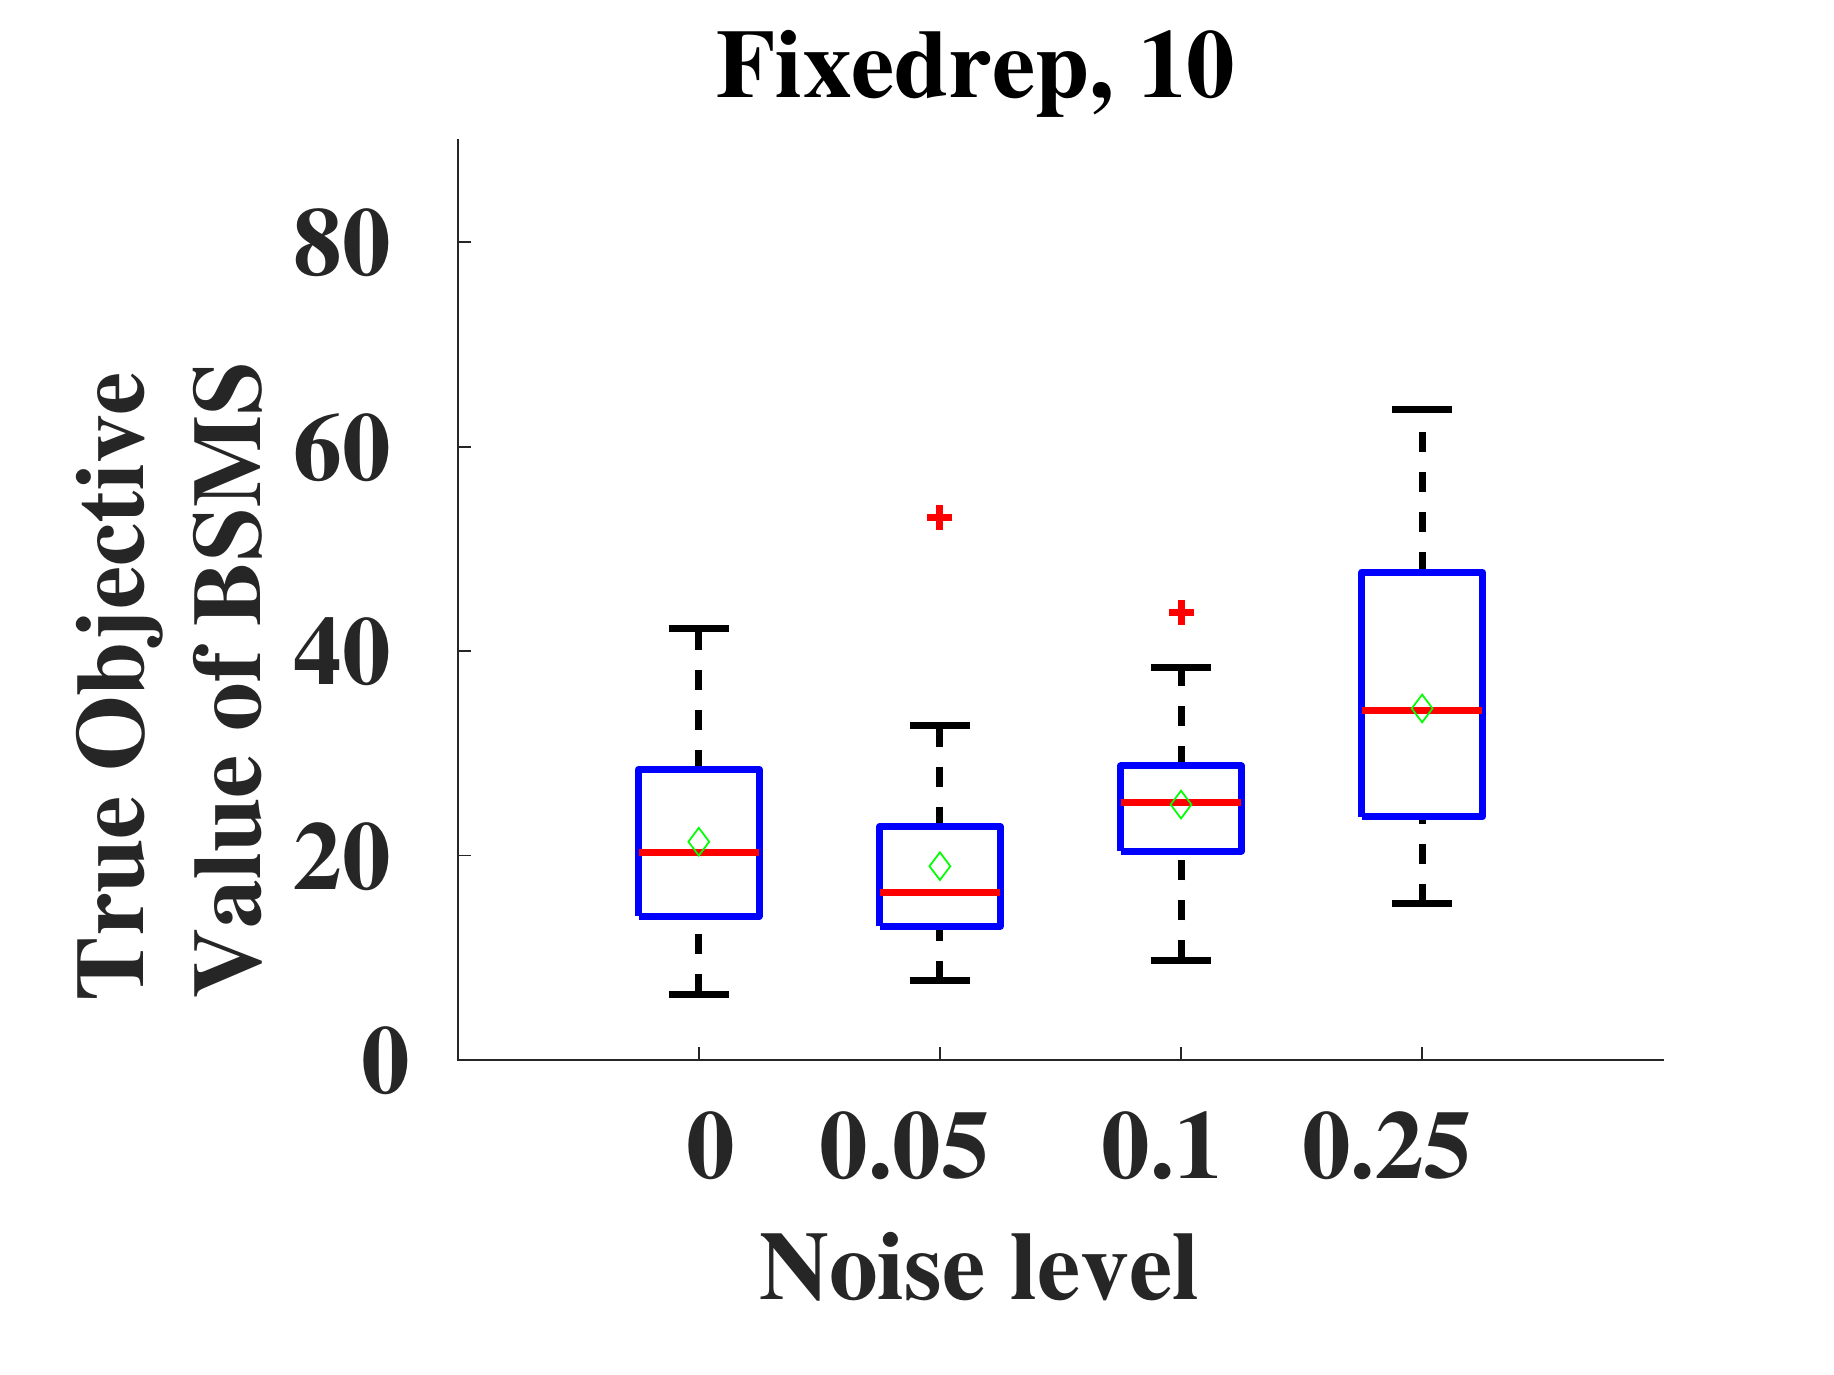}}
    \end{minipage}

    \begin{minipage}{\linewidth}
        \subfloat[]{\includegraphics[width=0.35\textwidth]{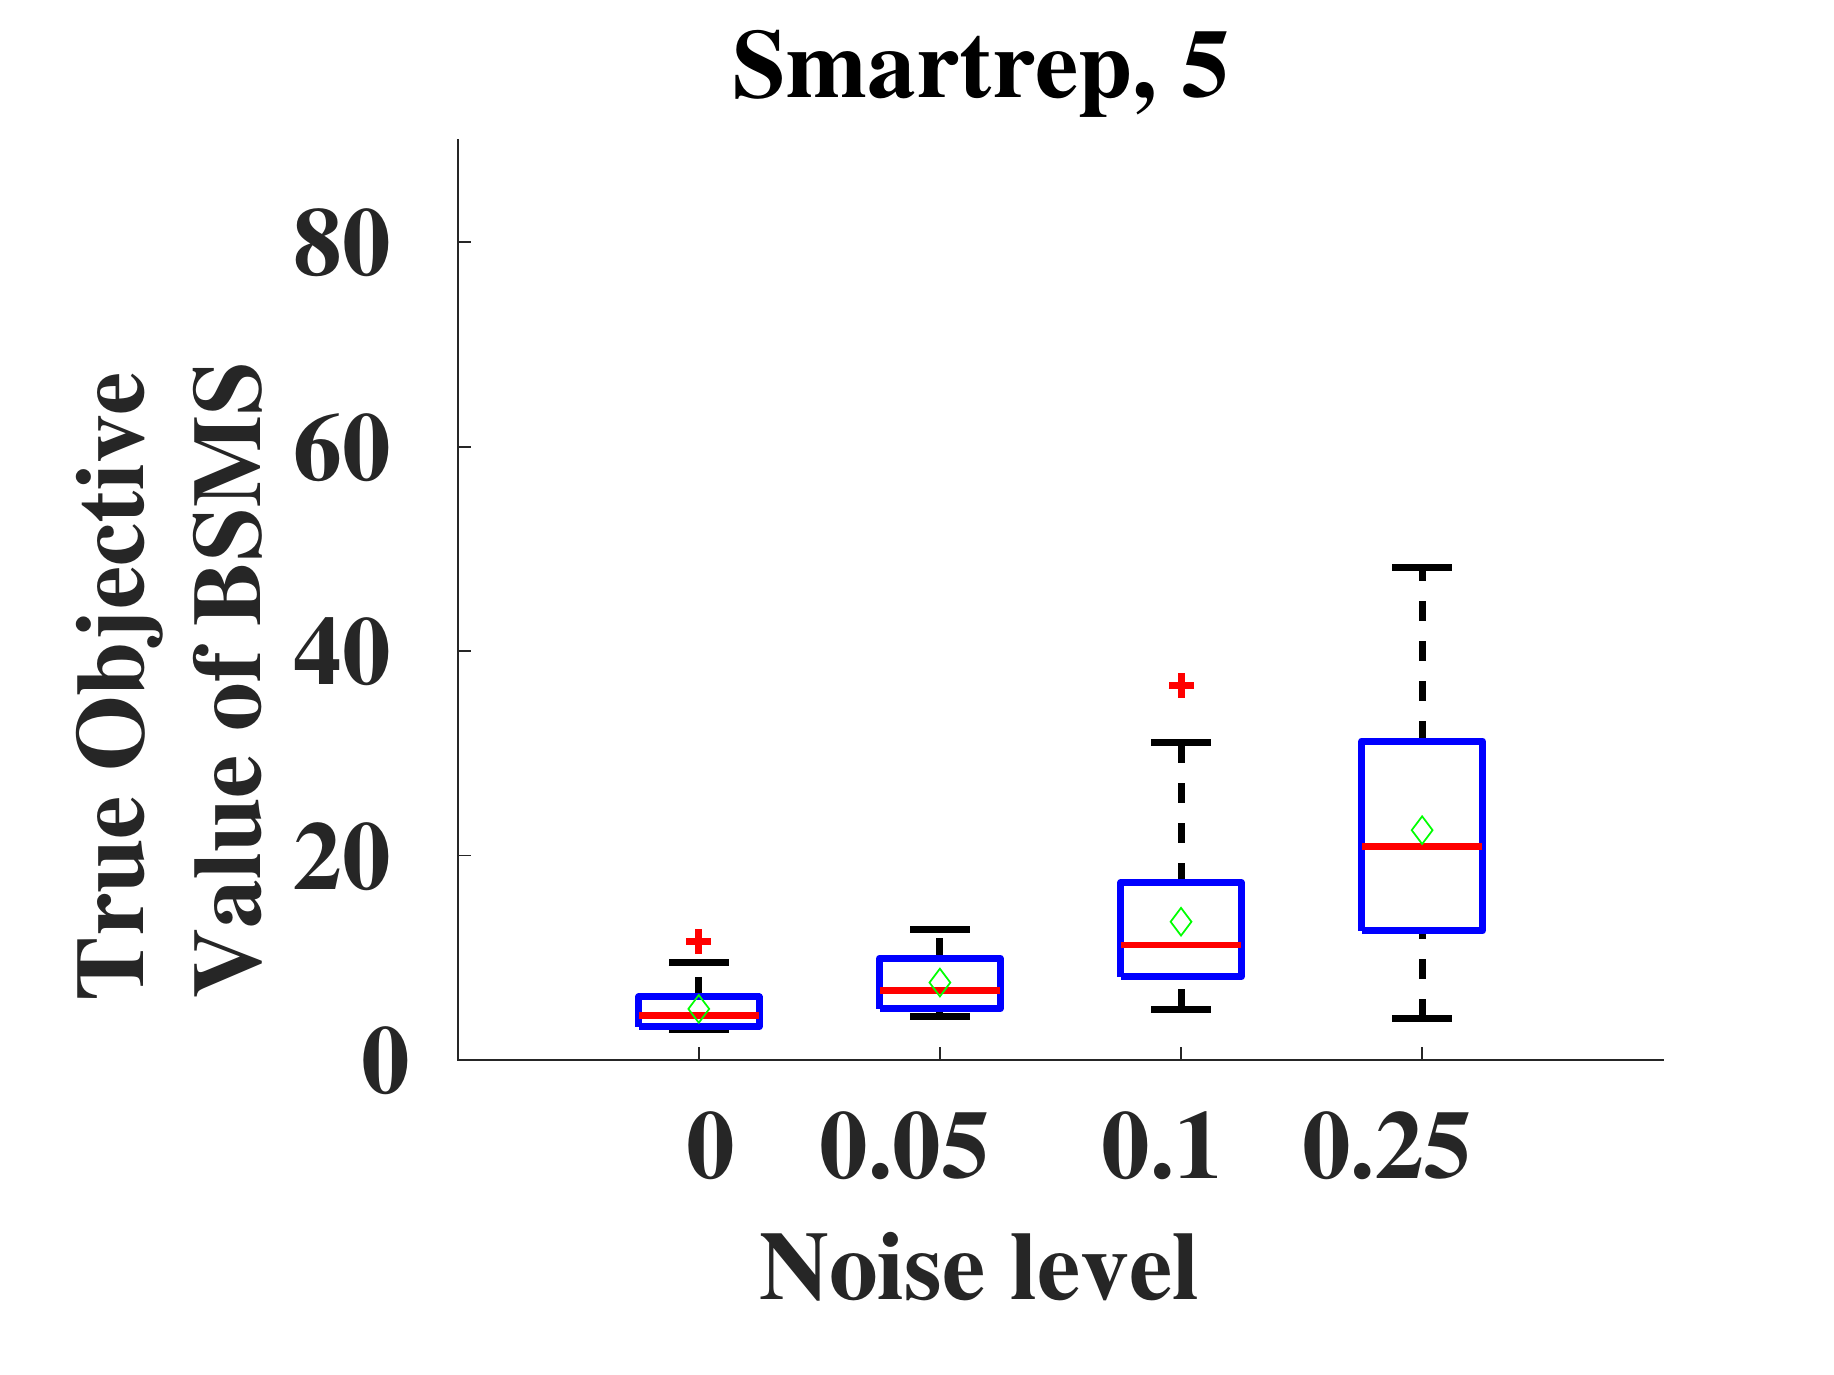}}
        \subfloat[]{\includegraphics[width=0.35\textwidth]{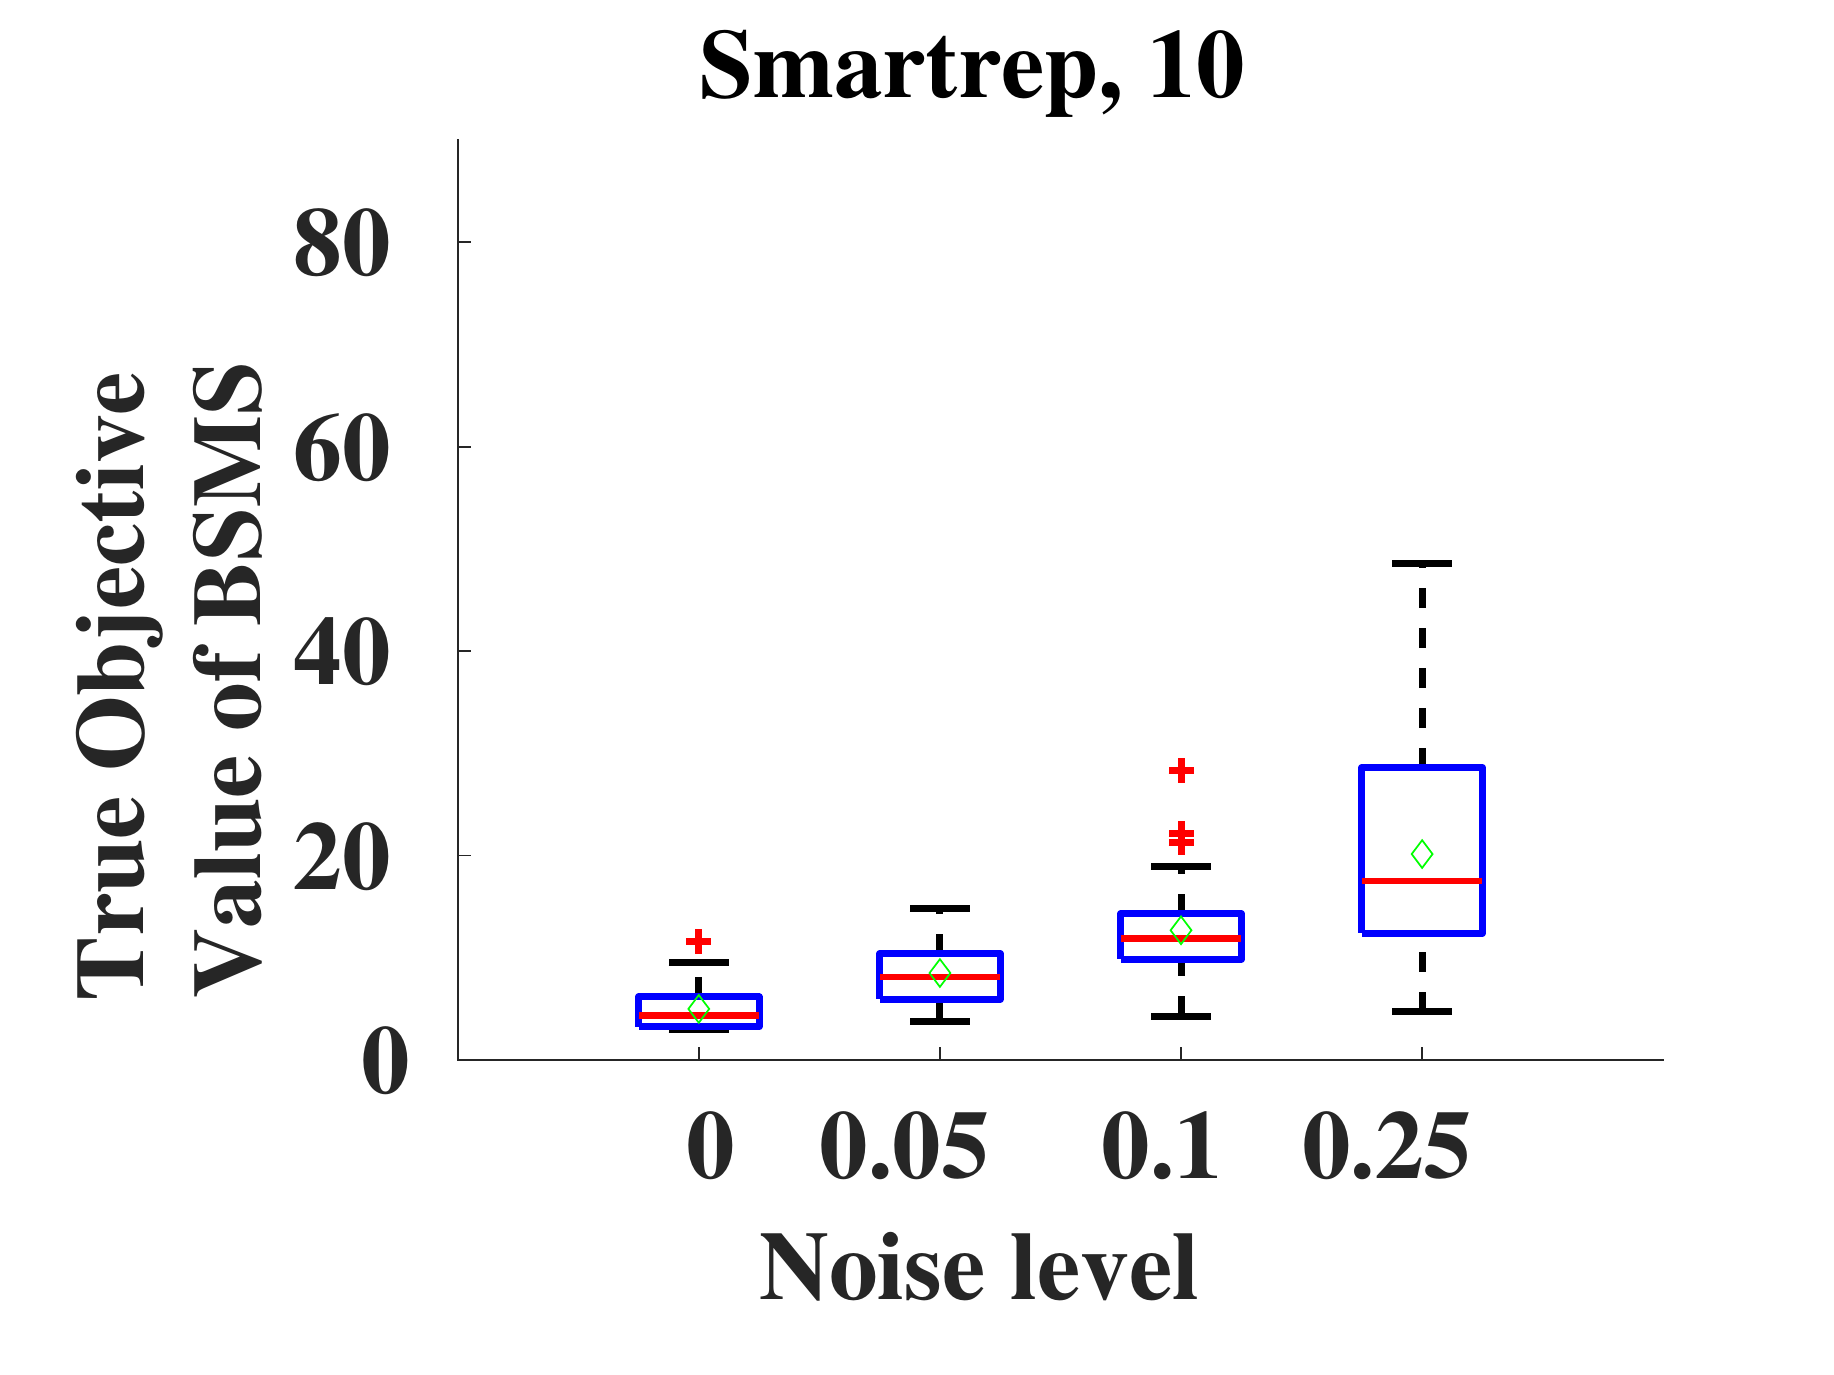}}
    \end{minipage}
    \caption{Box-plots of the true objective value of the BSMS after 1000 black-box function evaluations of surrogate optimization using TK-MARS on the Levy function}
    \label{fig:bks_box_levy}
    \vspace{-5mm}
\end{figure}



\begin{figure}[!htp]
\centering
    \begin{minipage}{\linewidth}
        \subfloat[]{\includegraphics[width=0.35\textwidth]{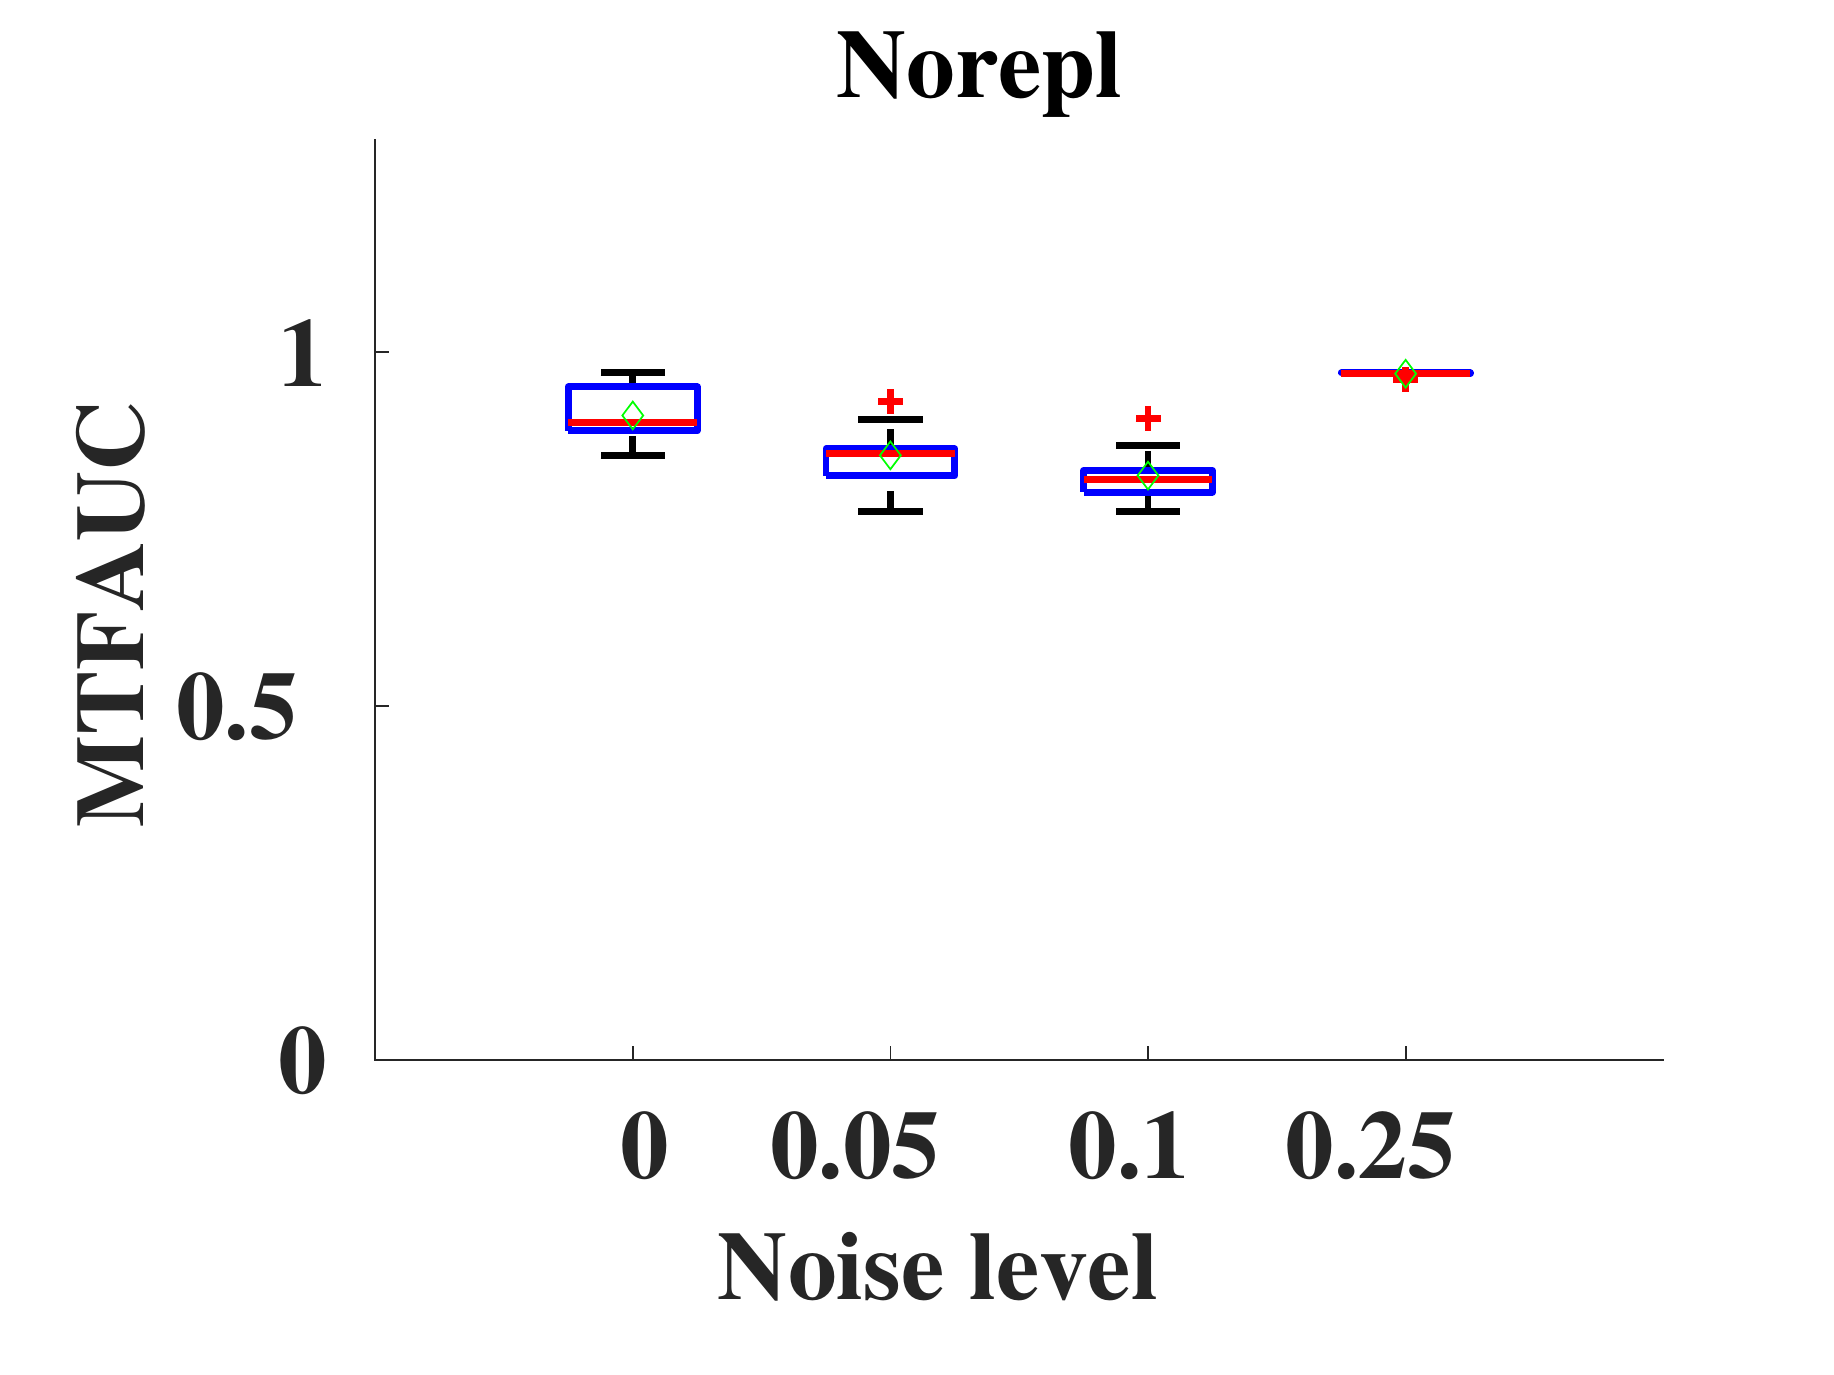}}
        \subfloat[]{\includegraphics[width=0.35\textwidth]{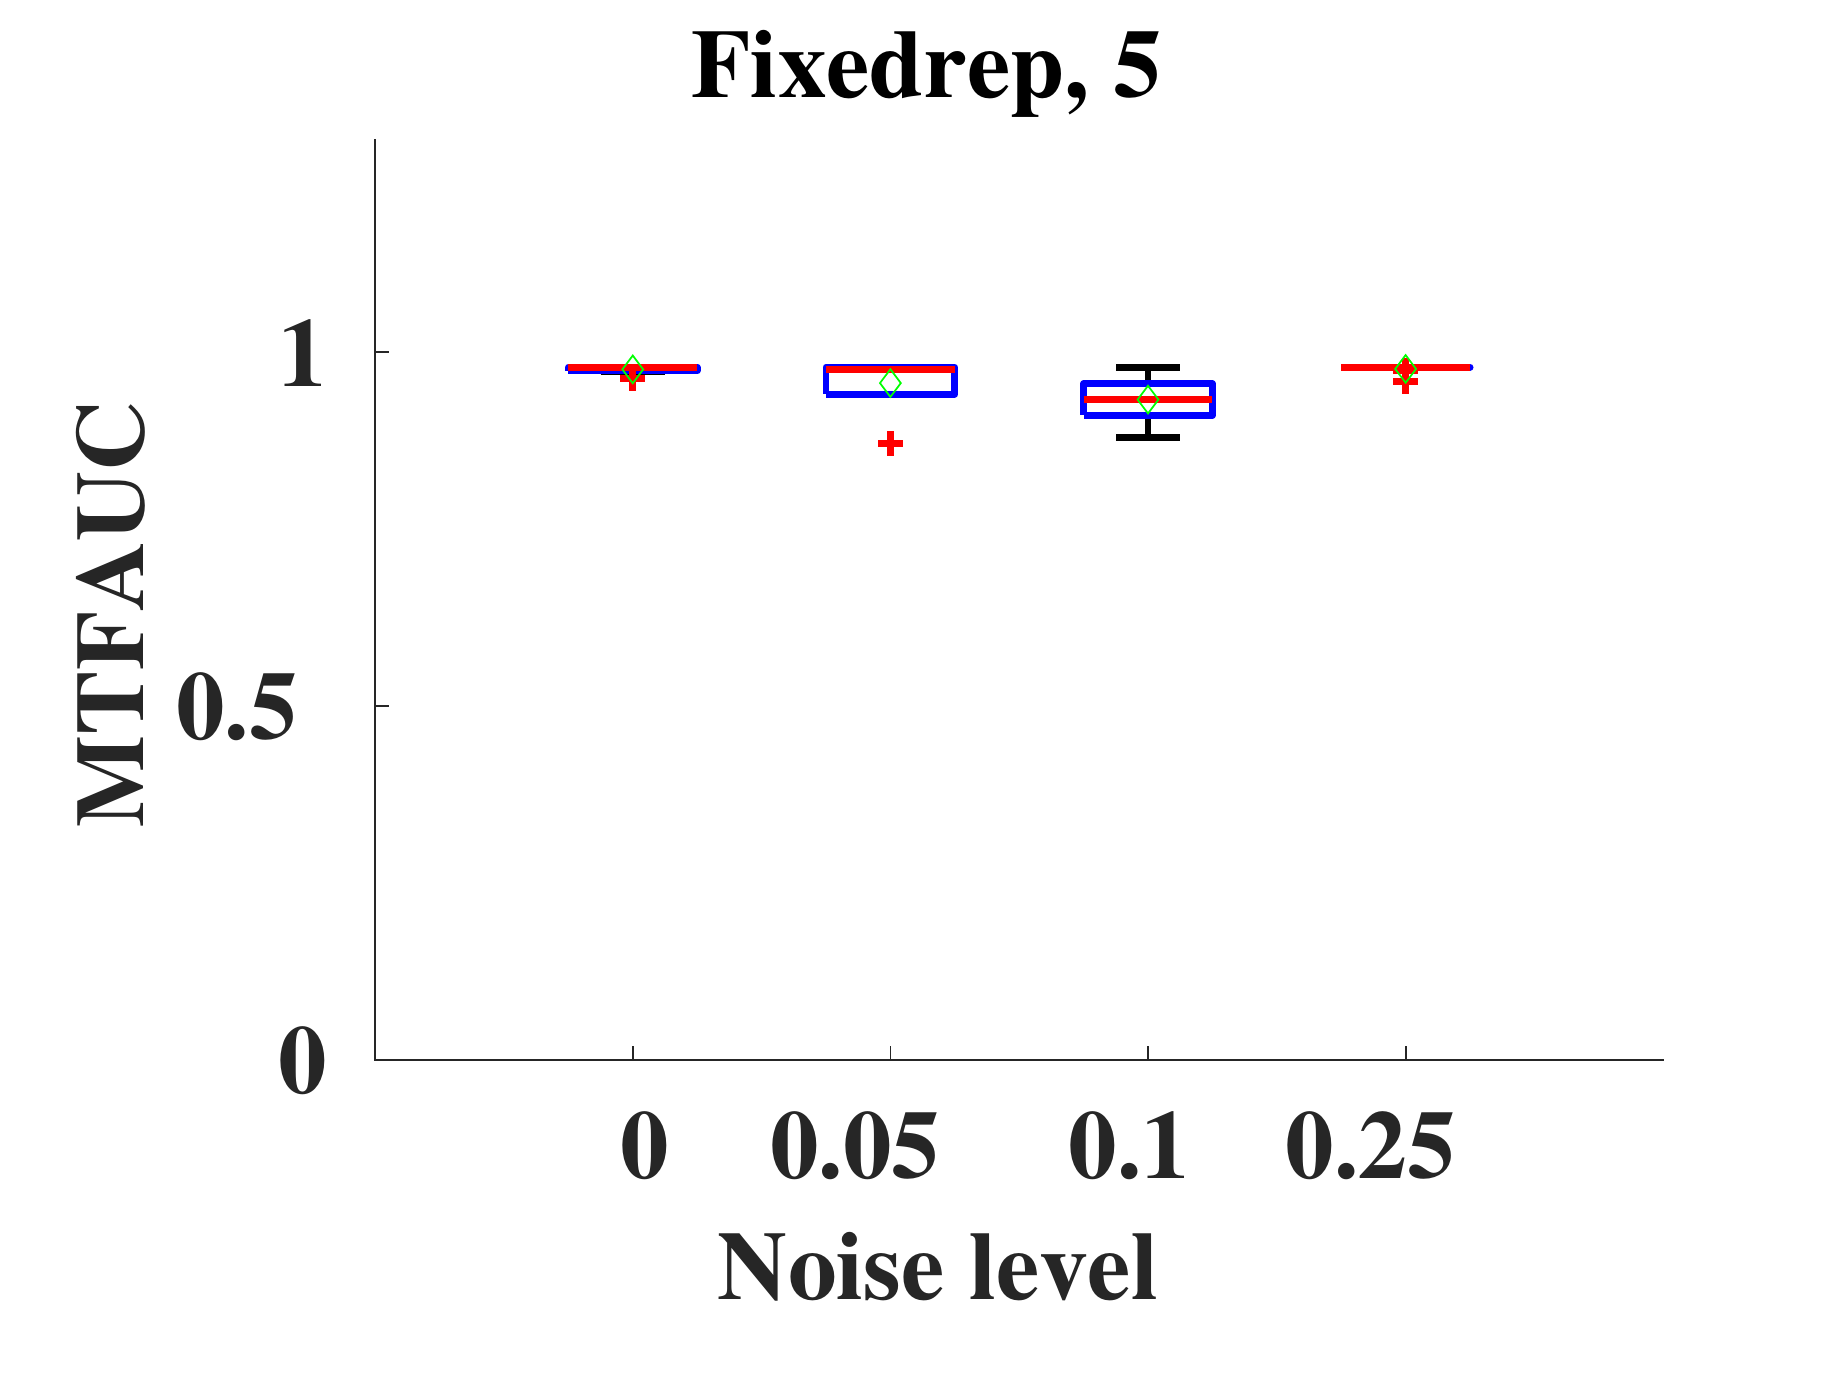}}
        \subfloat[]{\includegraphics[width=0.35\textwidth]{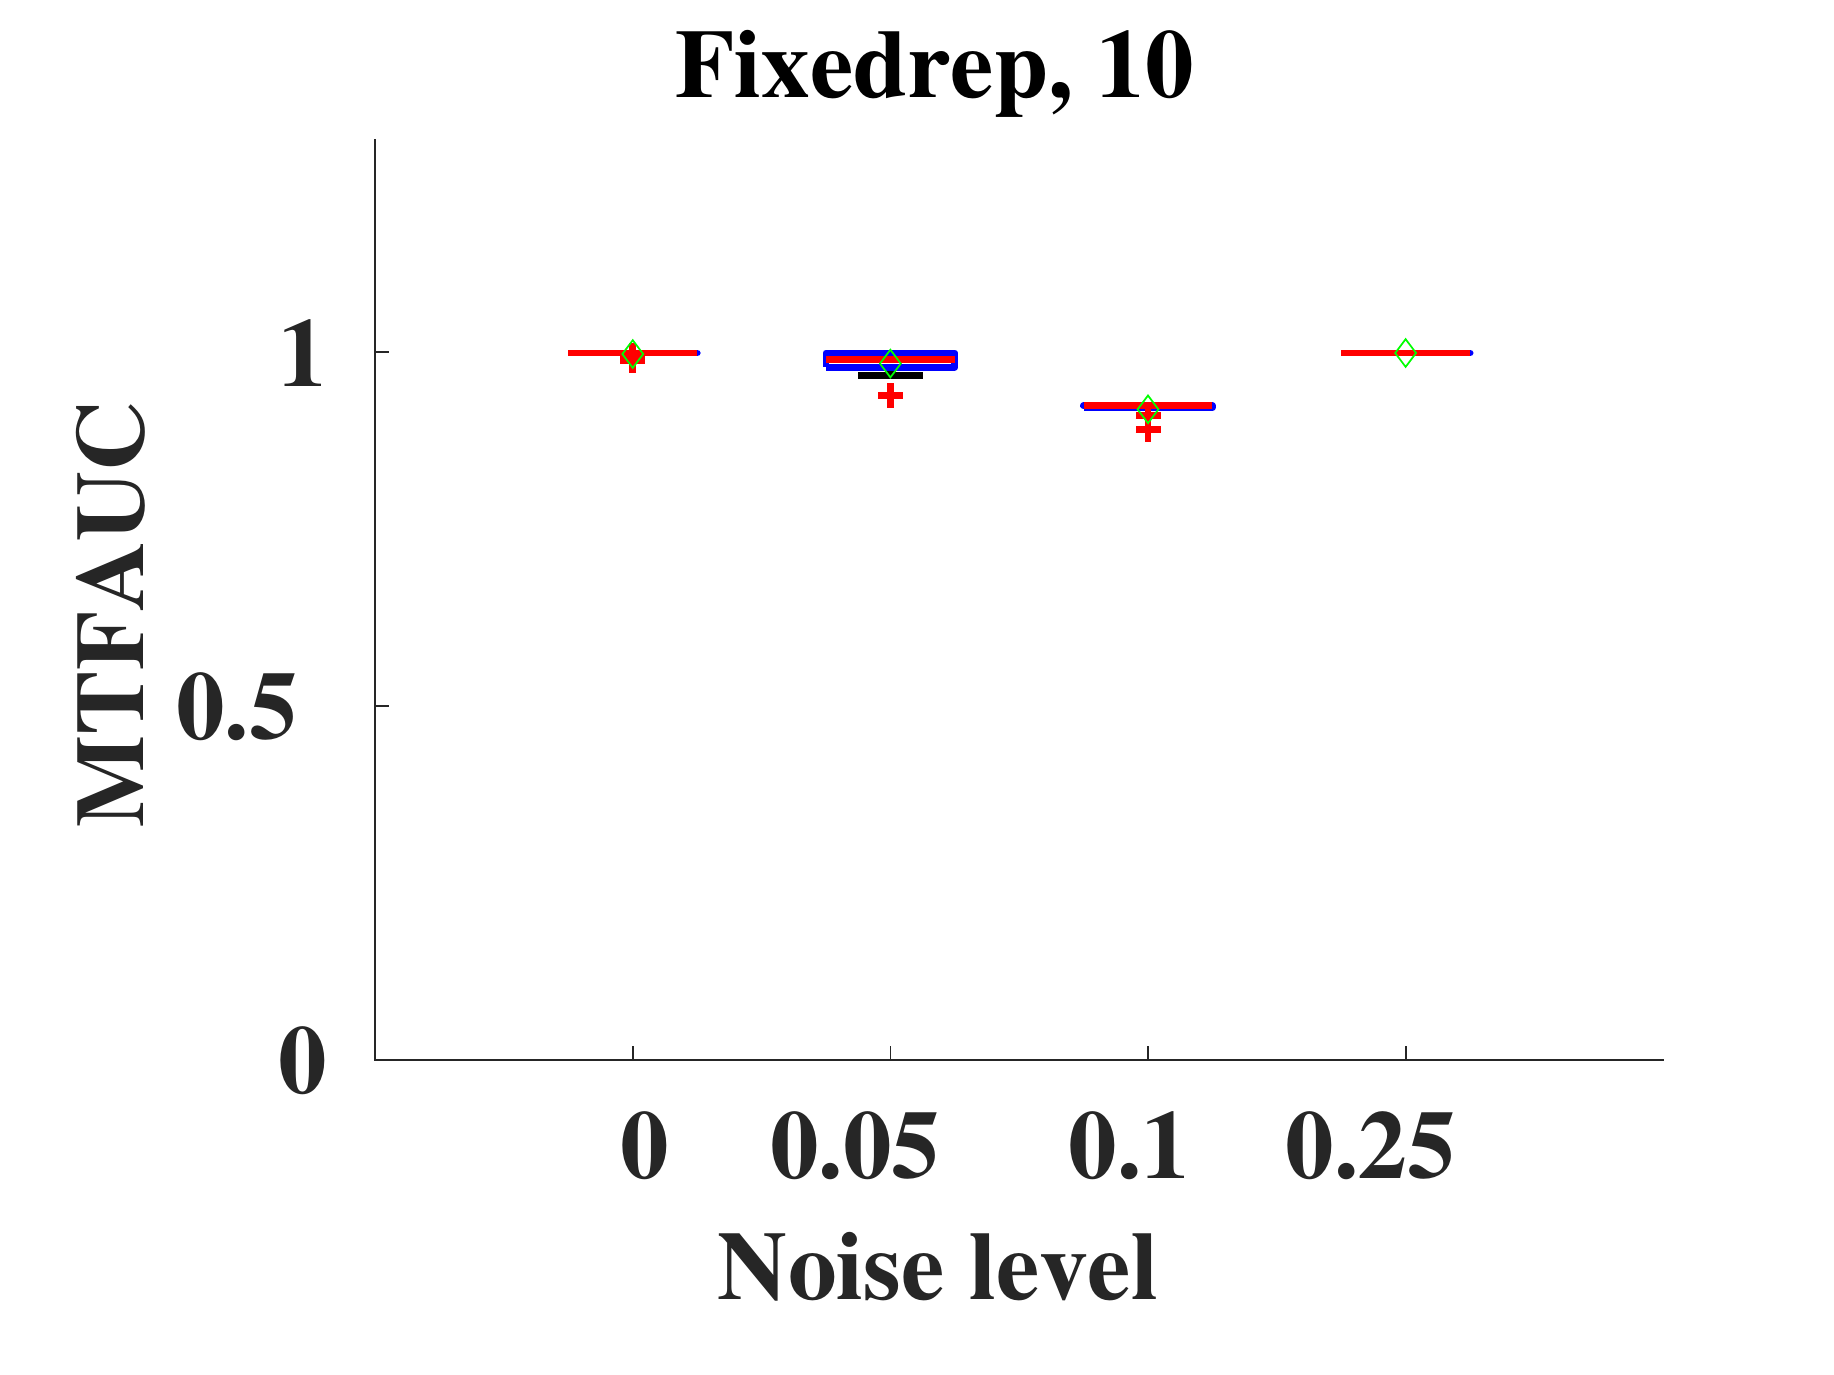}}
    \end{minipage}

    \begin{minipage}{\linewidth}
        \subfloat[]{\includegraphics[width=0.35\textwidth]{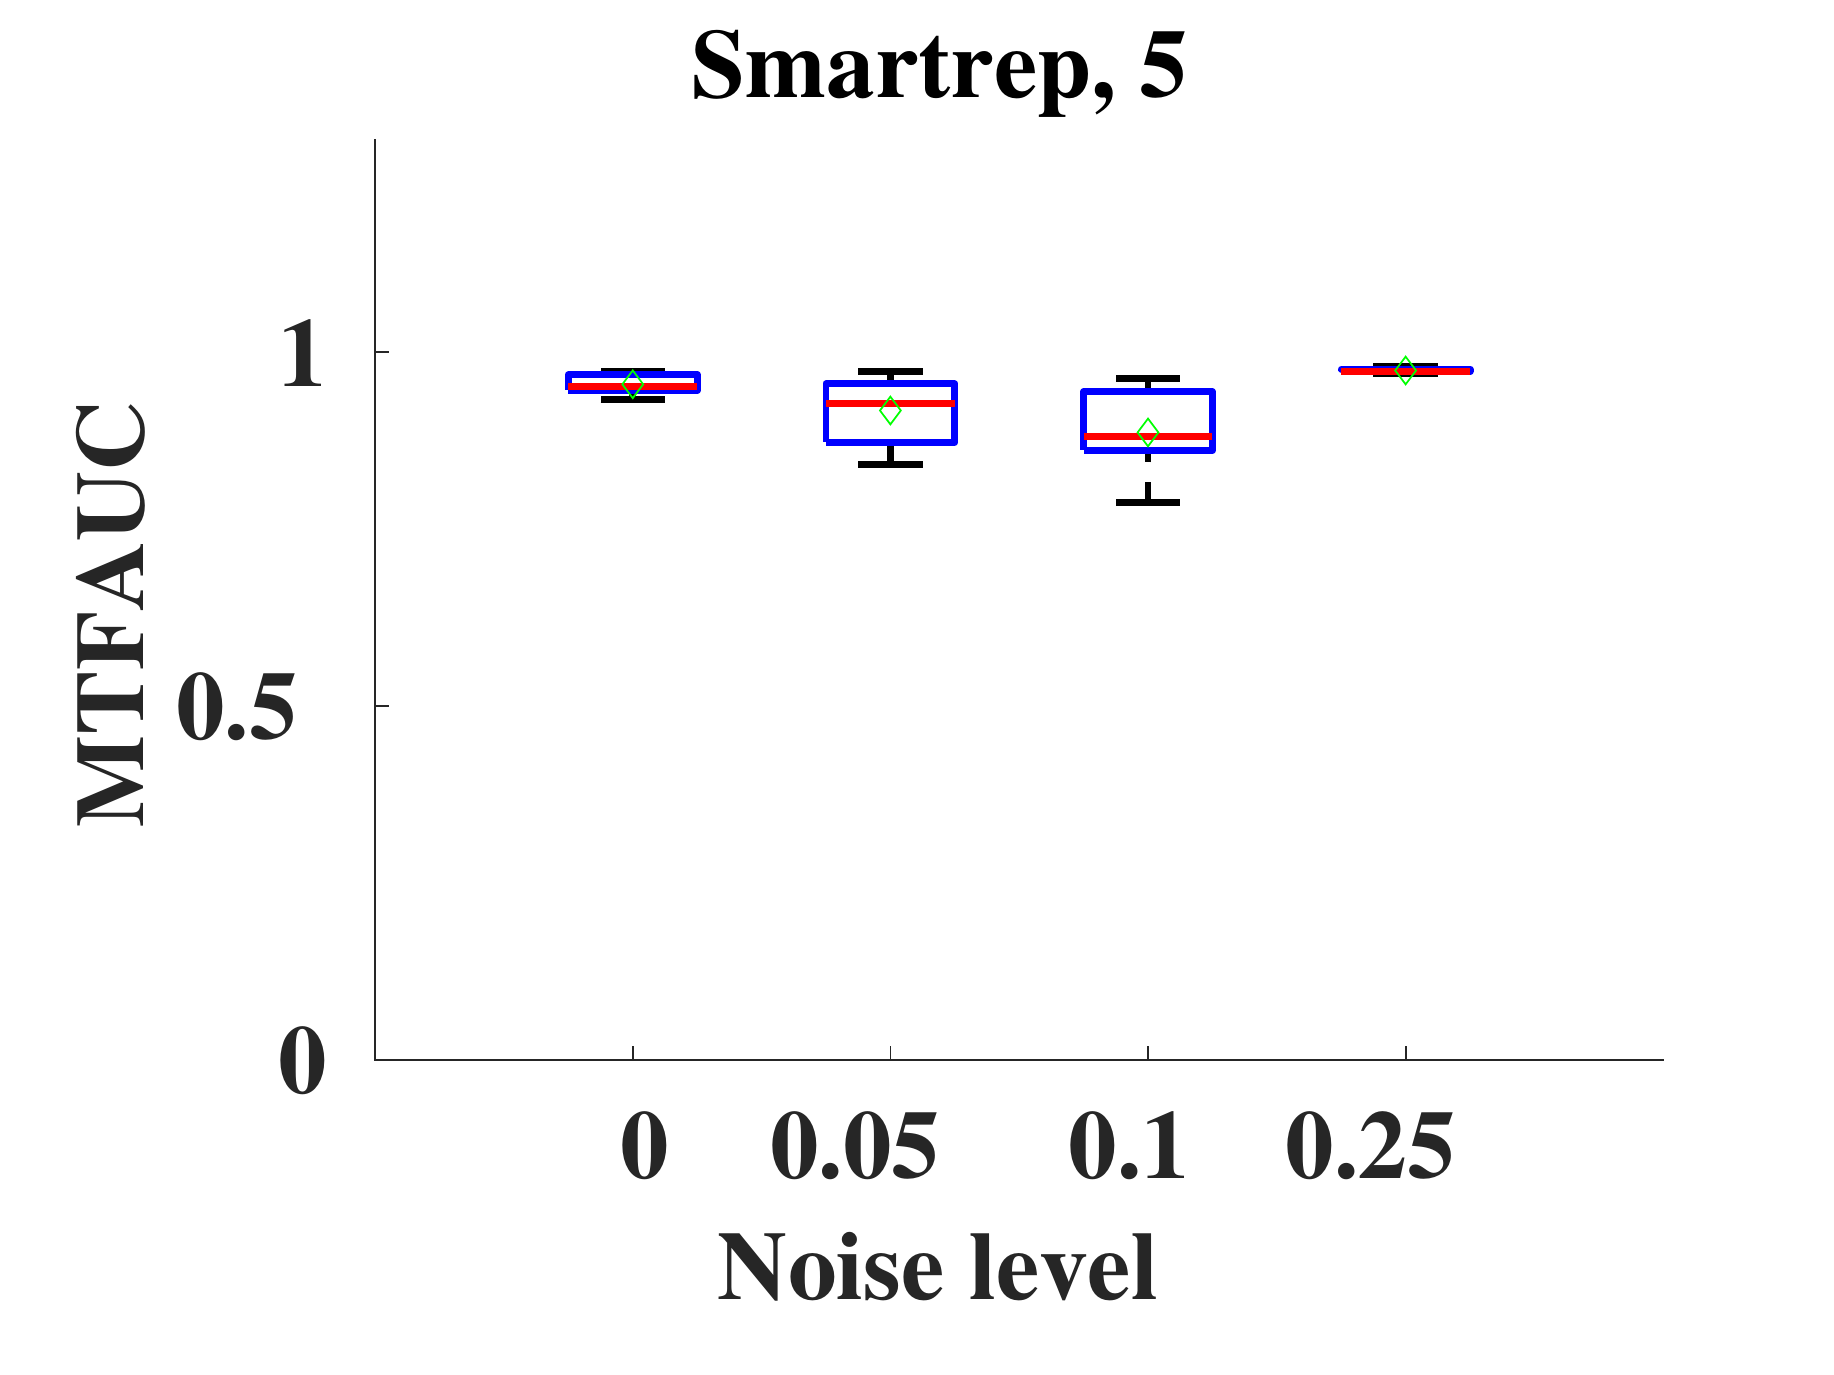}}
        \subfloat[]{\includegraphics[width=0.35\textwidth]{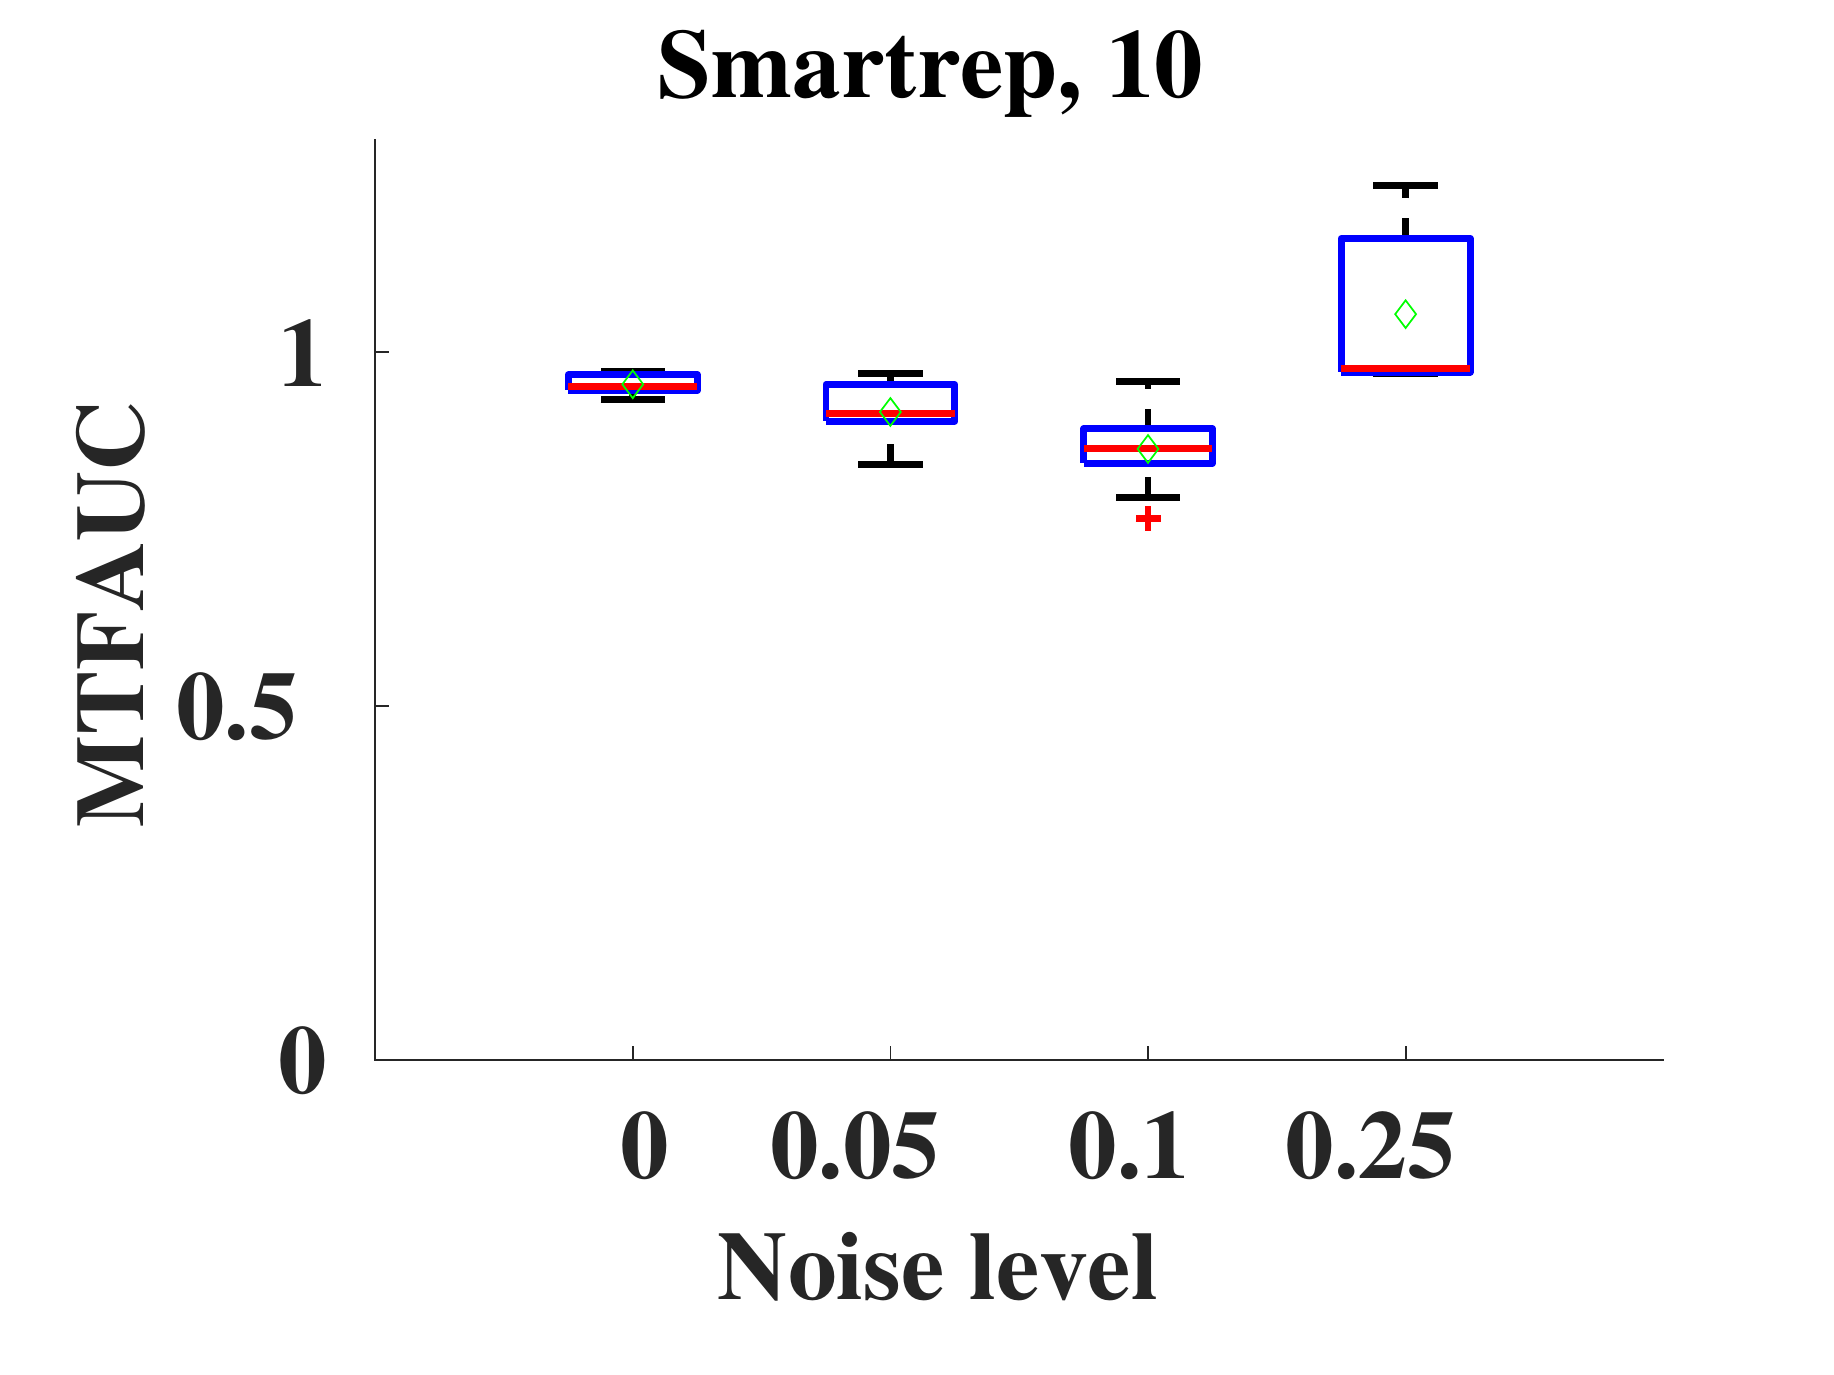}}
    \end{minipage}
    \caption{Box-plots of MTFAUC of surrogate optimization using RBF on the Rastrigin function}
    \label{fig:rbf_auc_box_rast}
    \vspace{-5mm}
\end{figure}

\begin{figure}[!htp]
\centering
    \begin{minipage}{\linewidth}
        \subfloat[]{\includegraphics[width=0.35\textwidth]{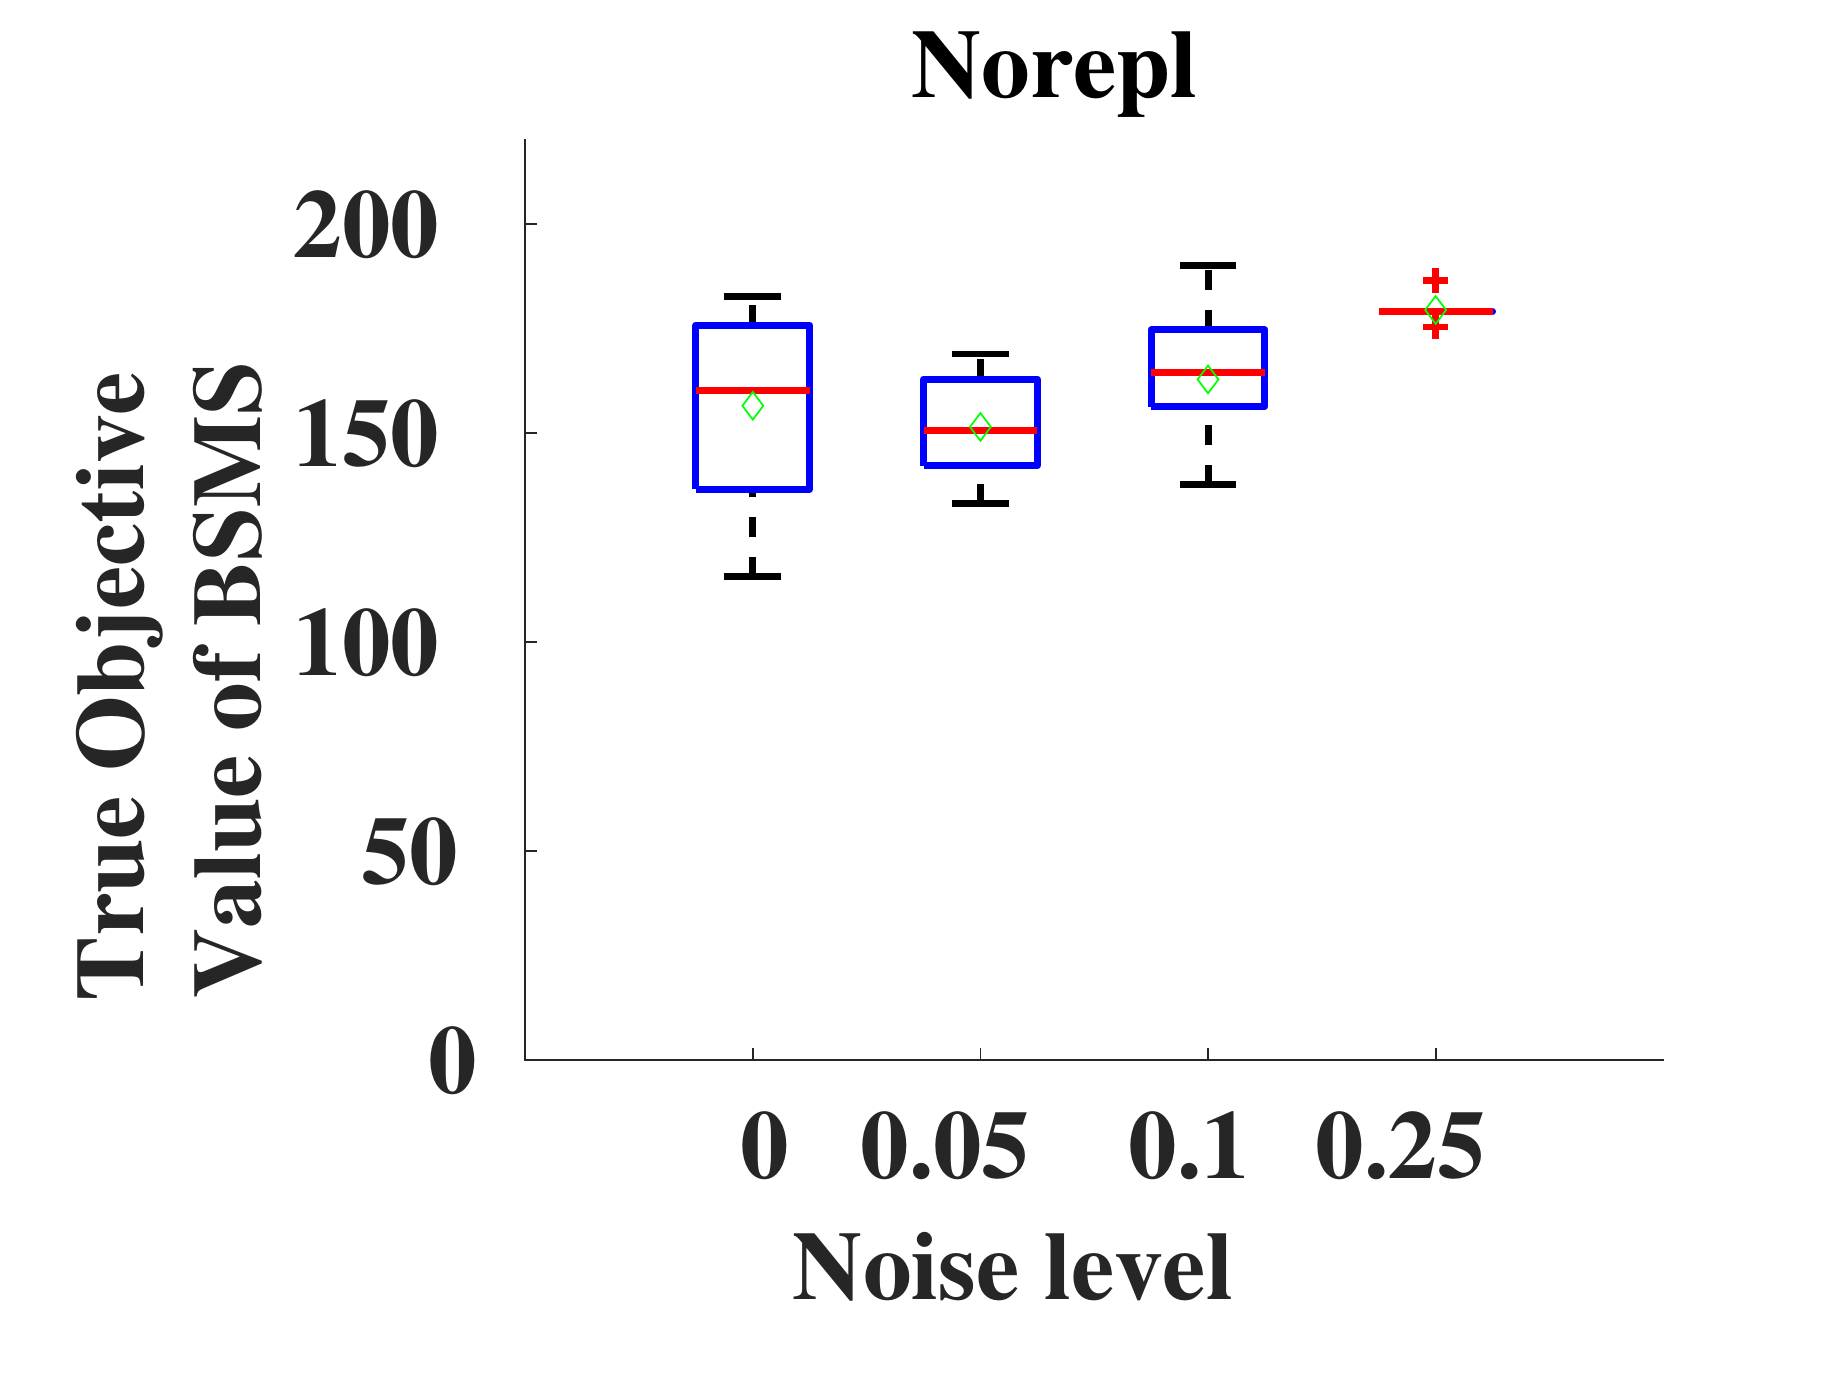}}
        \subfloat[]{\includegraphics[width=0.35\textwidth]{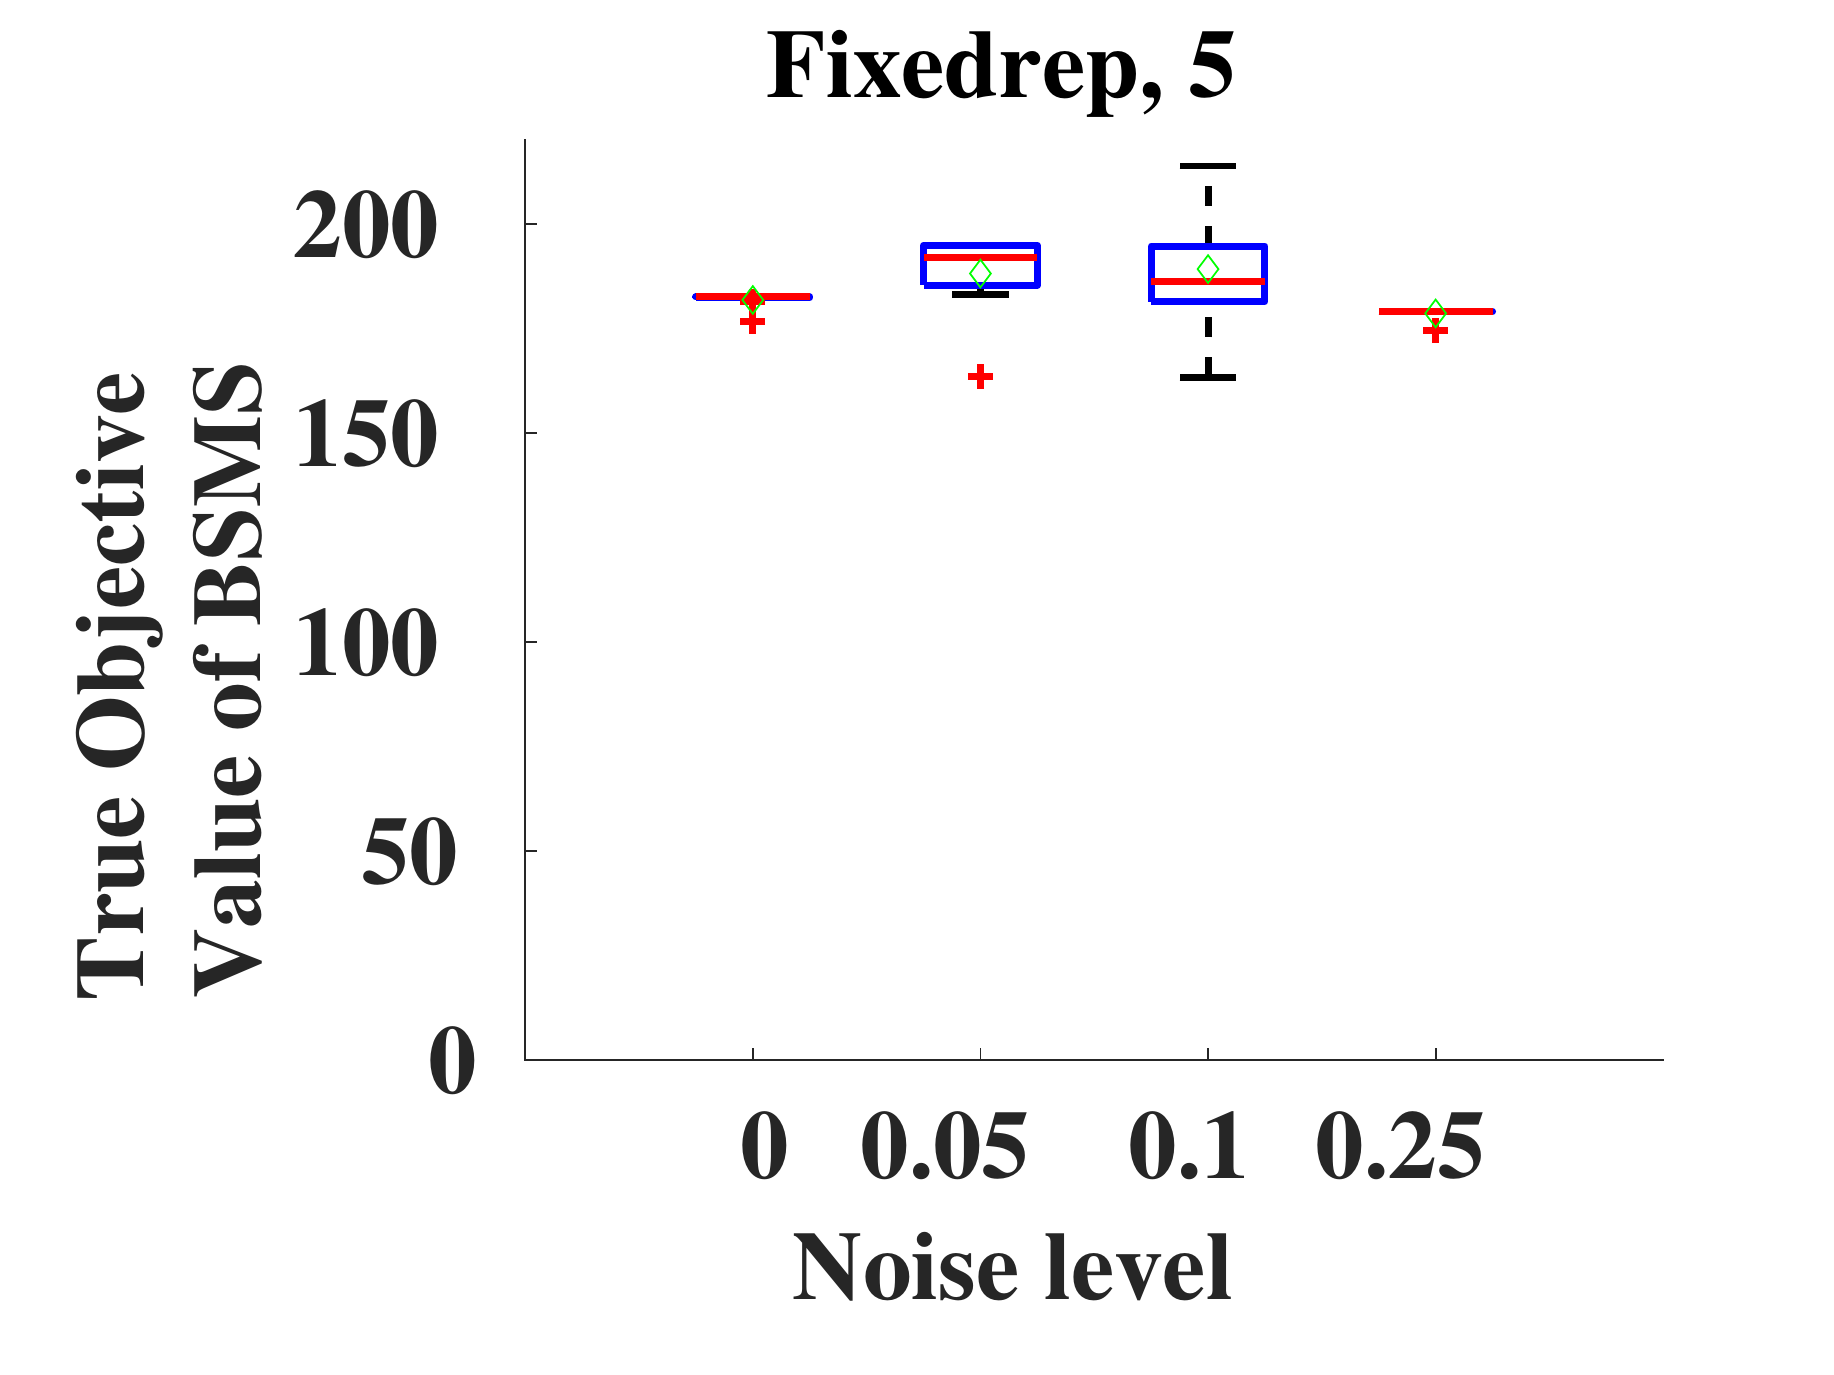}}
        \subfloat[]{\includegraphics[width=0.35\textwidth]{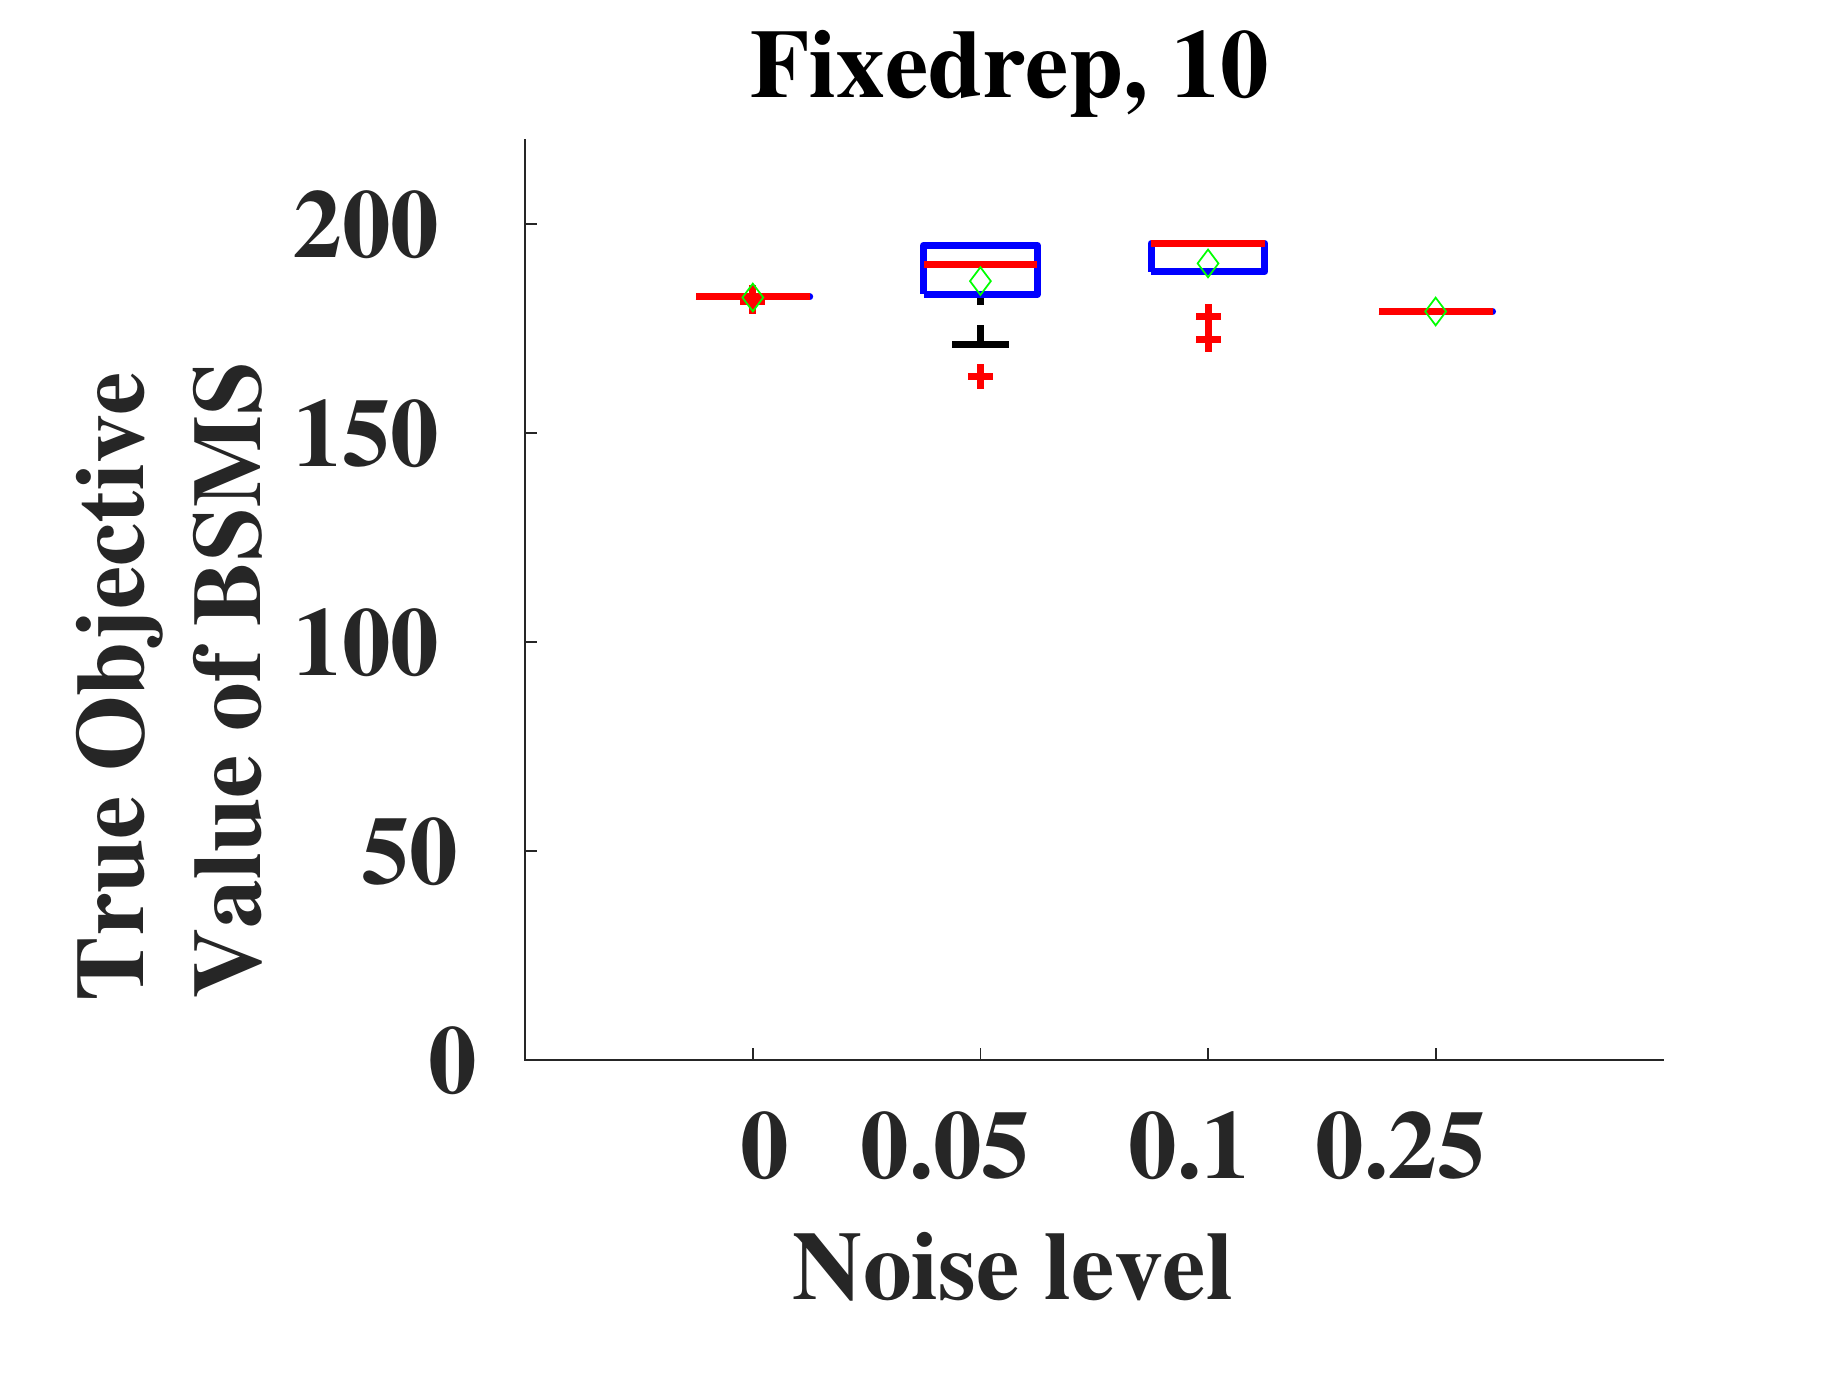}}
    \end{minipage}

    \begin{minipage}{\linewidth}
        \subfloat[]{\includegraphics[width=0.35\textwidth]{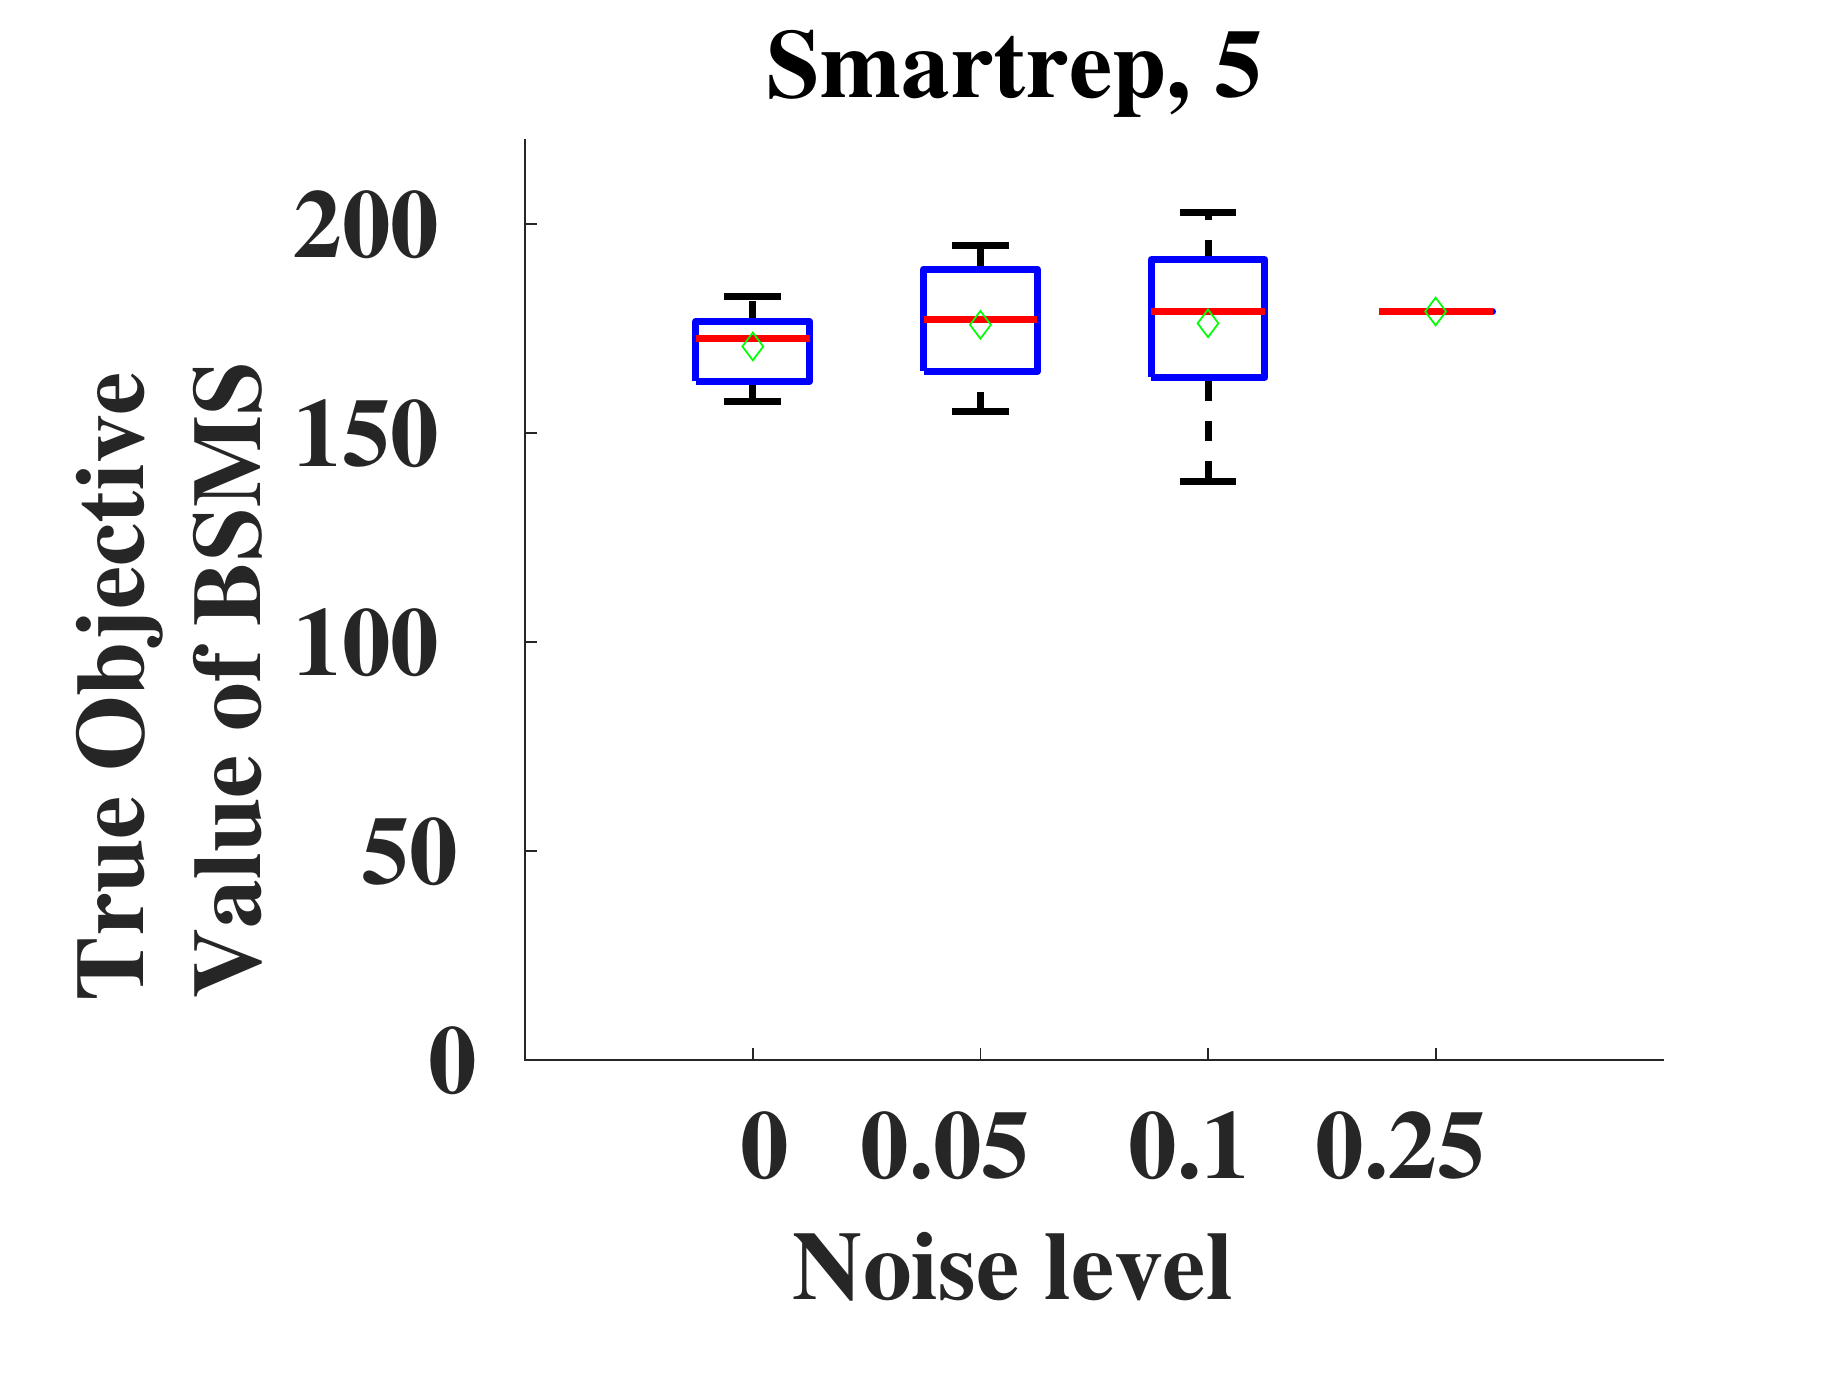}}
        \subfloat[]{\includegraphics[width=0.35\textwidth]{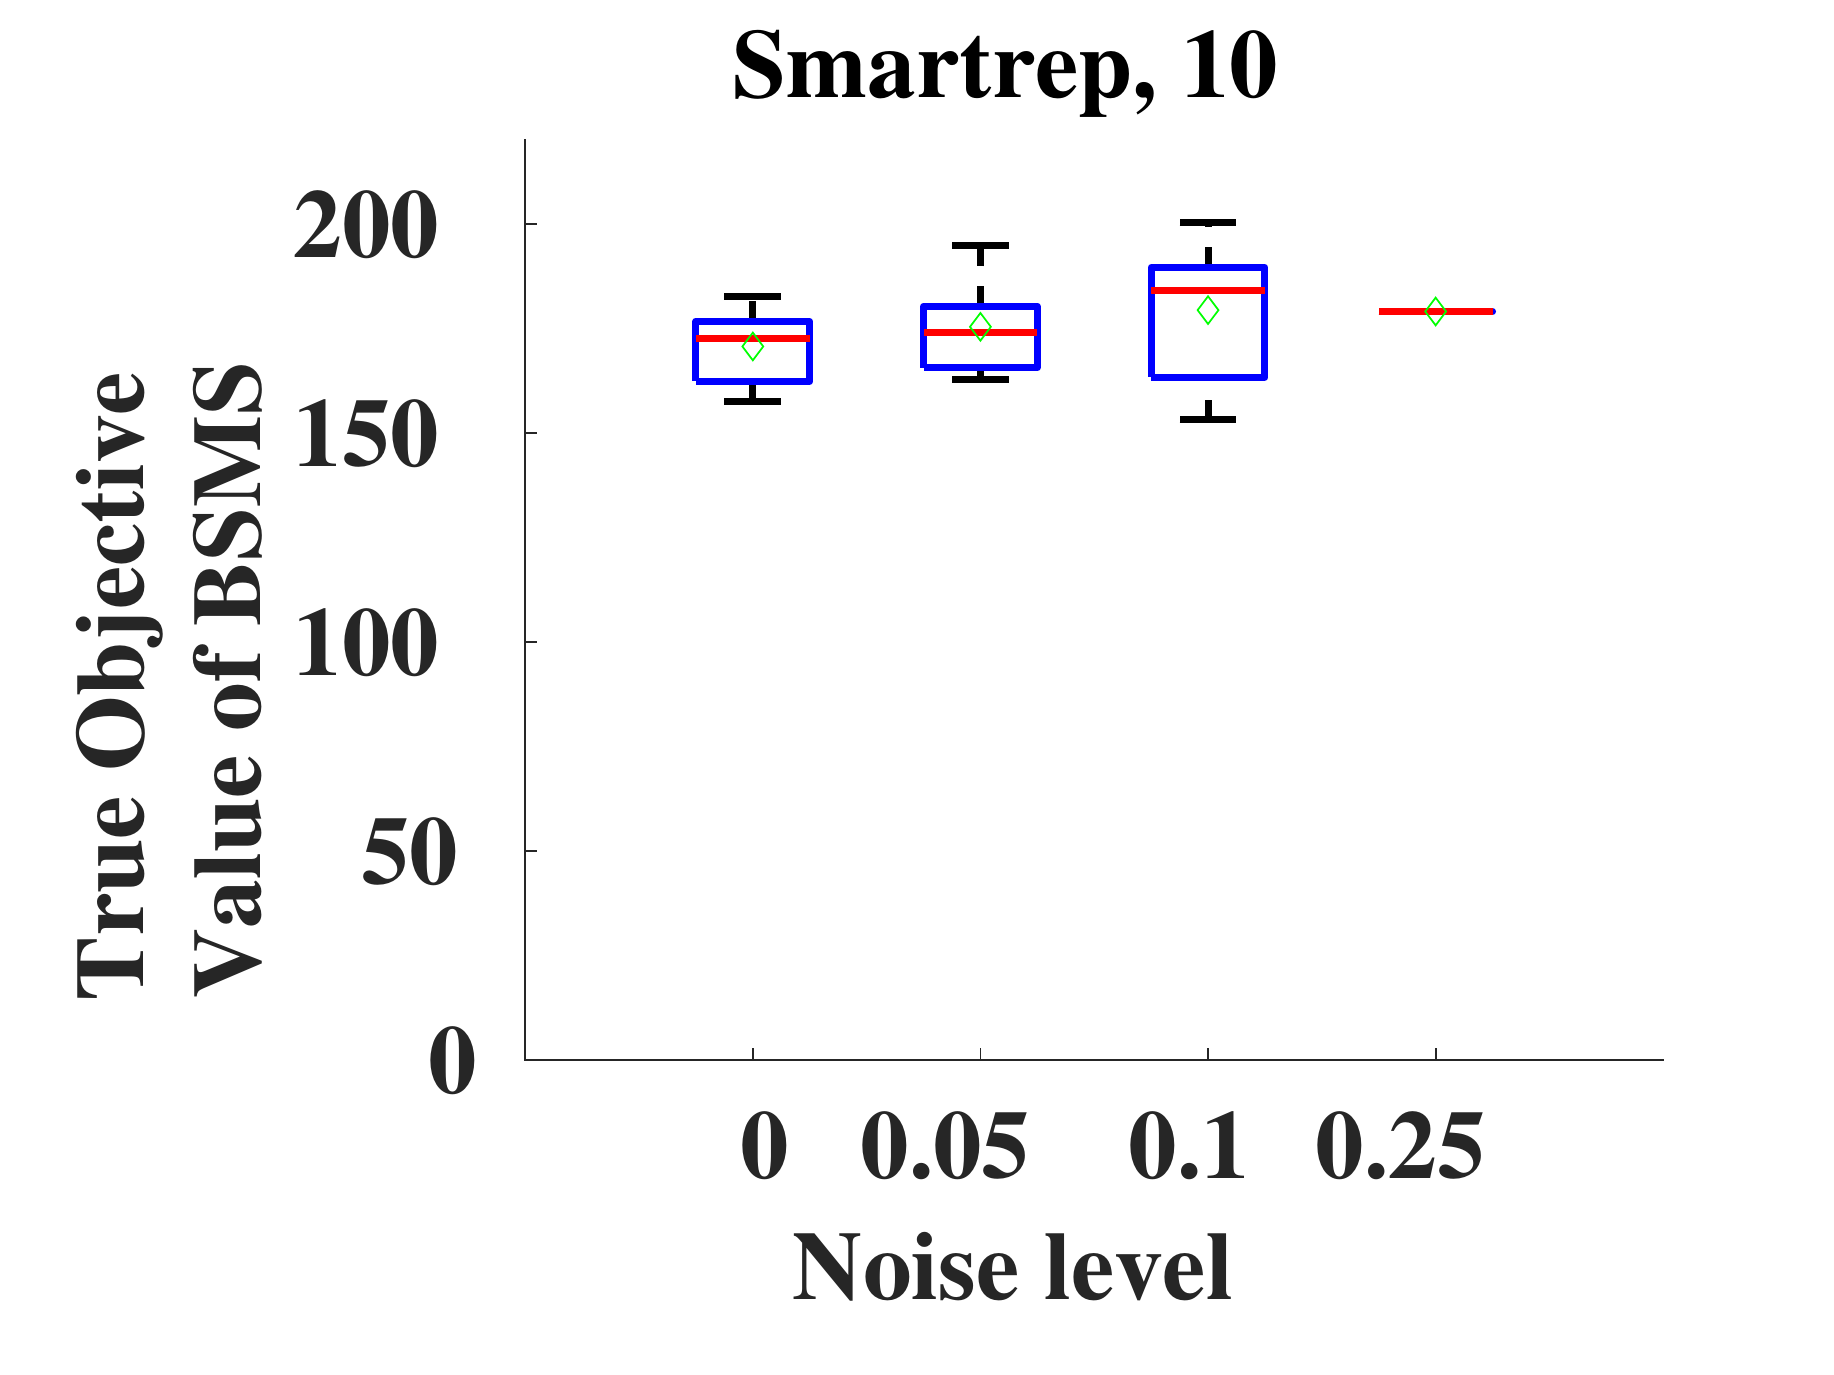}}
    \end{minipage}
    \caption{Box-plots of the true objective value of the BSMS after 1000 black-box function evaluations of surrogate optimization using RBF on the Rastrigin function}
    \label{fig:rbf_bks_box_rast}
    \vspace{-5mm}
\end{figure}

\begin{figure}[!htp]
\centering
    \begin{minipage}{\linewidth}
        \subfloat[]{\includegraphics[width=0.35\textwidth]{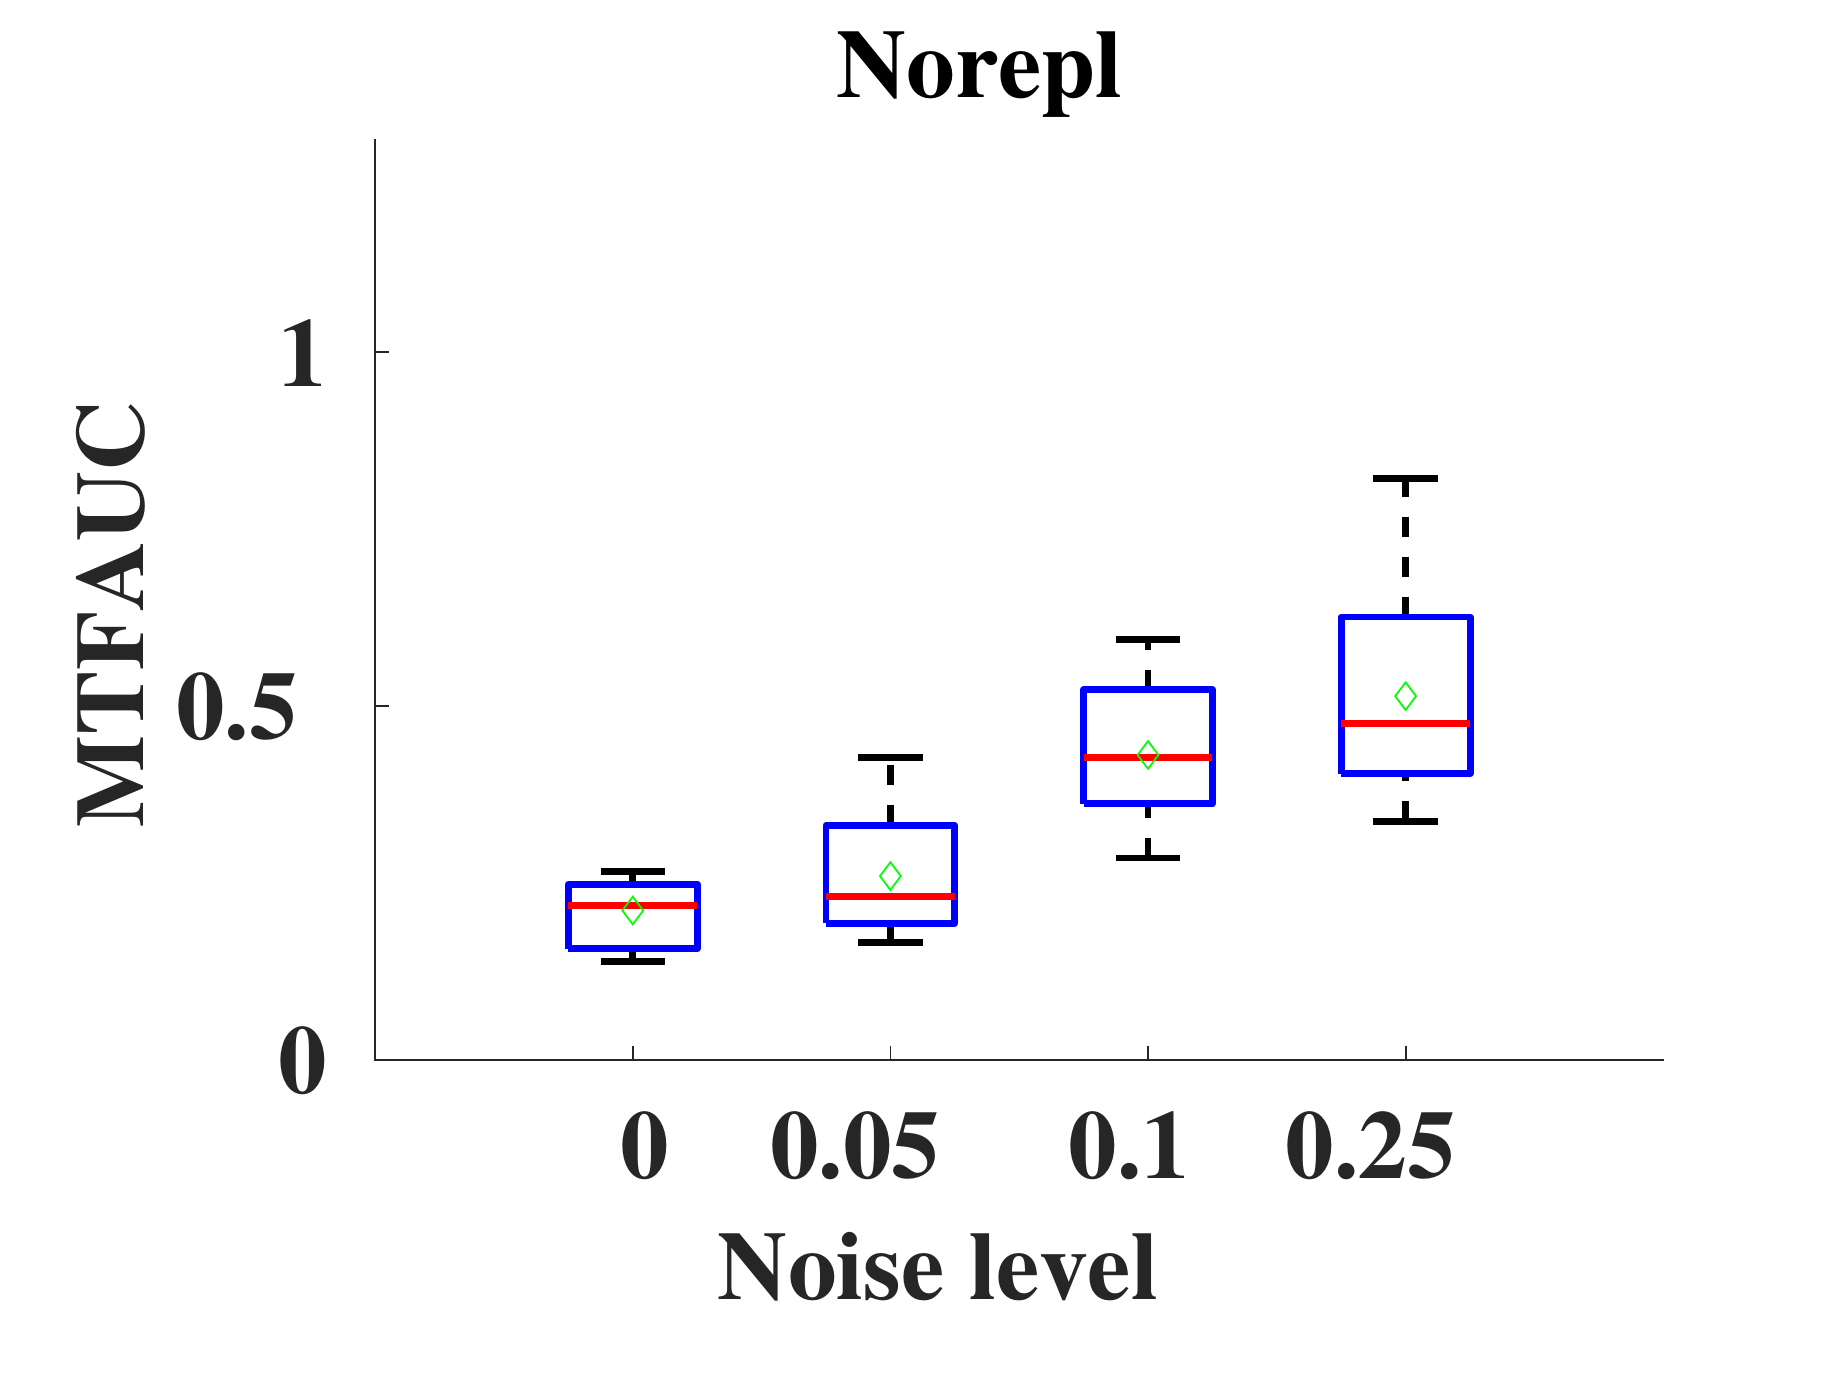}}
        \subfloat[]{\includegraphics[width=0.35\textwidth]{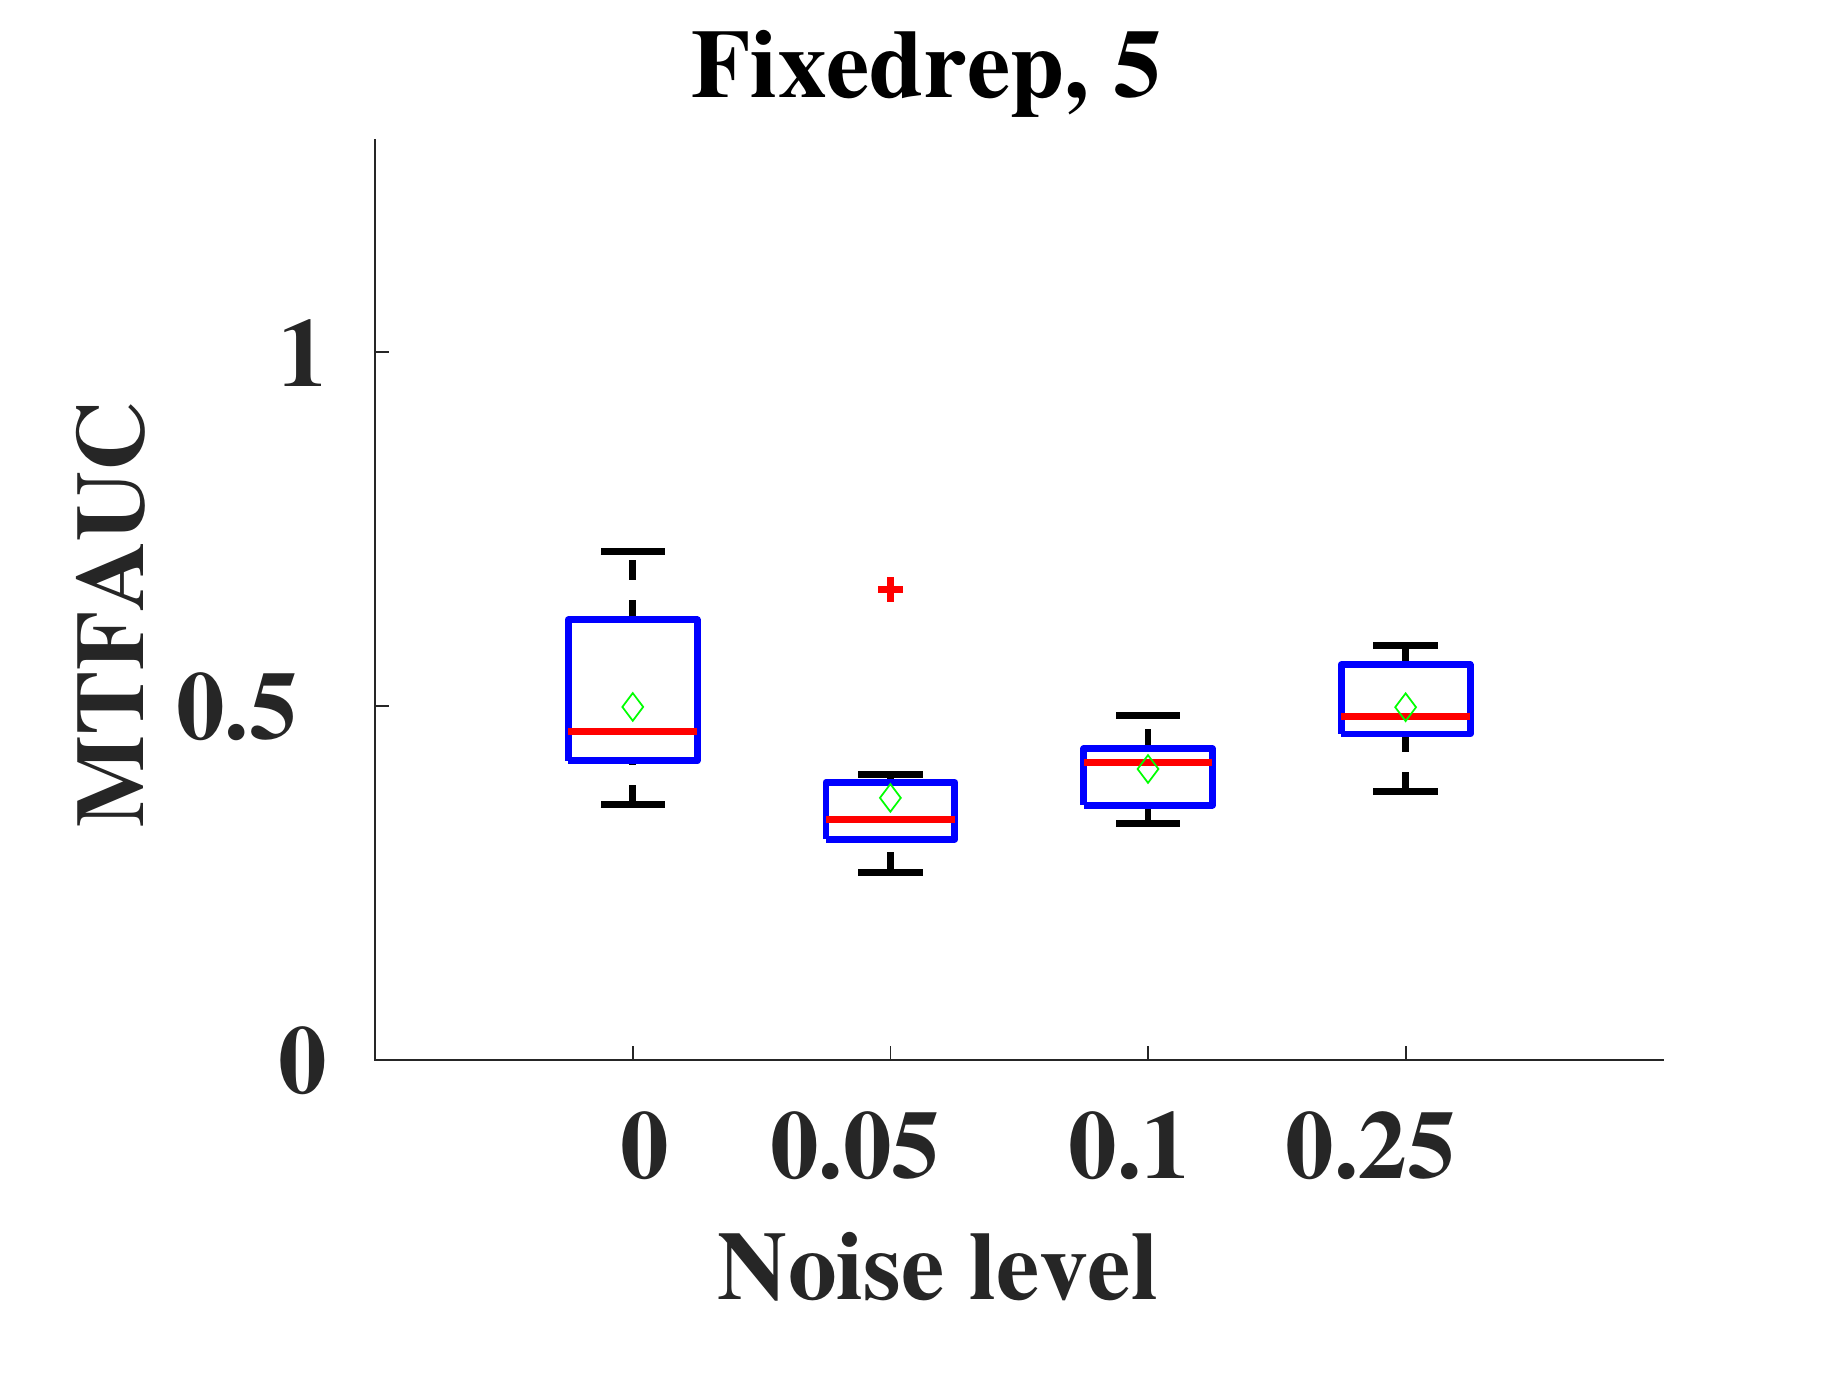}}
        \subfloat[]{\includegraphics[width=0.35\textwidth]{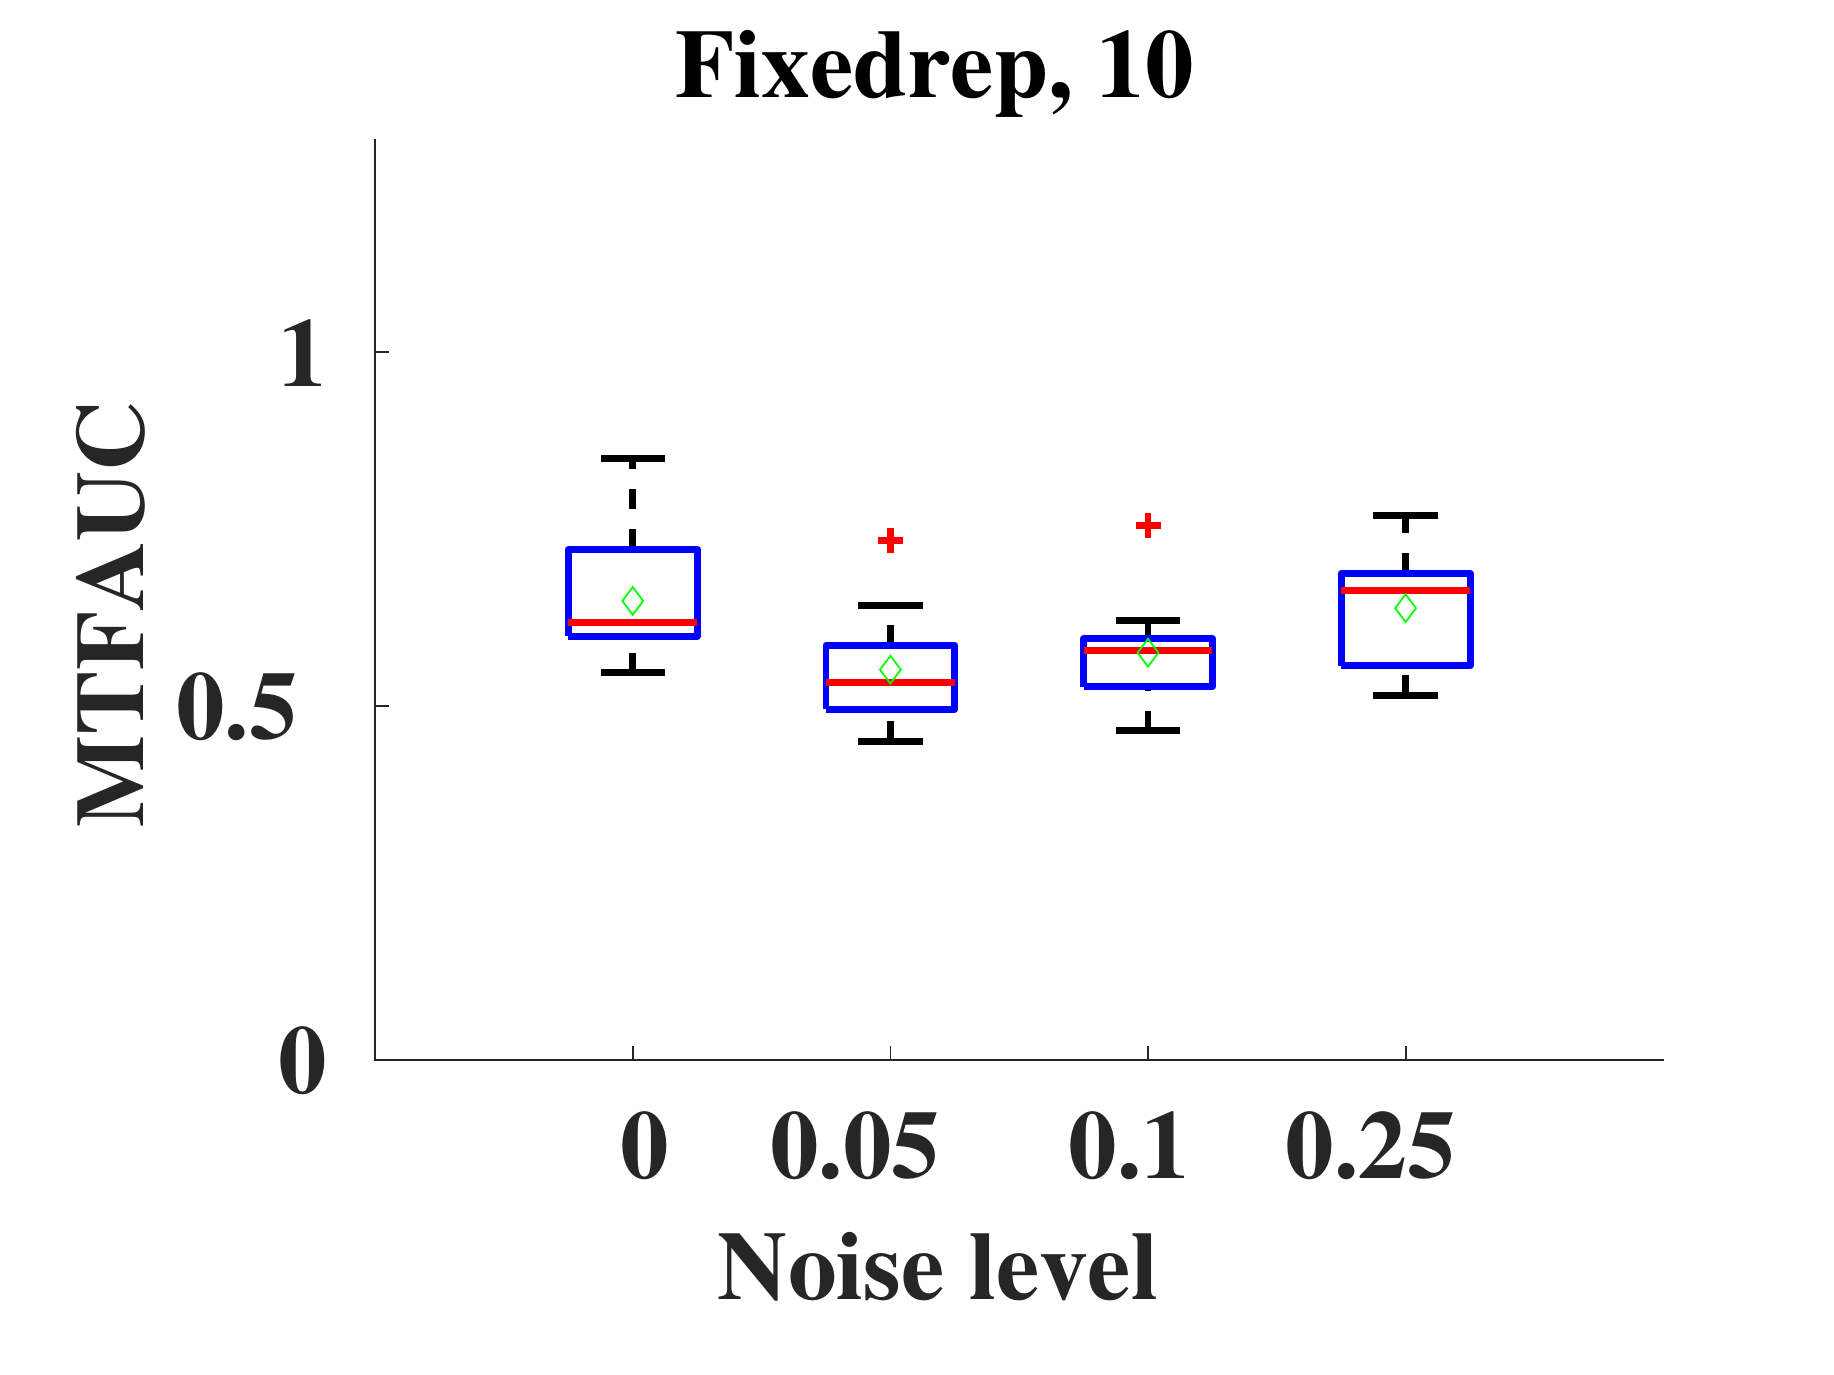}}
    \end{minipage}

    \begin{minipage}{\linewidth}
        \subfloat[]{\includegraphics[width=0.35\textwidth]{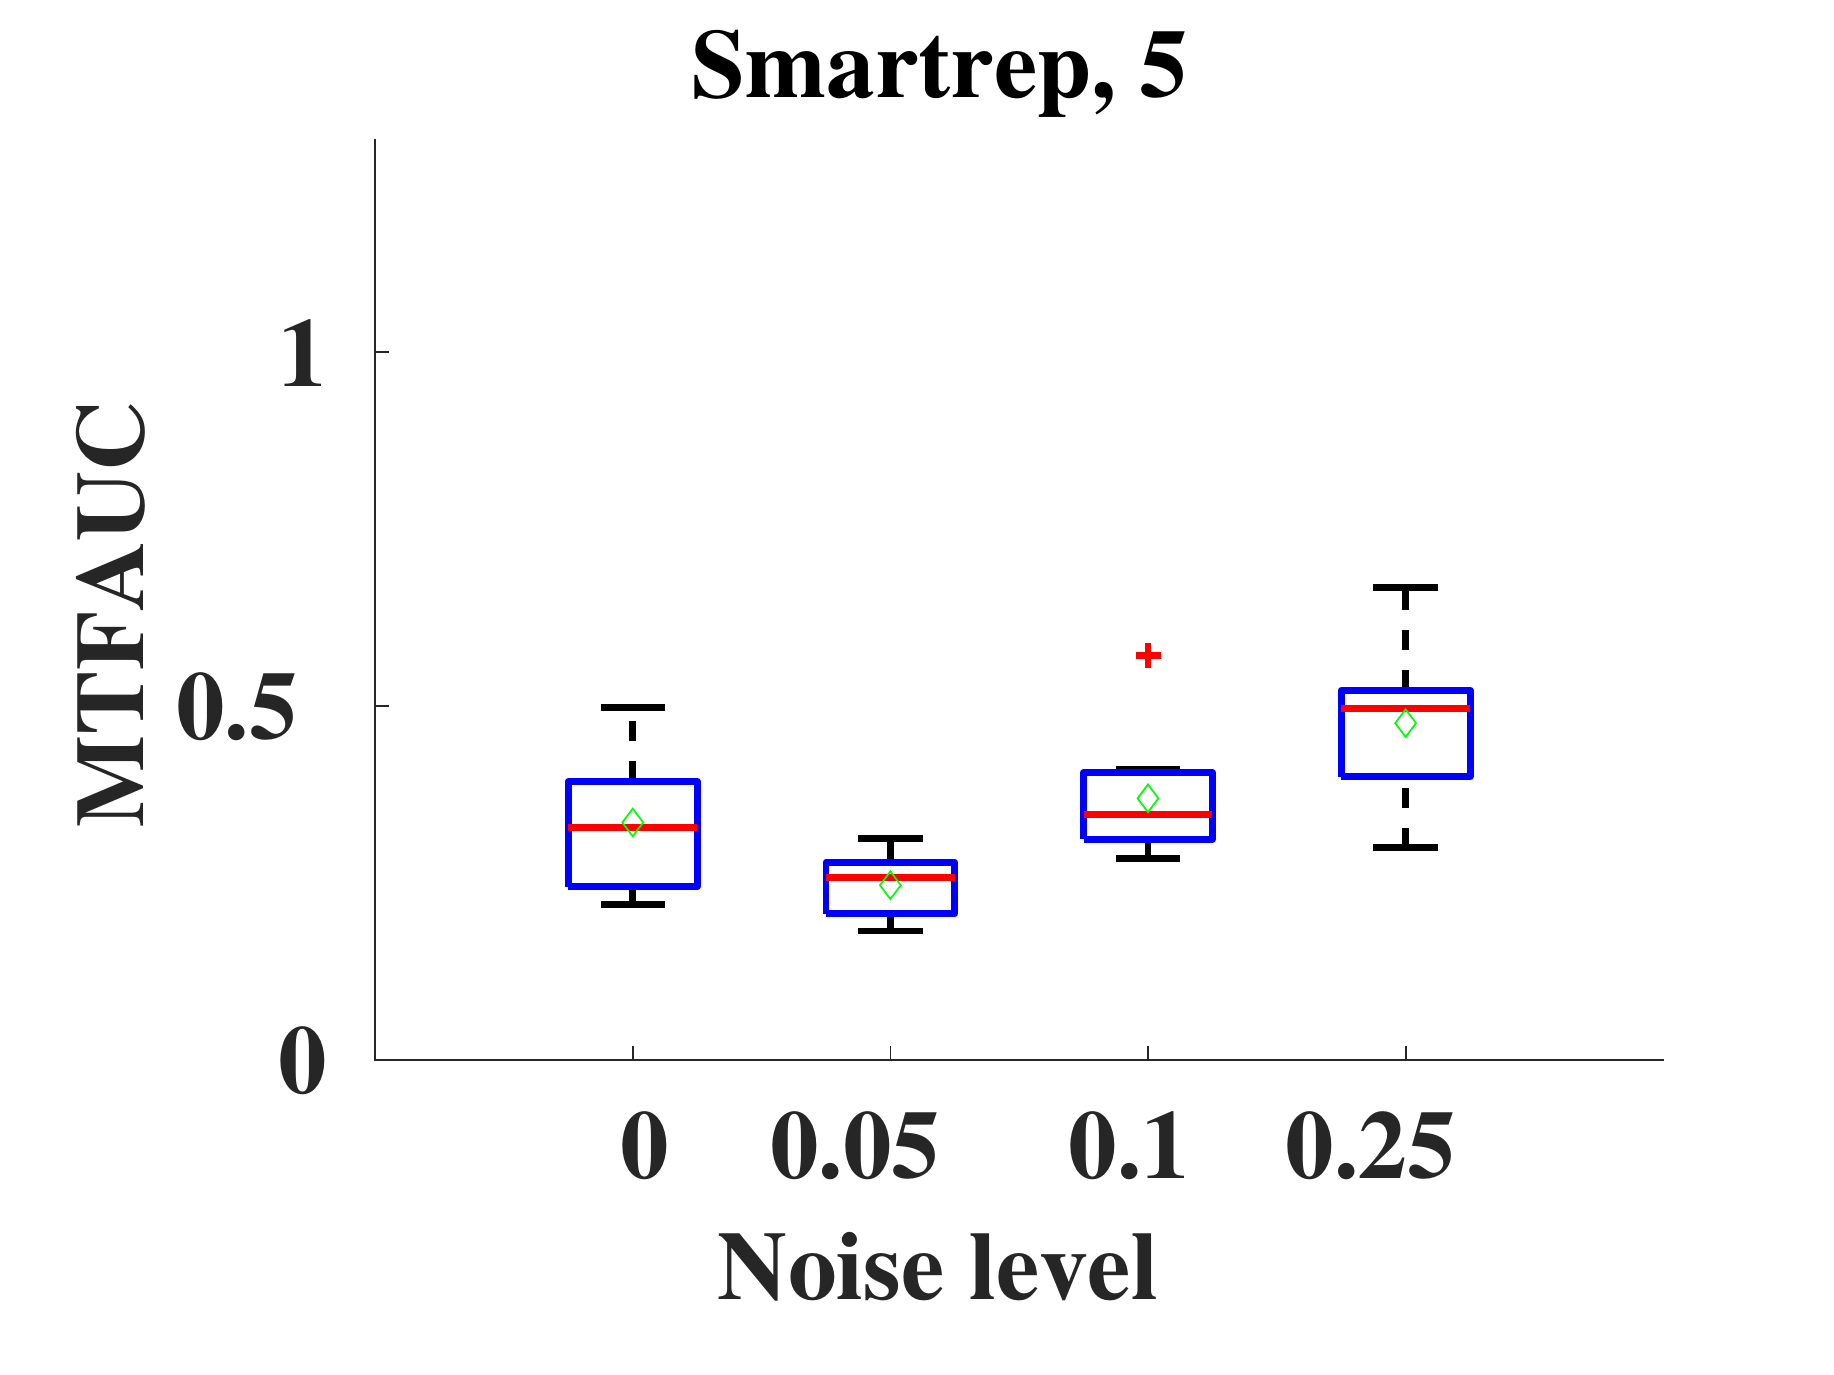}}
        \subfloat[]{\includegraphics[width=0.35\textwidth]{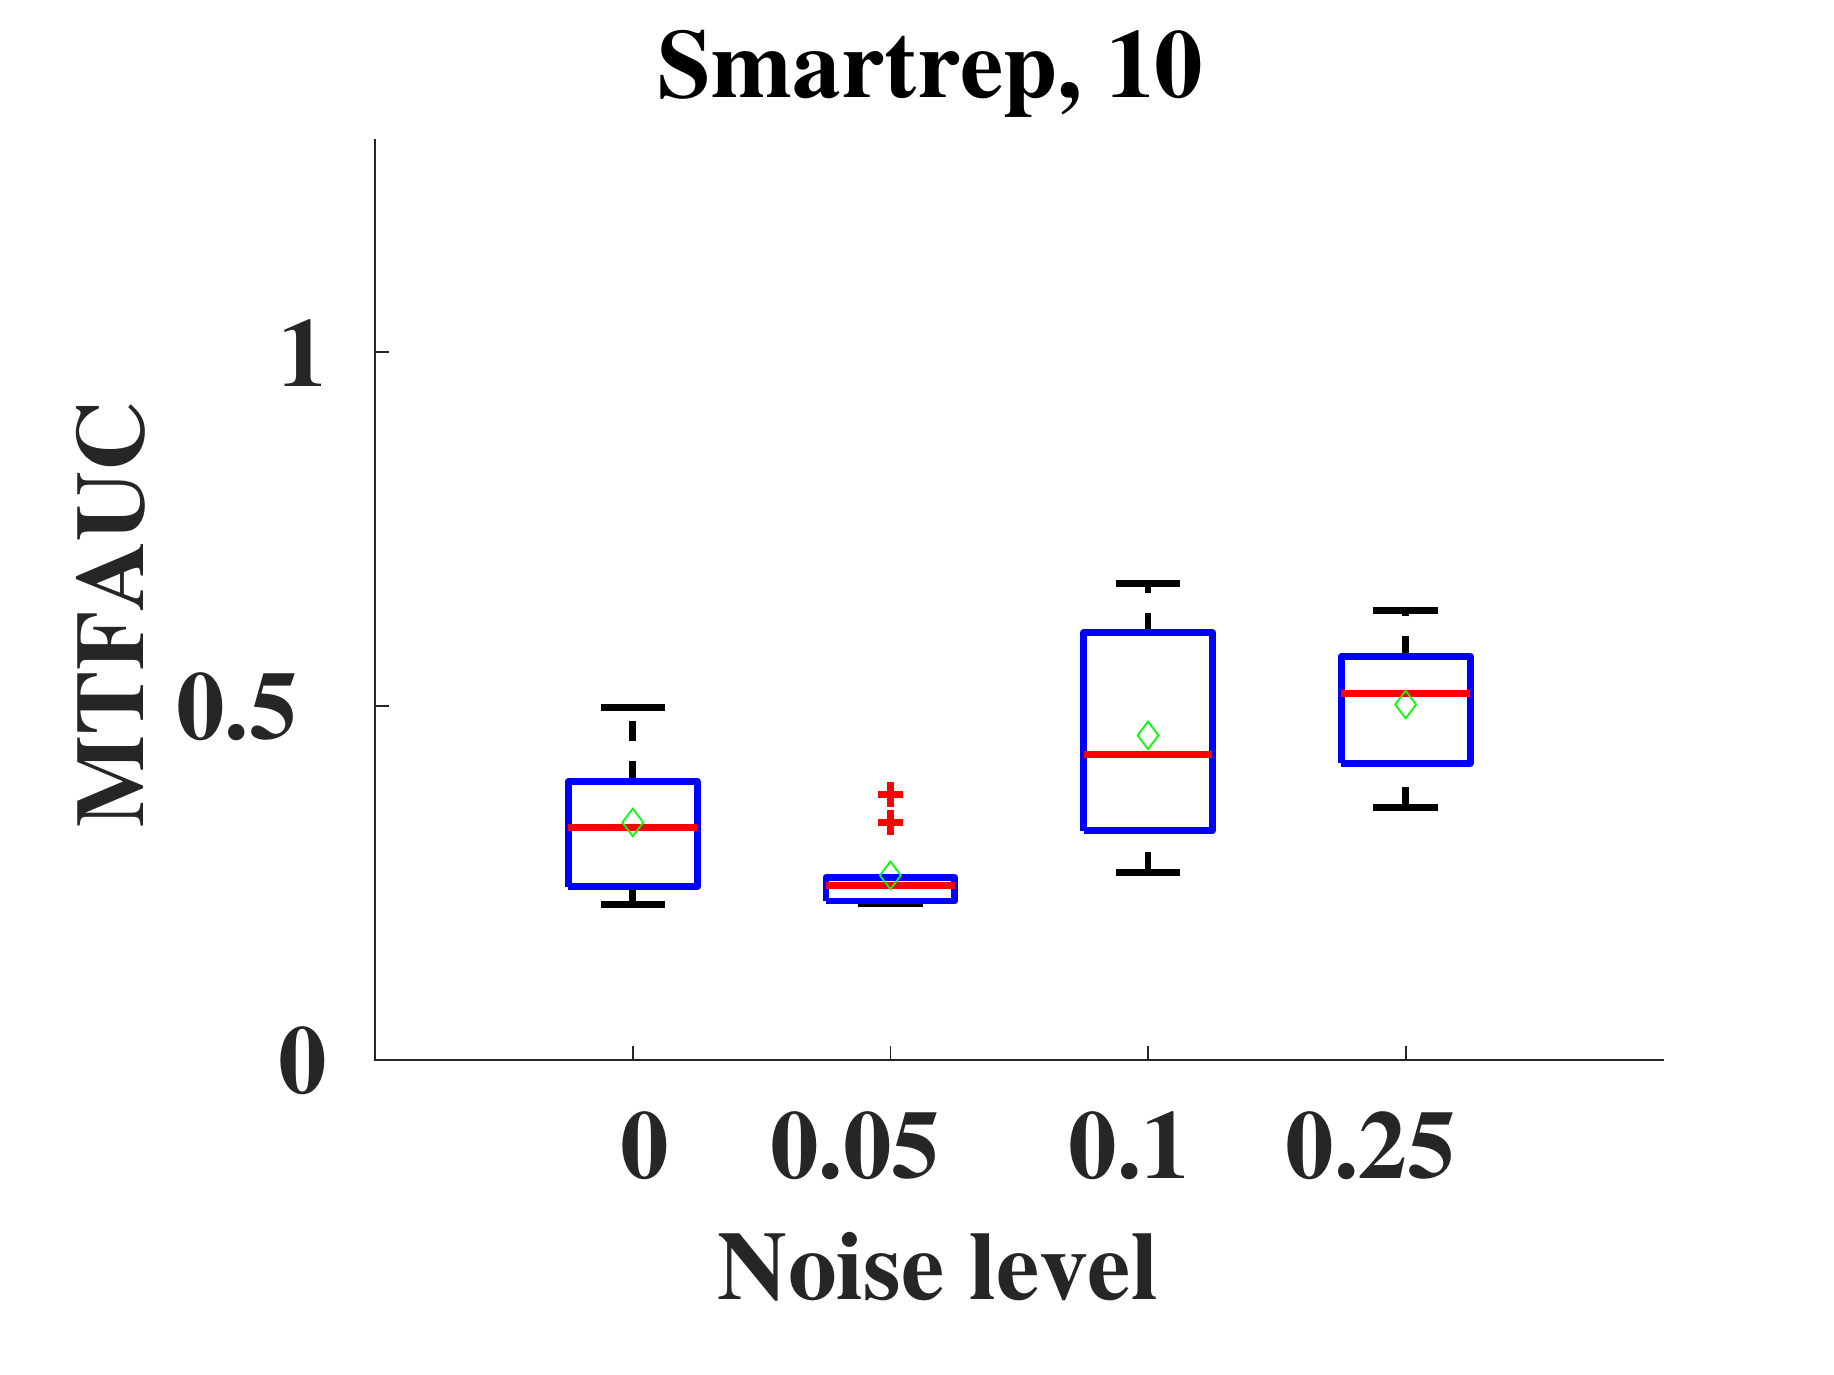}}
    \end{minipage}
    \caption{Box-plots of MTFAUC of surrogate optimization using RBF on the Levy function}
    \label{fig:rbf_auc_box_levy}
    \vspace{-5mm}
\end{figure}
\begin{figure}[!htp]
\centering
    \begin{minipage}{\linewidth}
        \subfloat[]{\includegraphics[width=0.35\textwidth]{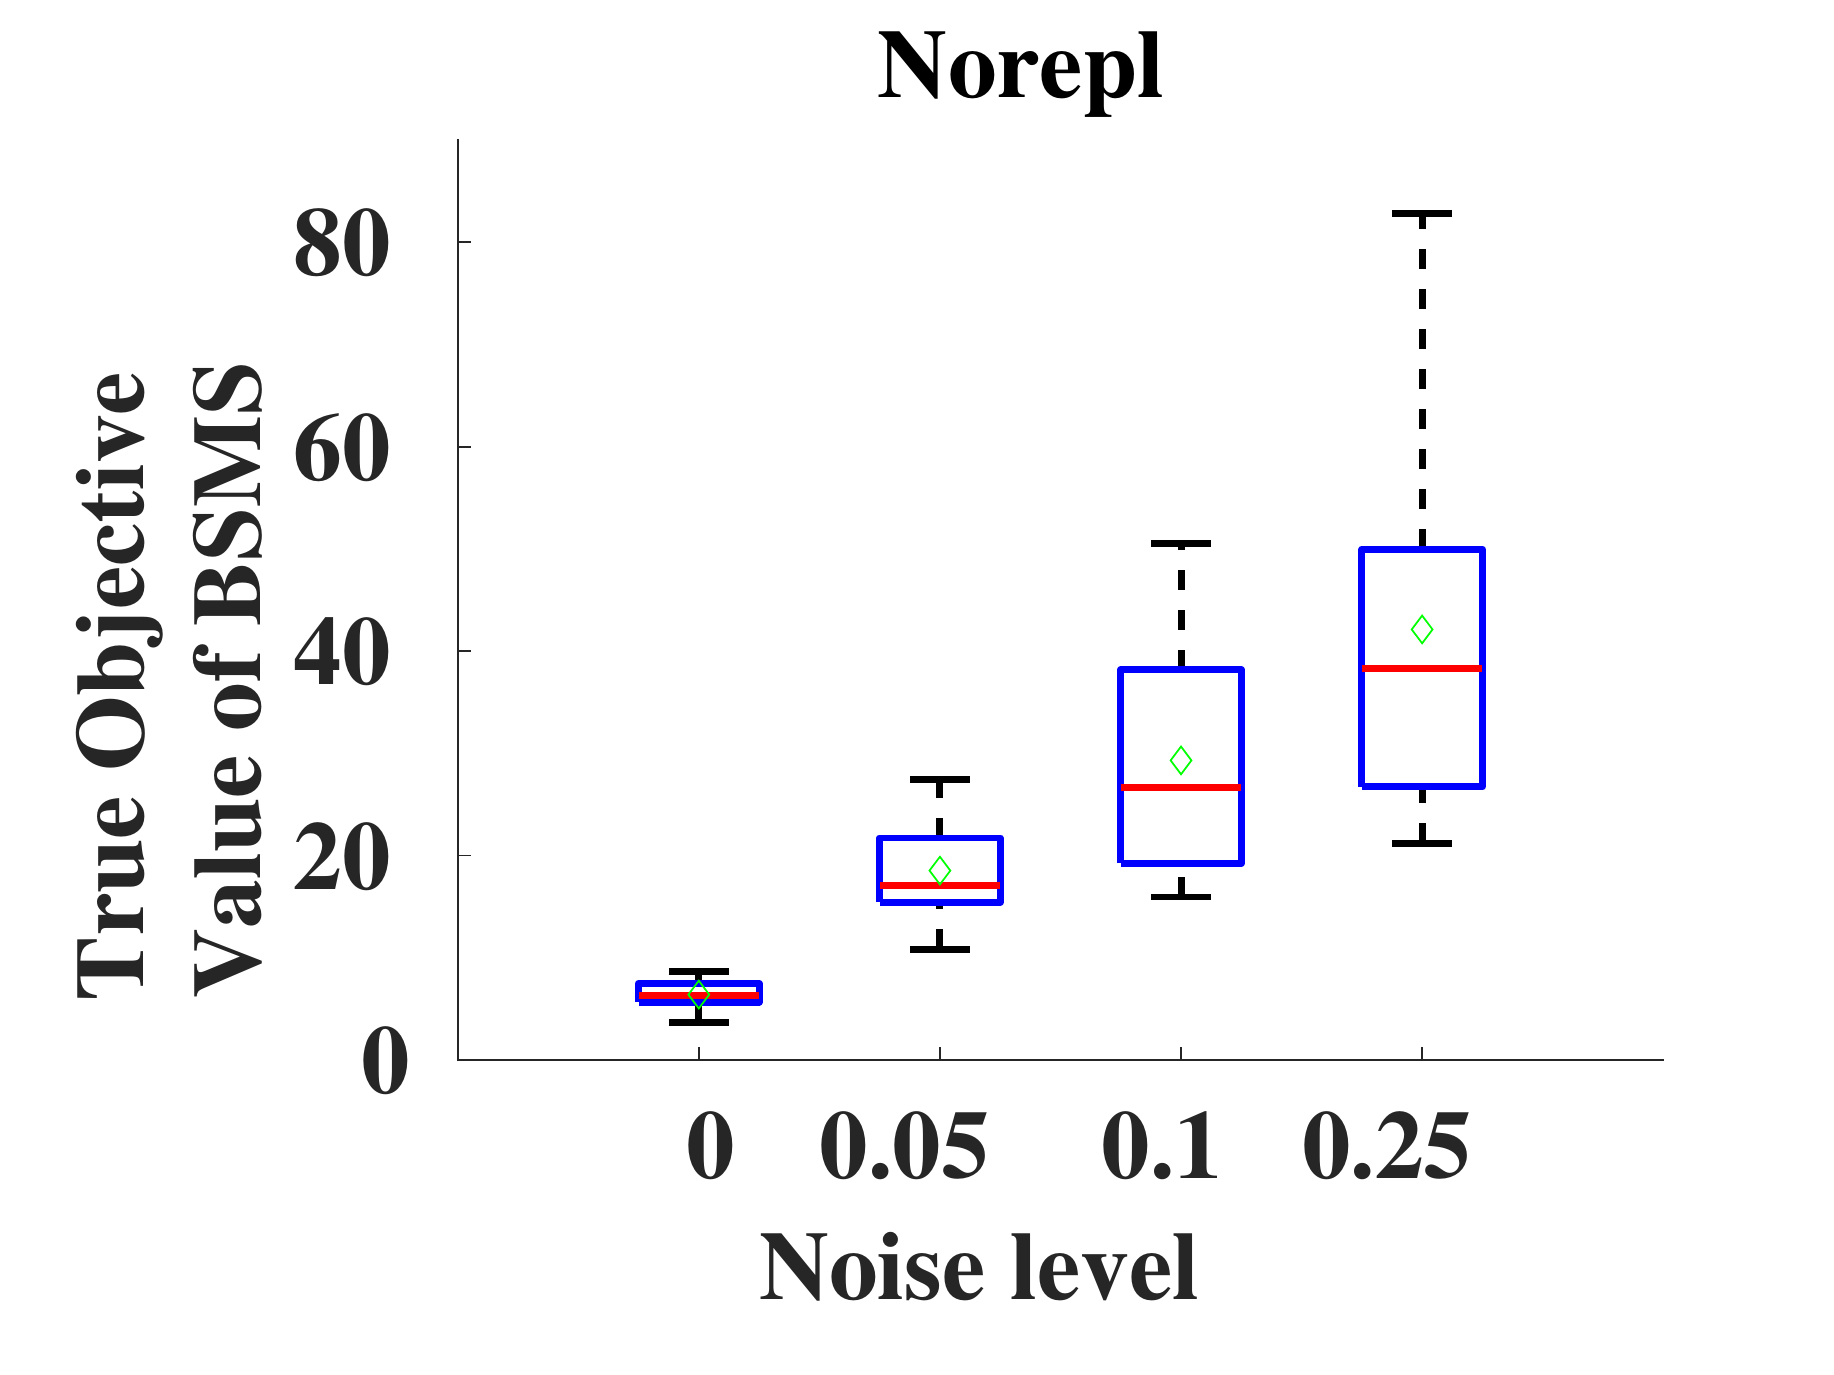}}
        \subfloat[]{\includegraphics[width=0.35\textwidth]{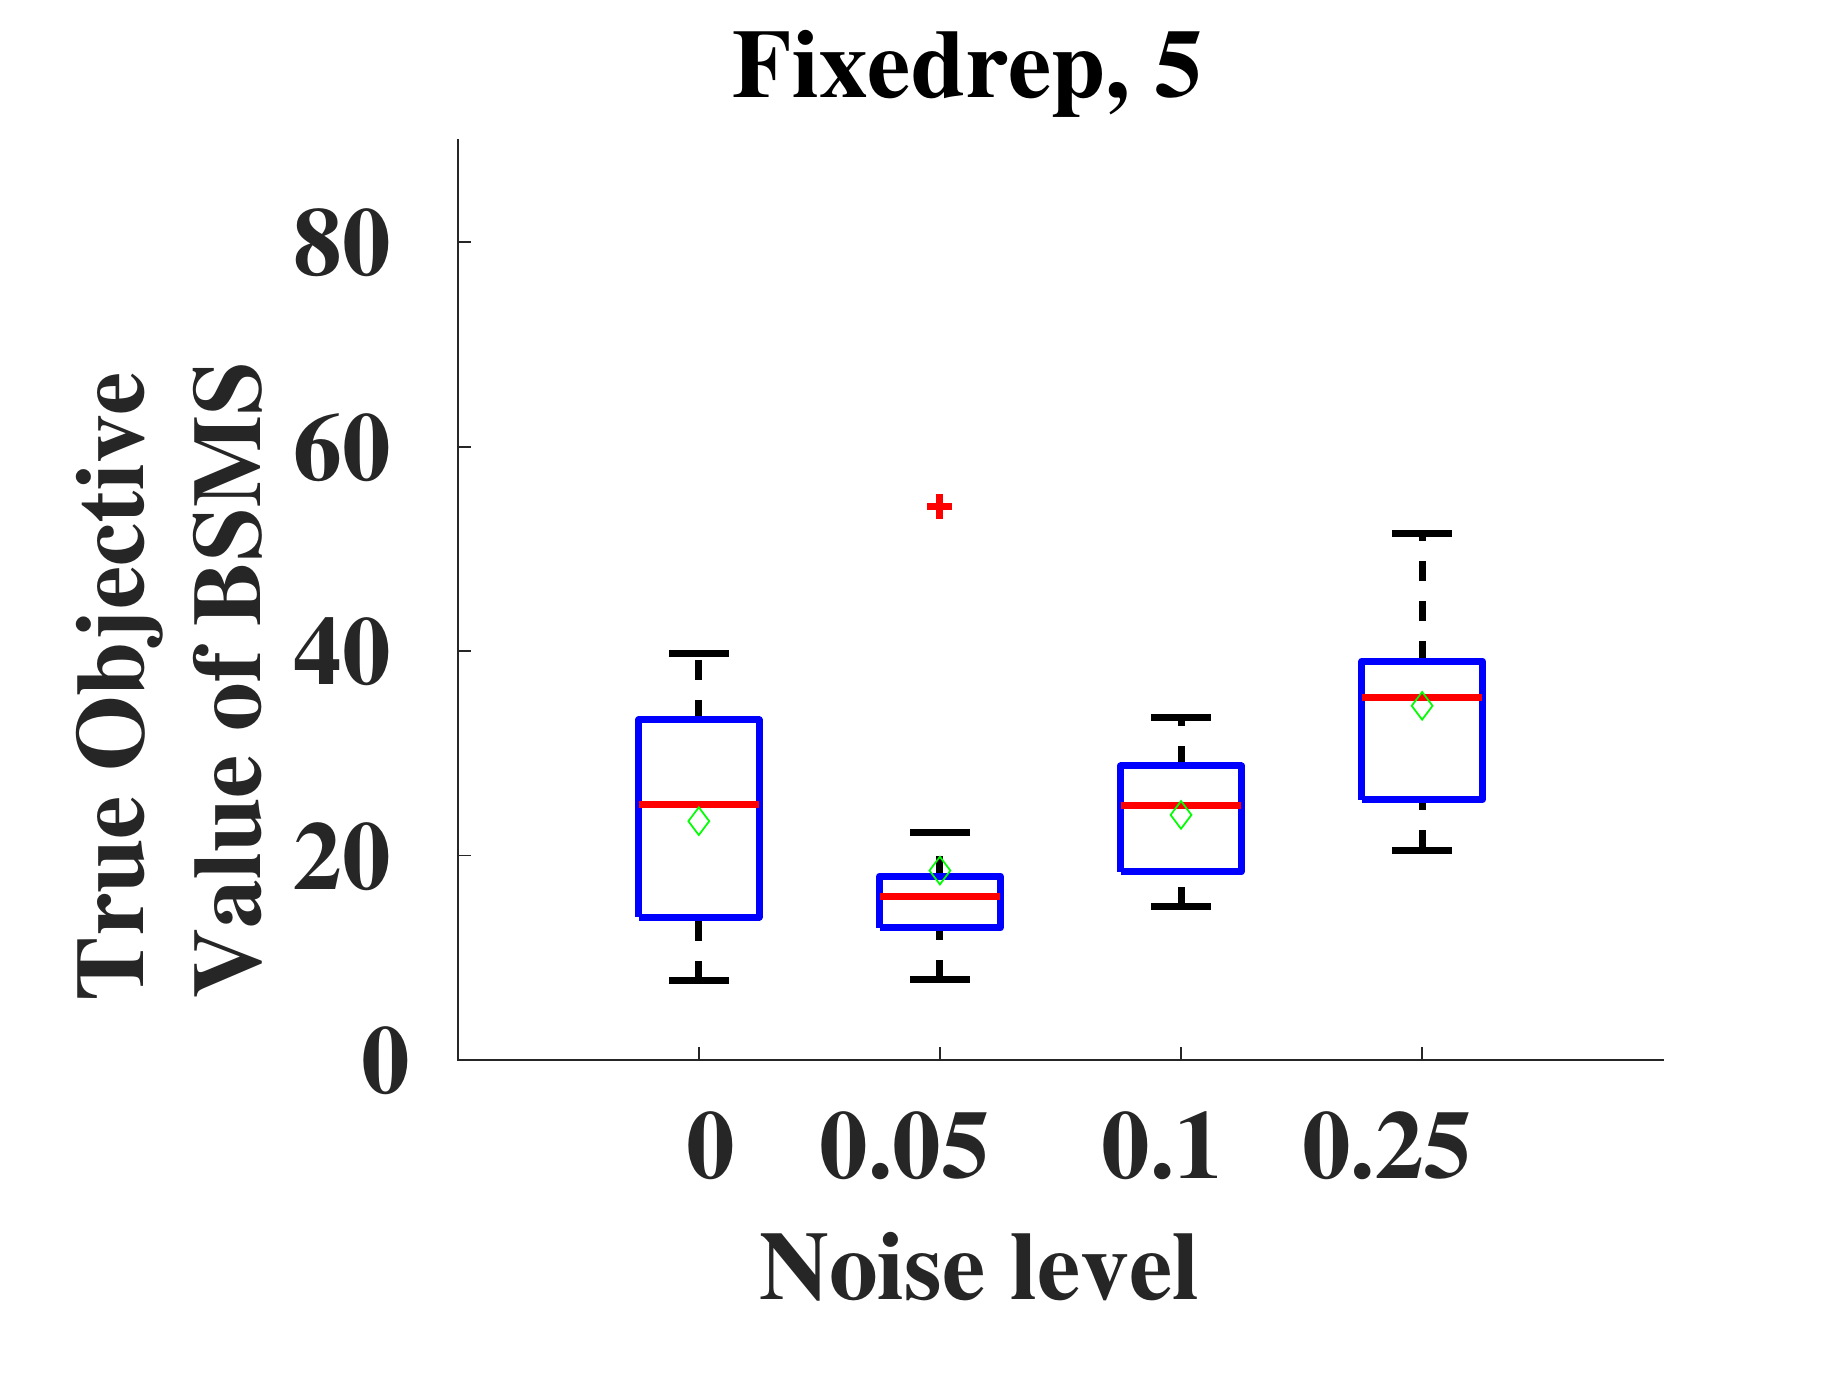}}
        \subfloat[]{\includegraphics[width=0.35\textwidth]{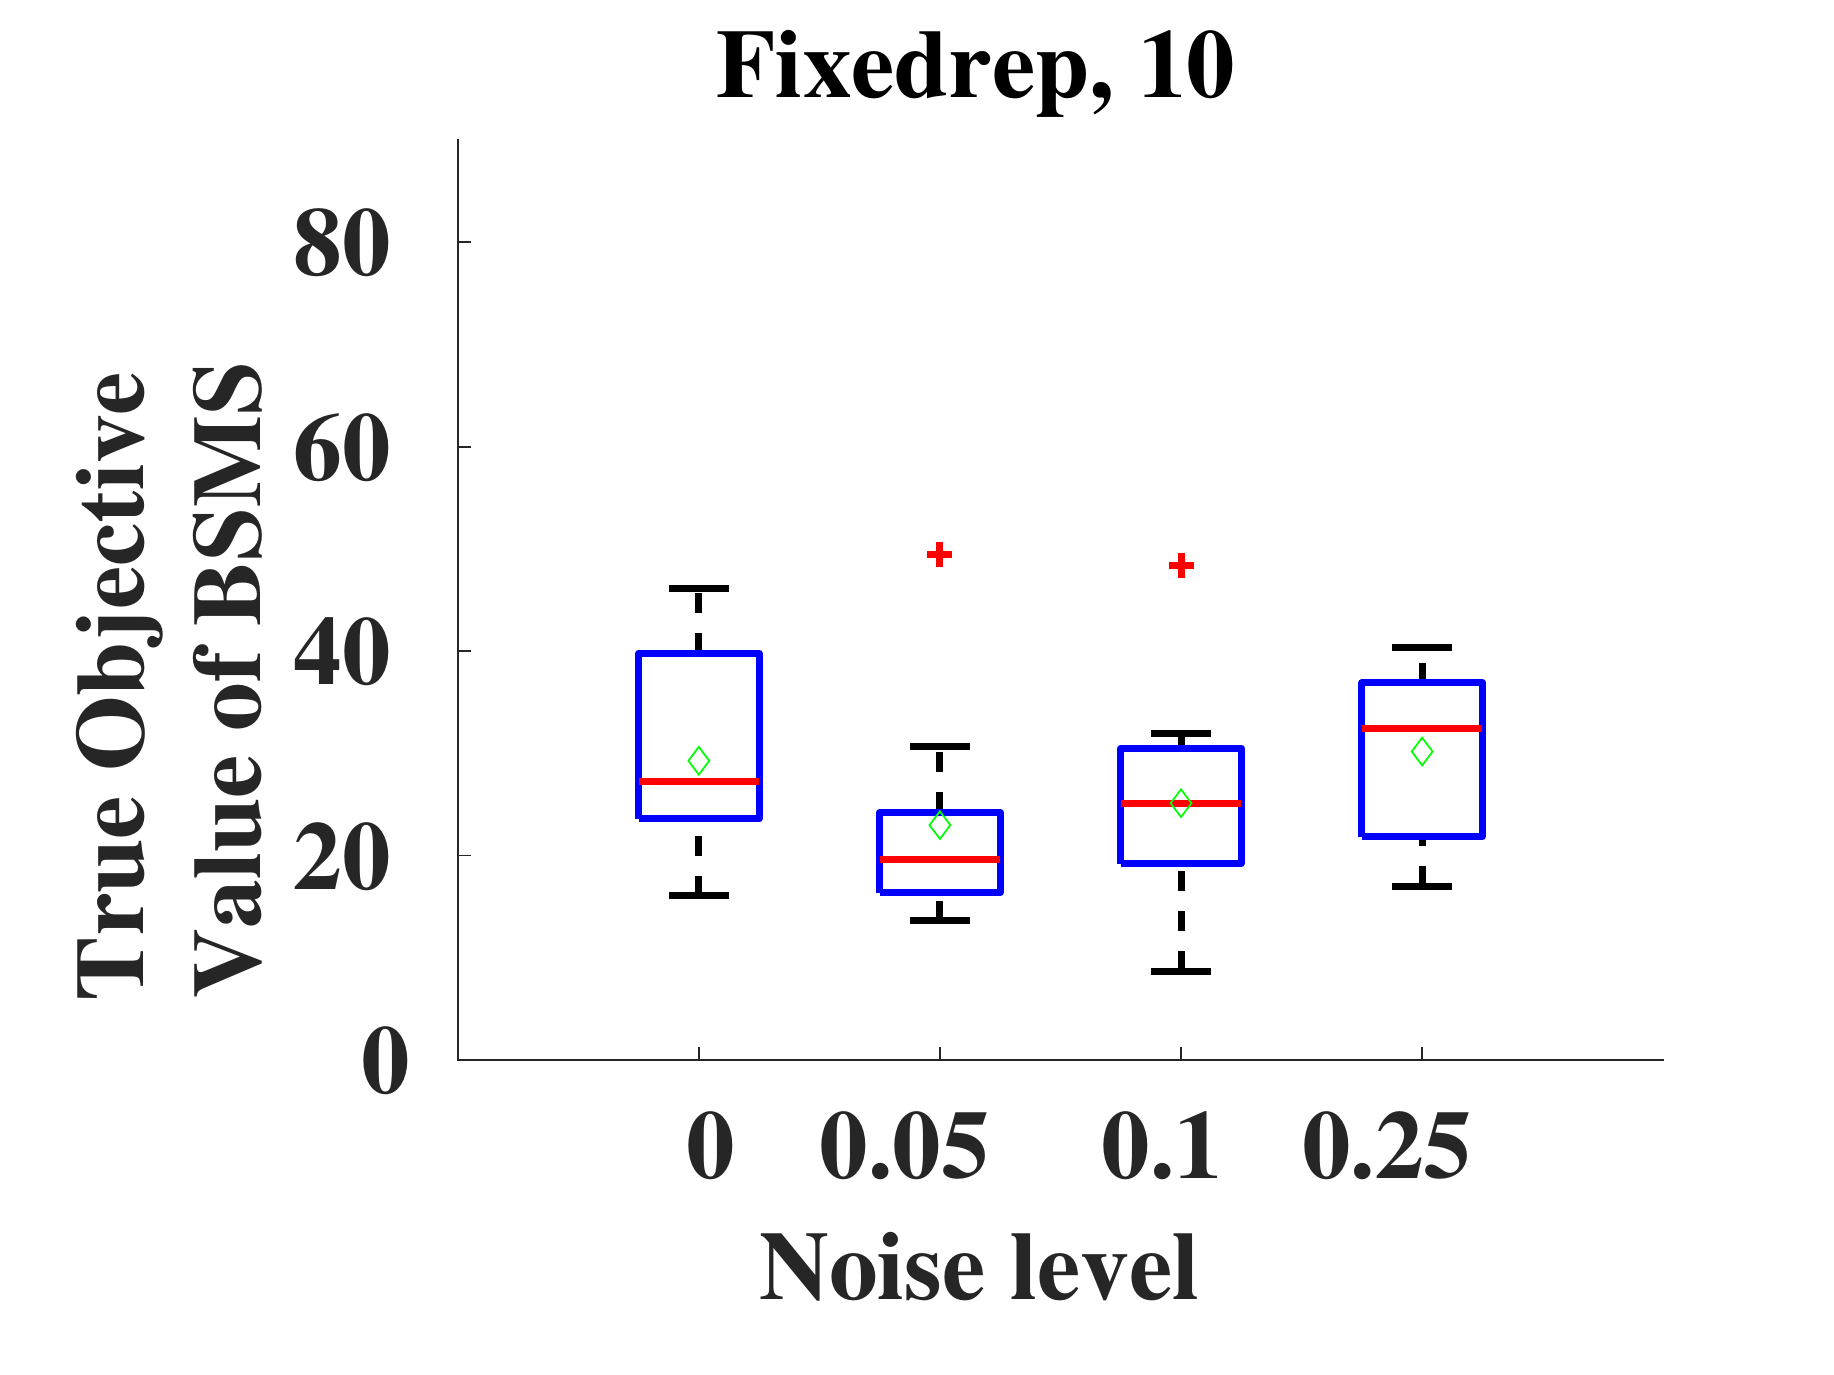}}
    \end{minipage}

    \begin{minipage}{\linewidth}
        \subfloat[]{\includegraphics[width=0.35\textwidth]{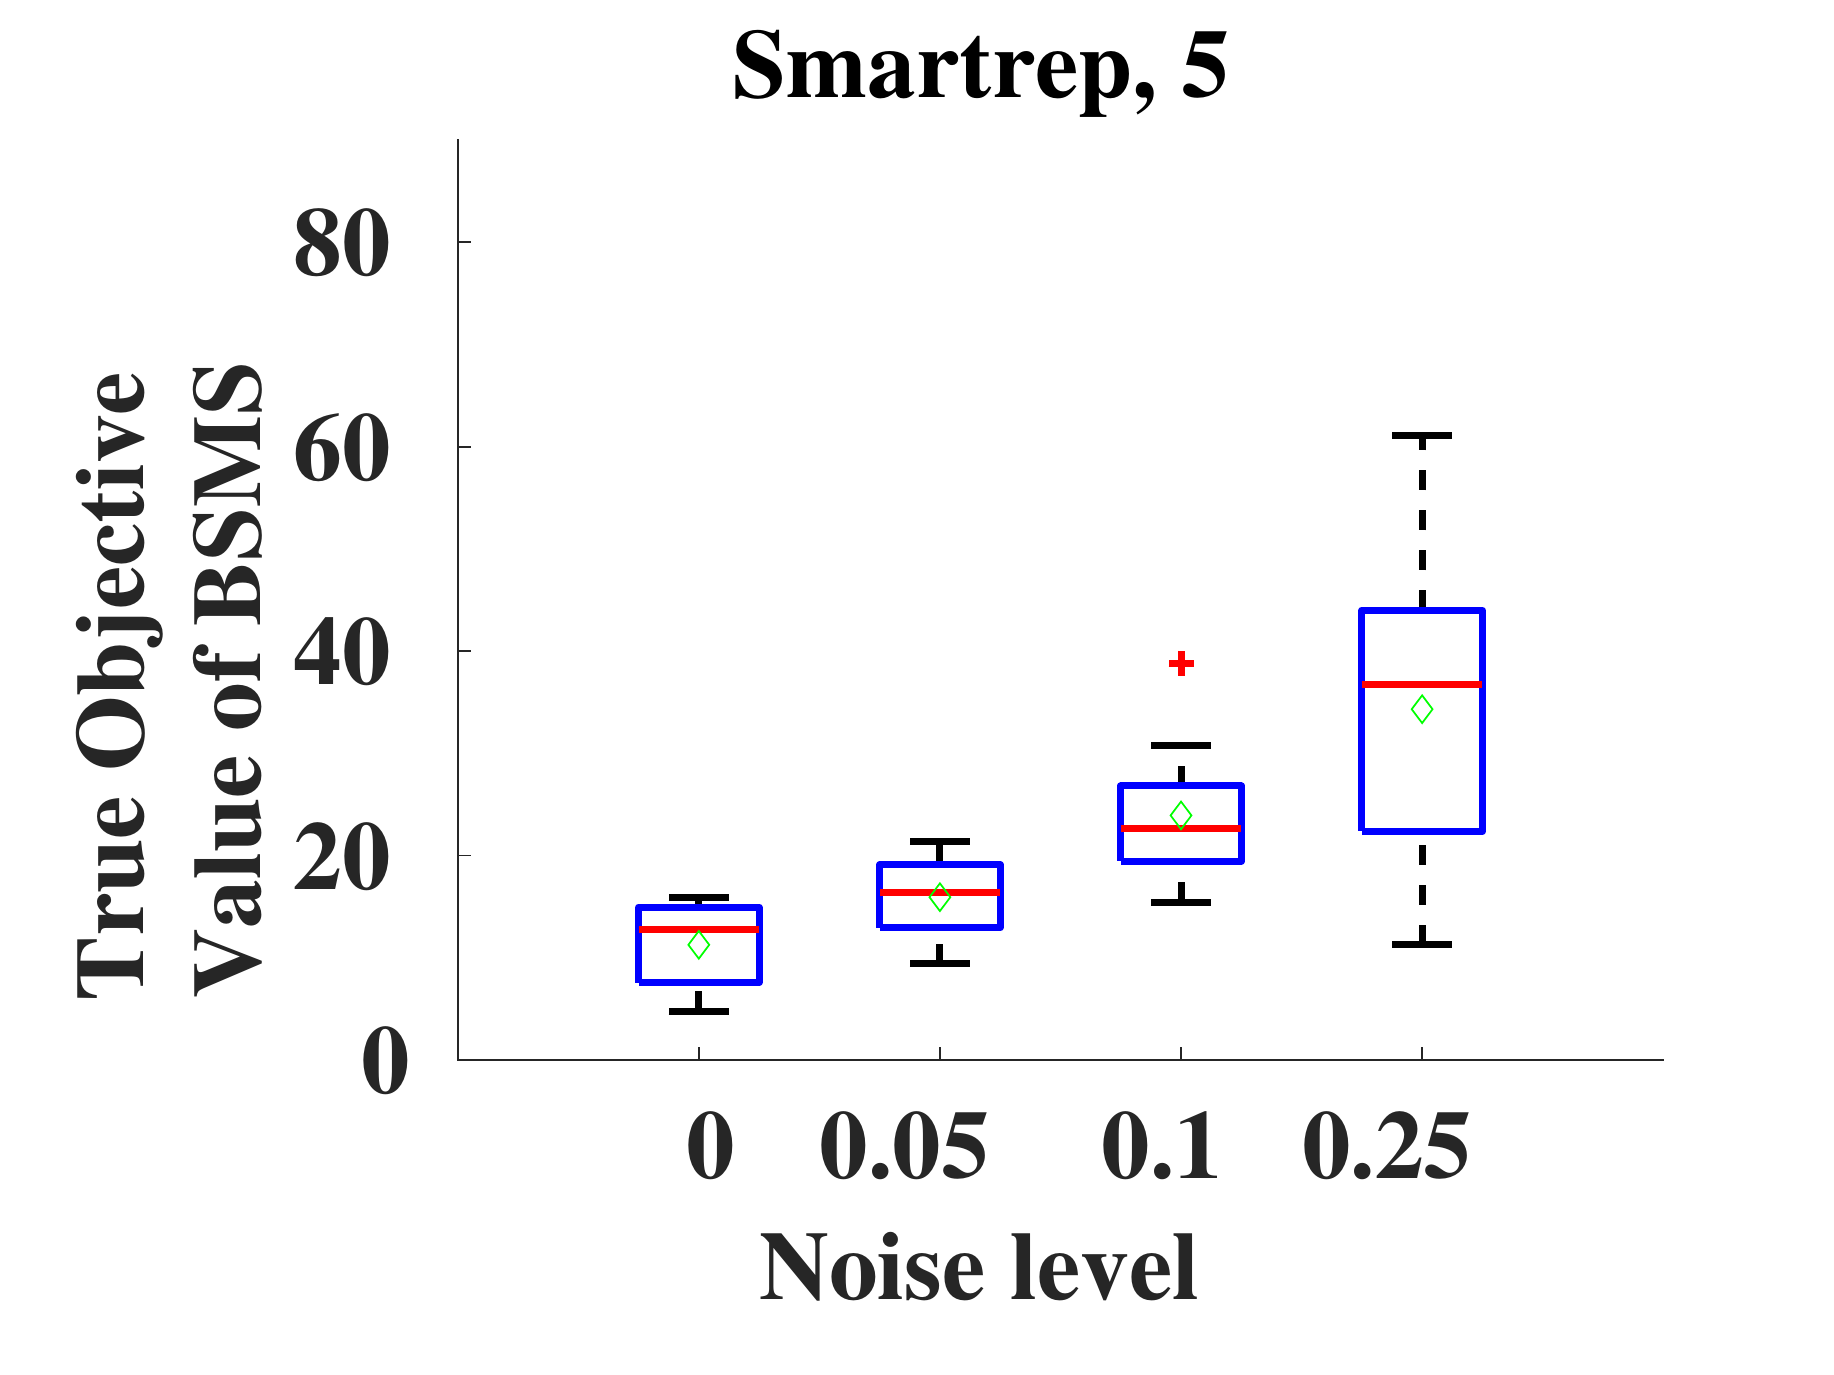}}
        \subfloat[]{\includegraphics[width=0.35\textwidth]{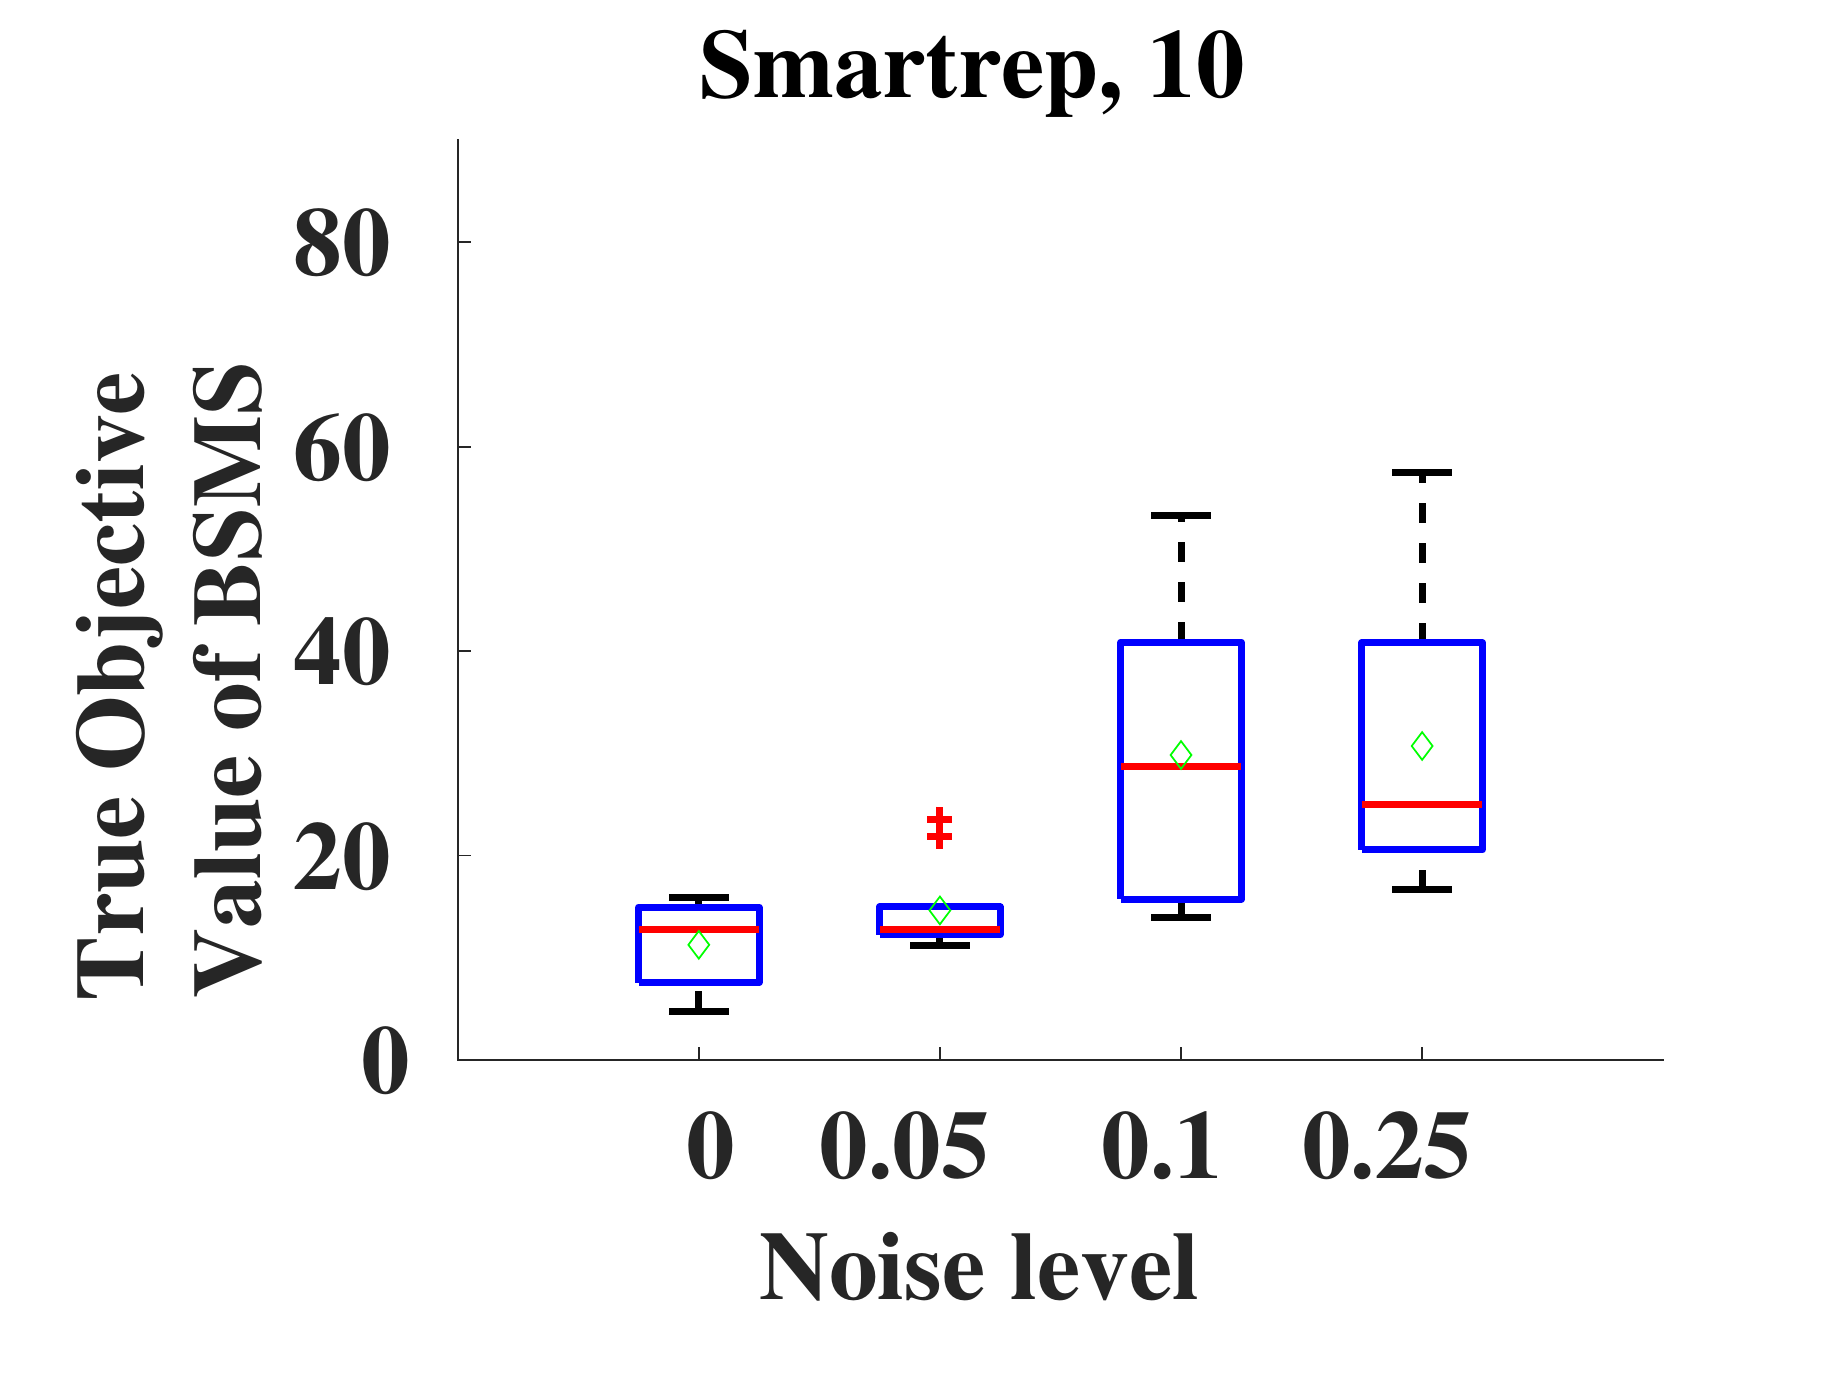}}
    \end{minipage}
    \caption{Box-plots of the true objective value of the BSMS after 1000 black-box function evaluations of surrogate optimization using RBF on the Levy function}
    \label{fig:rbf_bks_box_levy}
    \vspace{-5mm}
\end{figure}
